# Supplementary material for: Bayesian Statistical Modeling in Action for Estimation and Forecasting in Low- and Middle-income Countries: The Case of the Family Planning Estimation Tool
Source: arXiv:2501.00007 source file (2025-12-09)

# Afghanistan − married

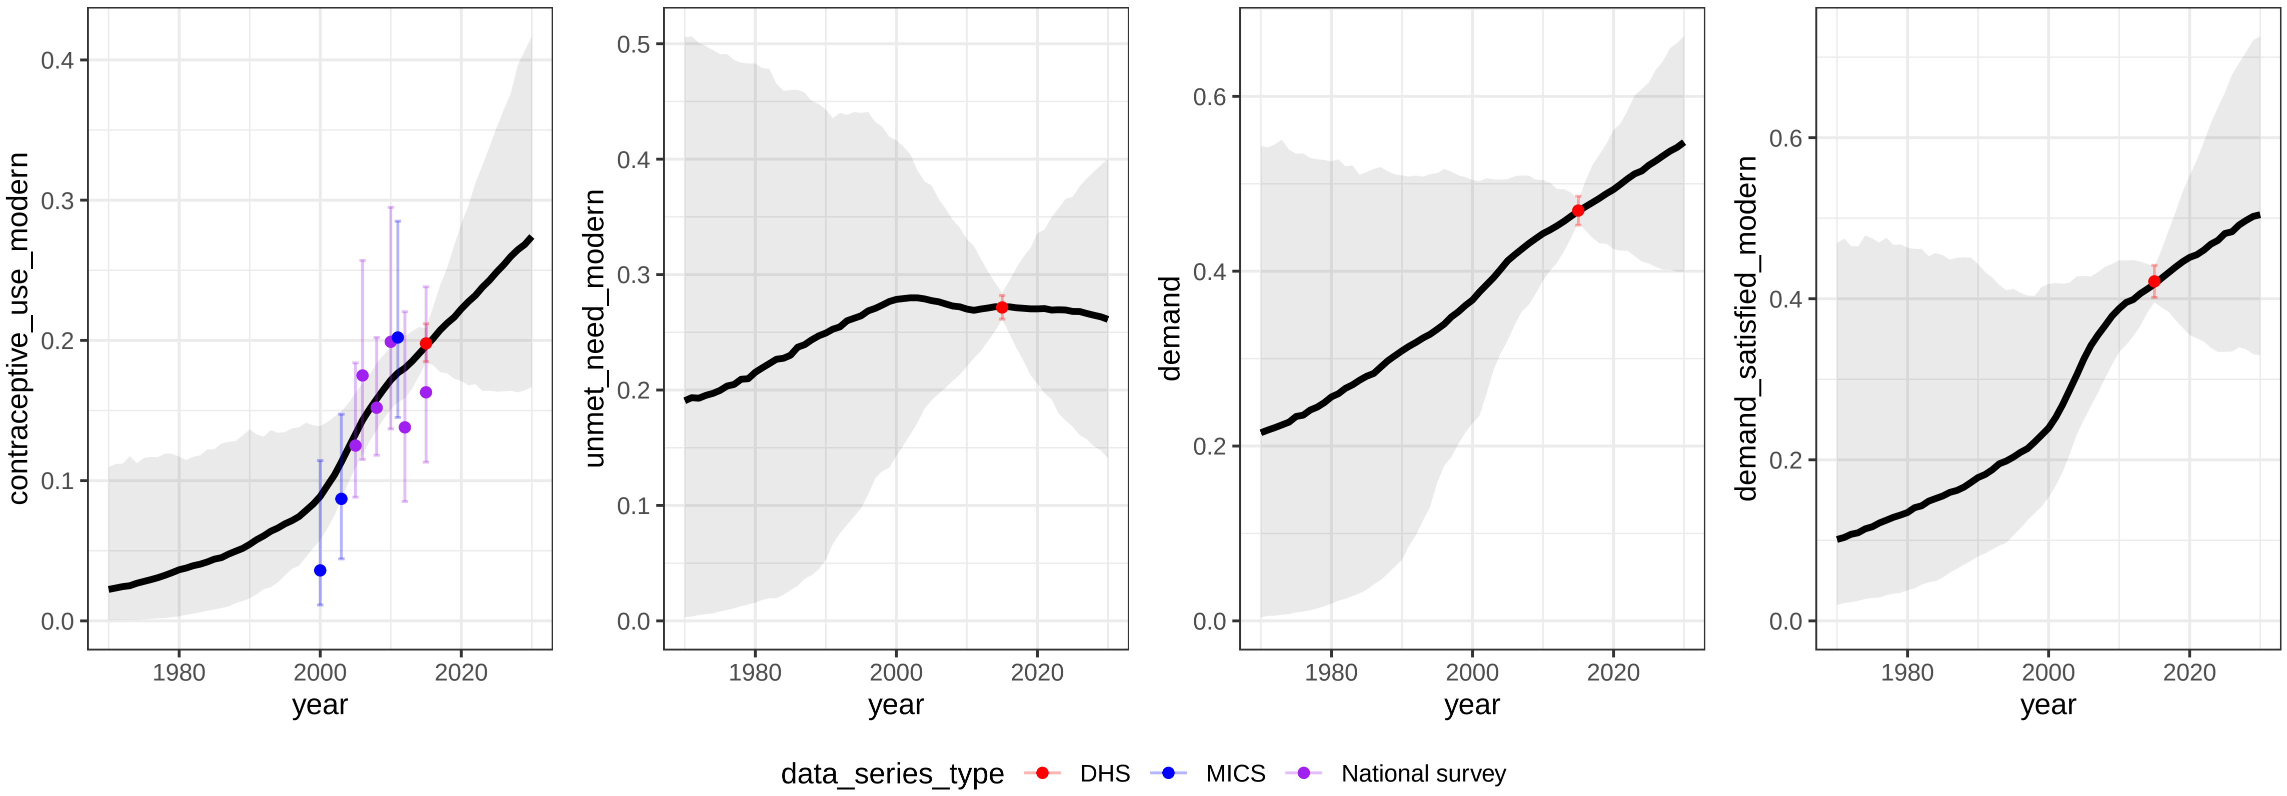

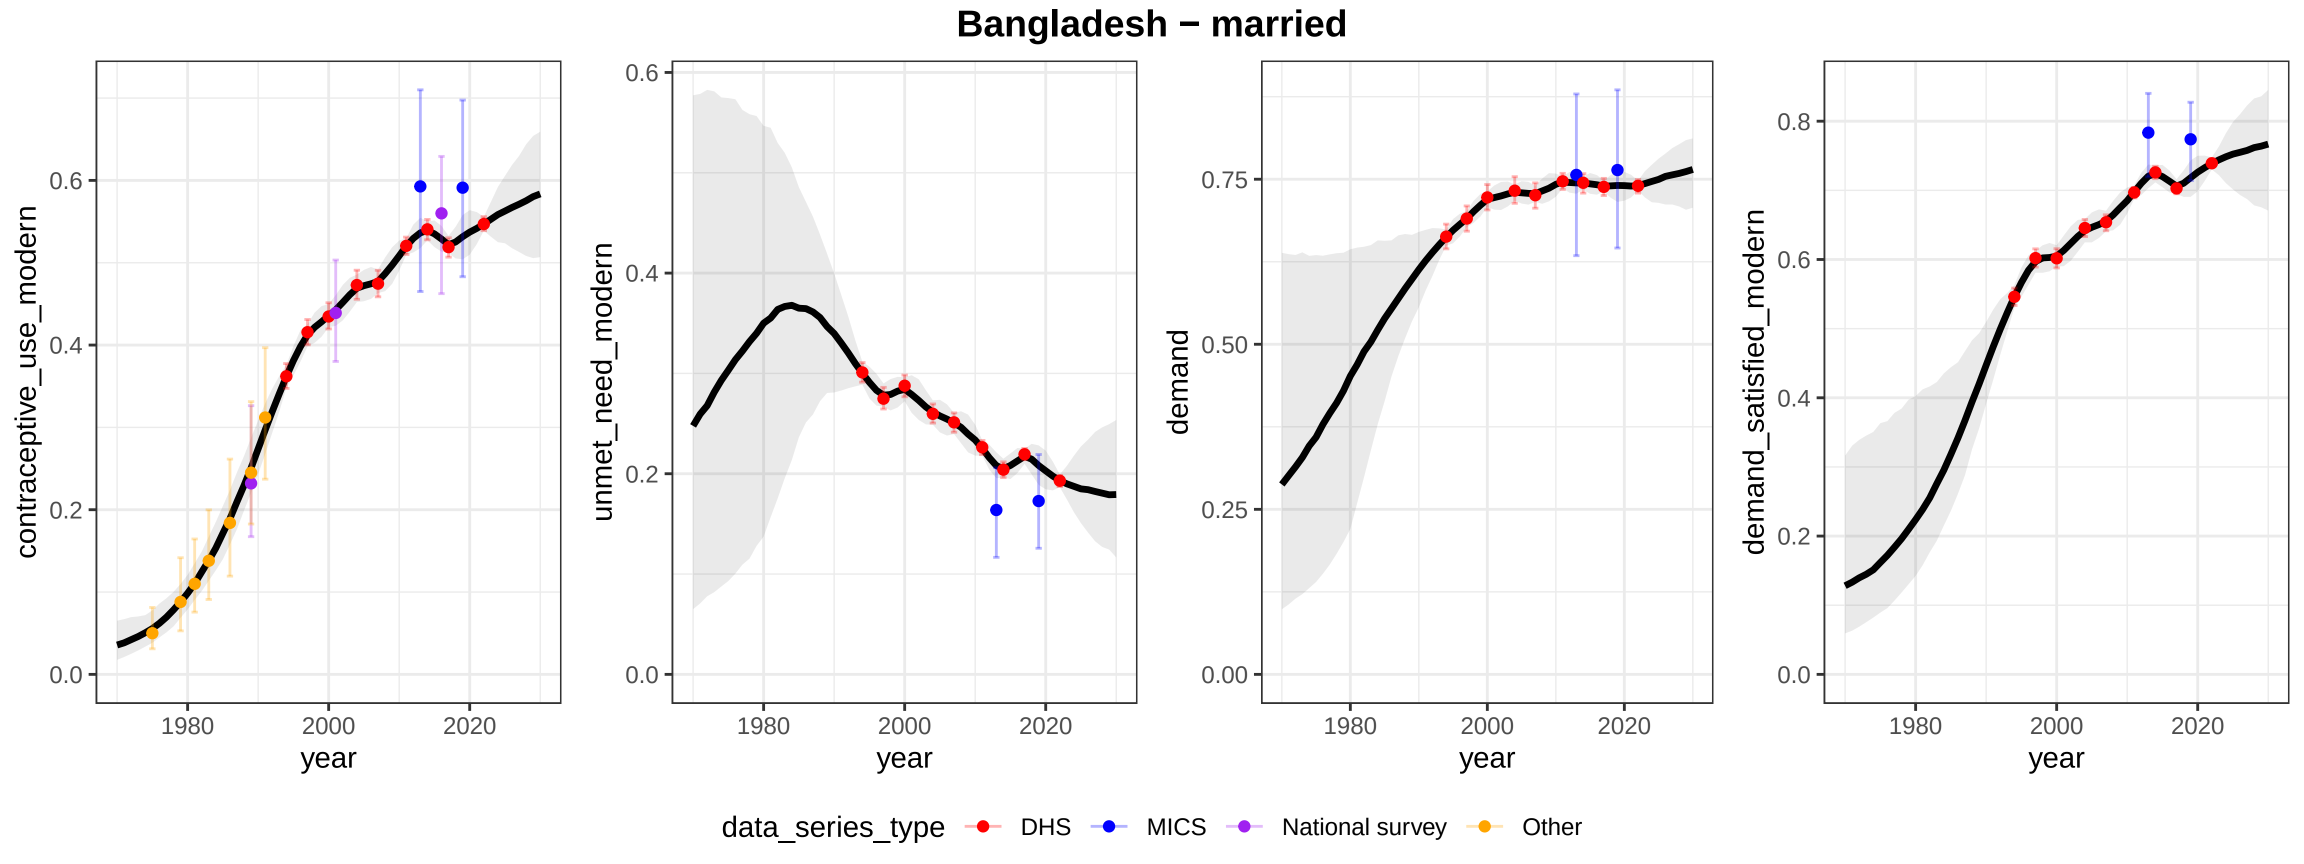

Bangladesh − married
contraceptive_use_modern
unmet_need_modern
demand
demand_satisfied_modern
year
1980
2000
2020
0.0
0.2
0.4
0.6
0.8
0.00
0.25
0.50
0.75
data_series_type
DHS
MICS
National survey
Other

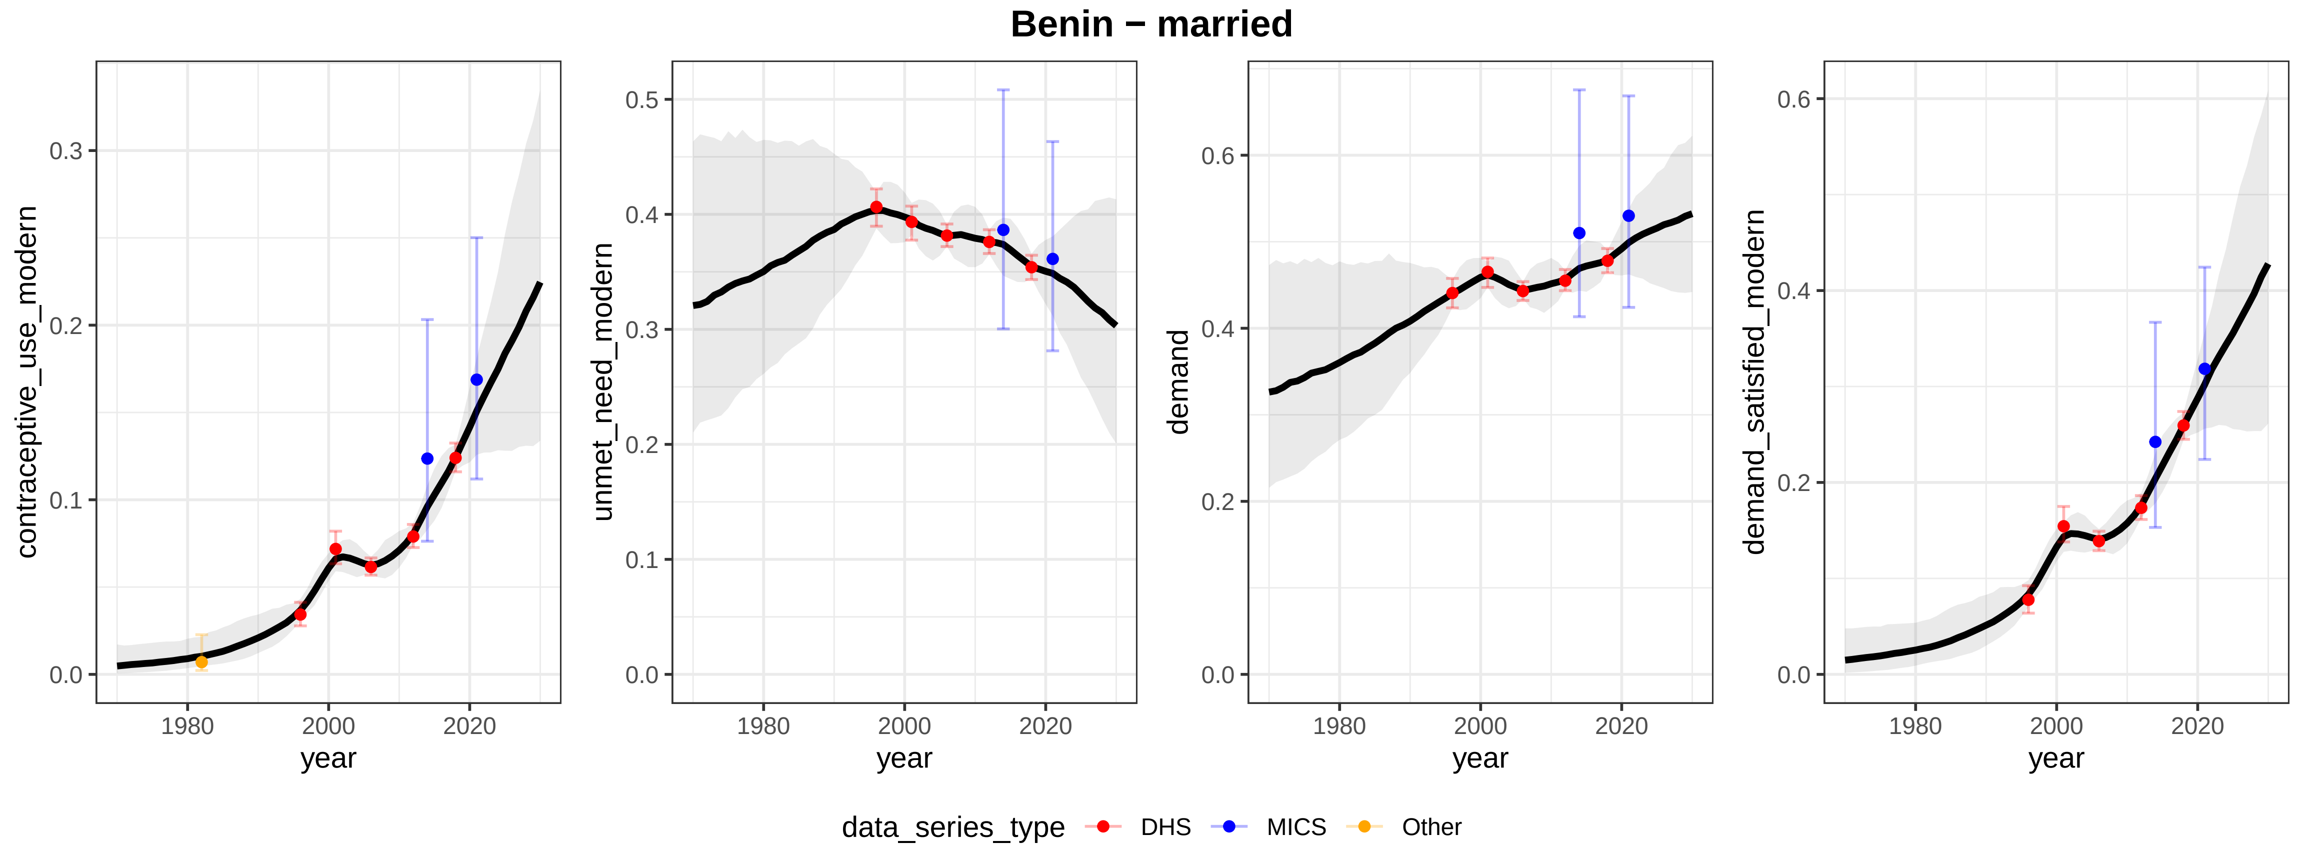
Benin − married
contraceptive_use_modern
unmet_need_modern
demand
demand_satisfied_modern
year
data_series_type
DHS
MICS
Other

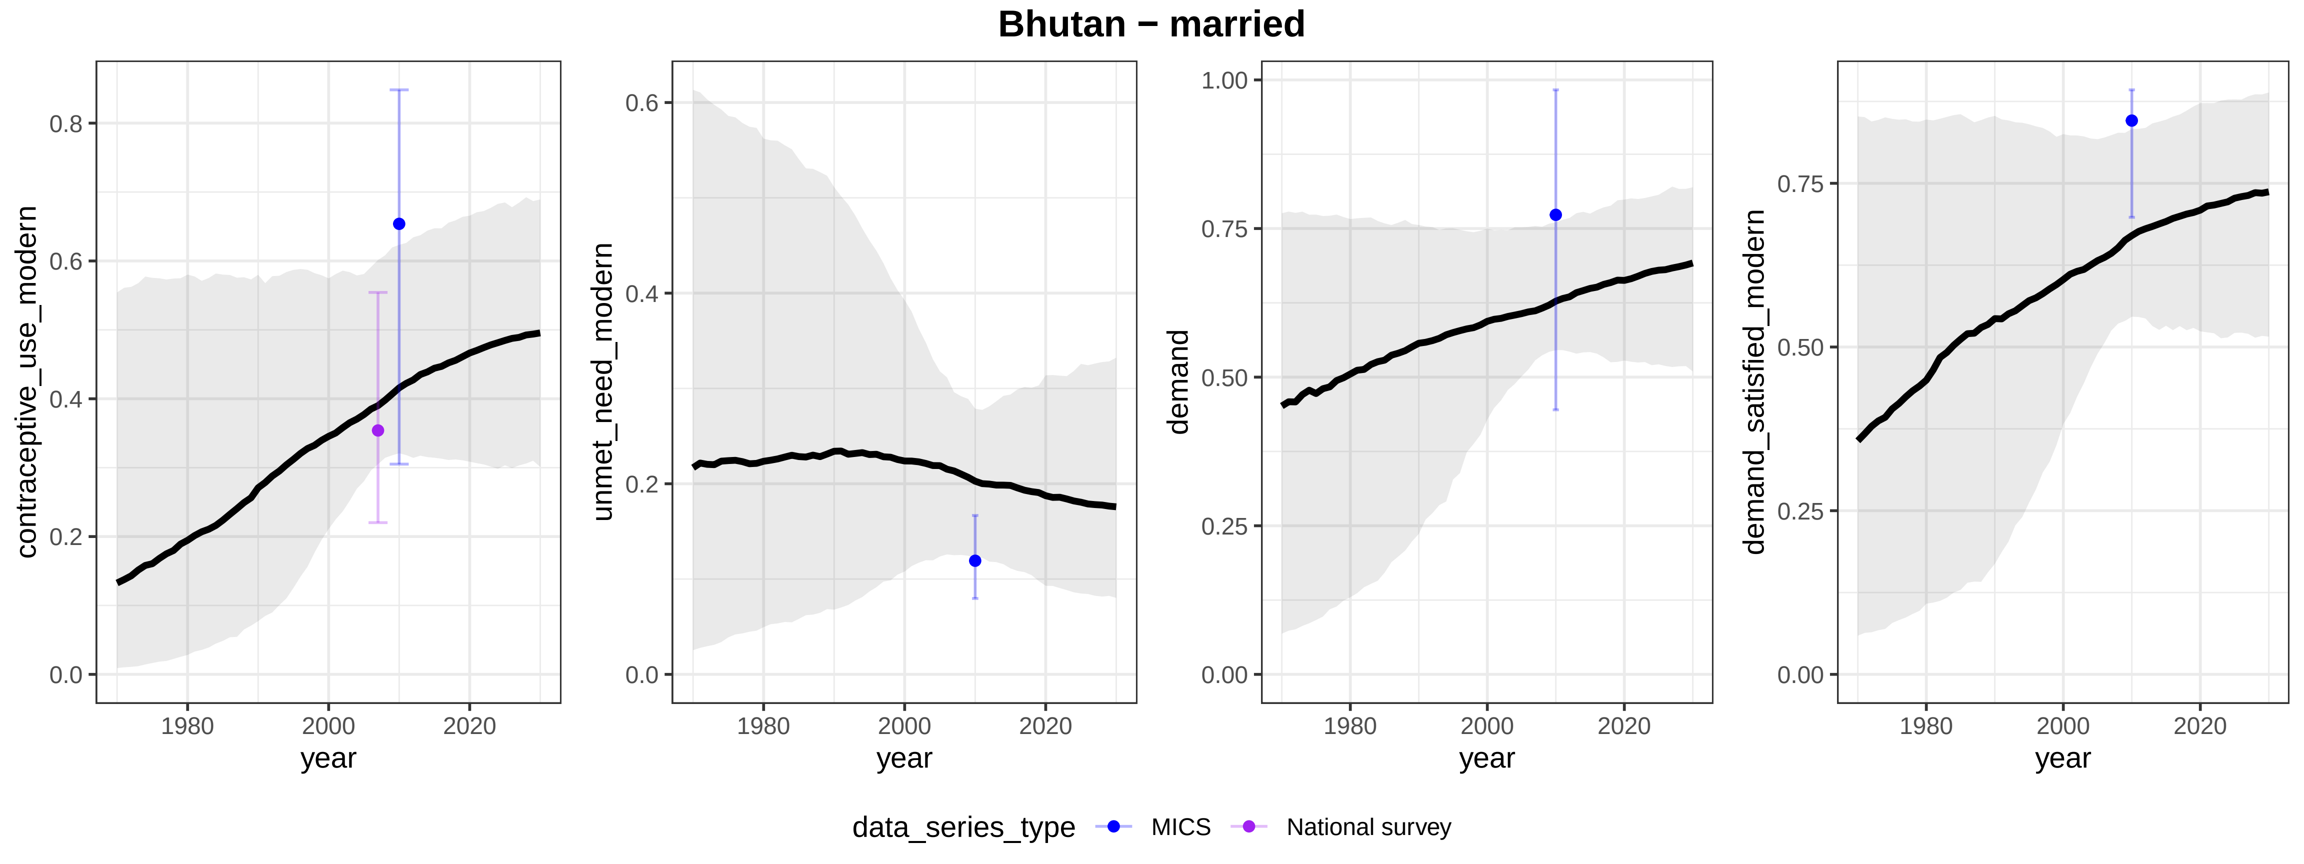
Bhutan − married
contraceptive_use_modern
unmet_need_modern
demand
demand_satisfied_modern
0.0
0.2
0.4
0.6
0.8
0.00
0.25
0.50
0.75
1.00
1980
2000
2020
year
data_series_type
MICS
National survey

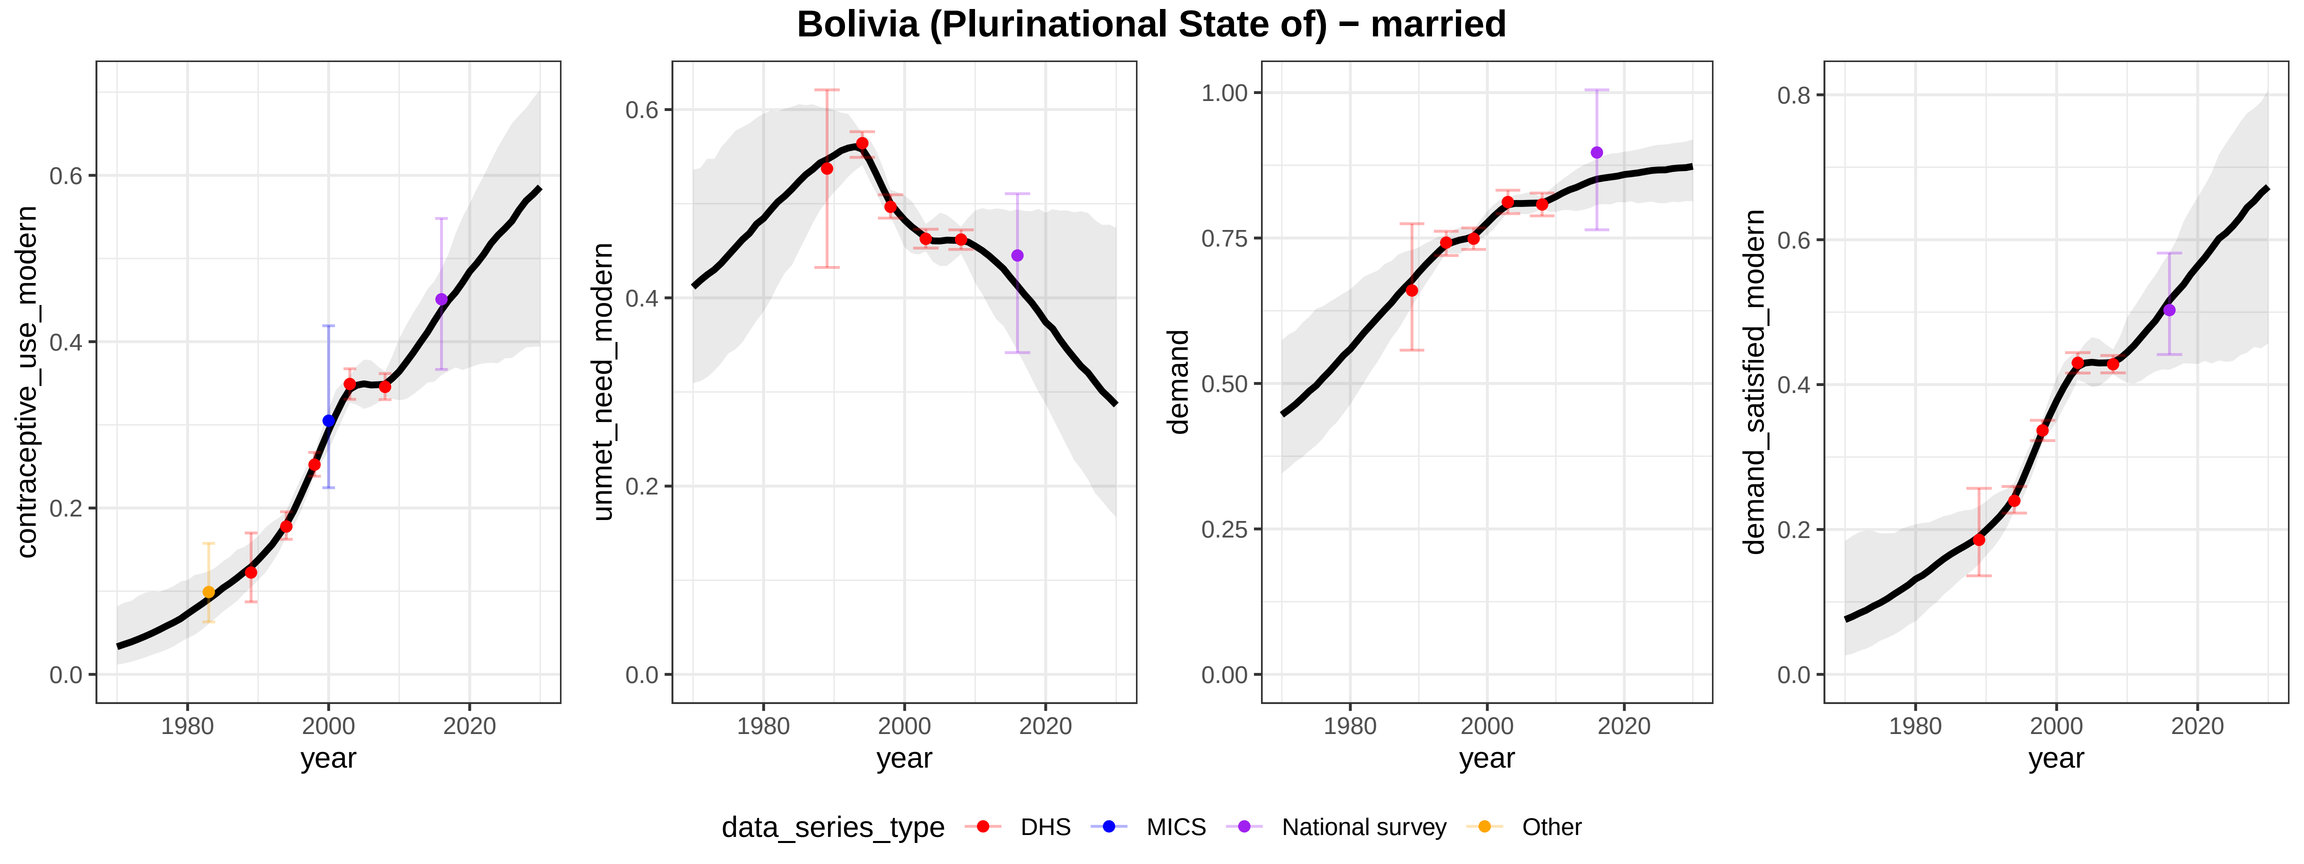

Bolivia (Plurinational State of) − married
contraceptive_use_modern
unmet_need_modern
demand
demand_satisfied_modern
year
1980
2000
2020
0.0
0.2
0.4
0.6
0.8
0.00
0.25
0.50
0.75
1.00
data_series_type
DHS
MICS
National survey
Other

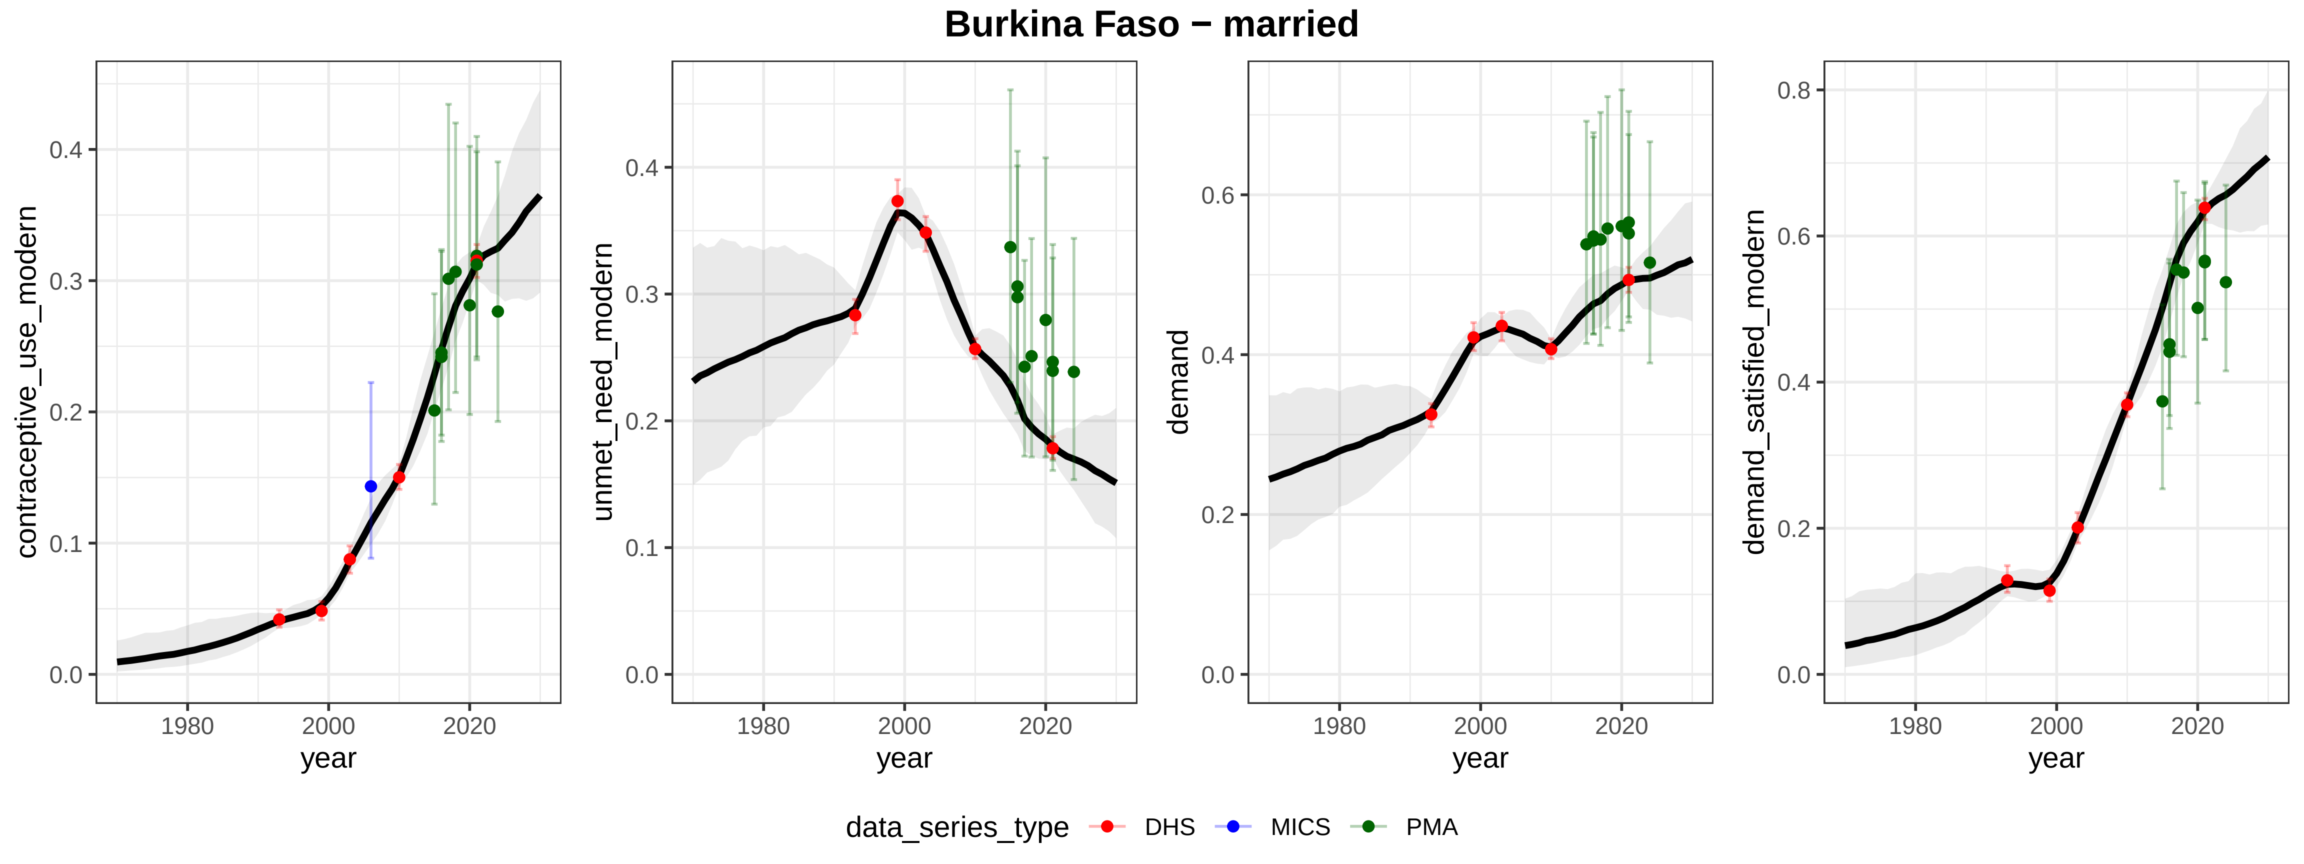

Burkina Faso − married
contraceptive_use_modern
unmet_need_modern
demand
demand_satisfied_modern
0.0
0.1
0.2
0.3
0.4
0.6
0.8
1980
2000
2020
year
data_series_type
DHS
MICS
PMA

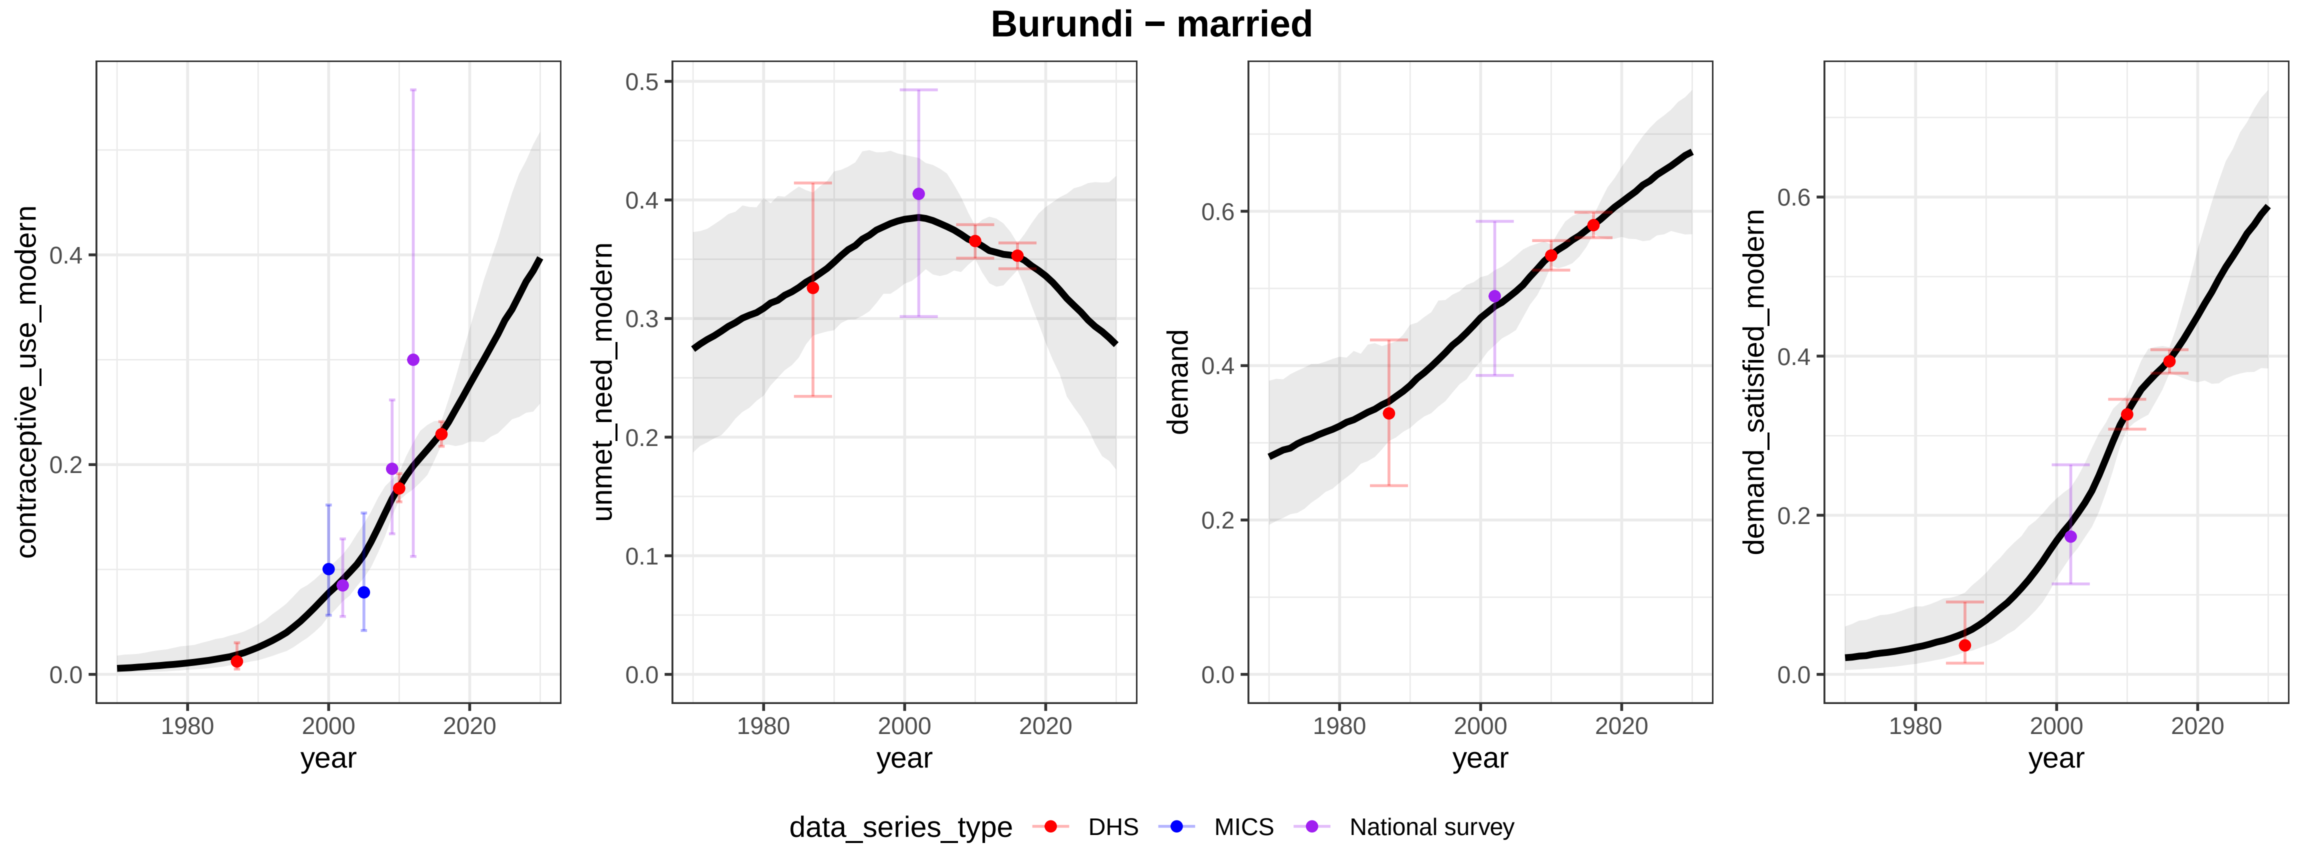

Burundi − married
contraceptive_use_modern
unmet_need_modern
demand
demand_satisfied_modern
year
0.0
0.2
0.4
0.1
0.3
0.5
0.6
1980
2000
2020
data_series_type
DHS
MICS
National survey

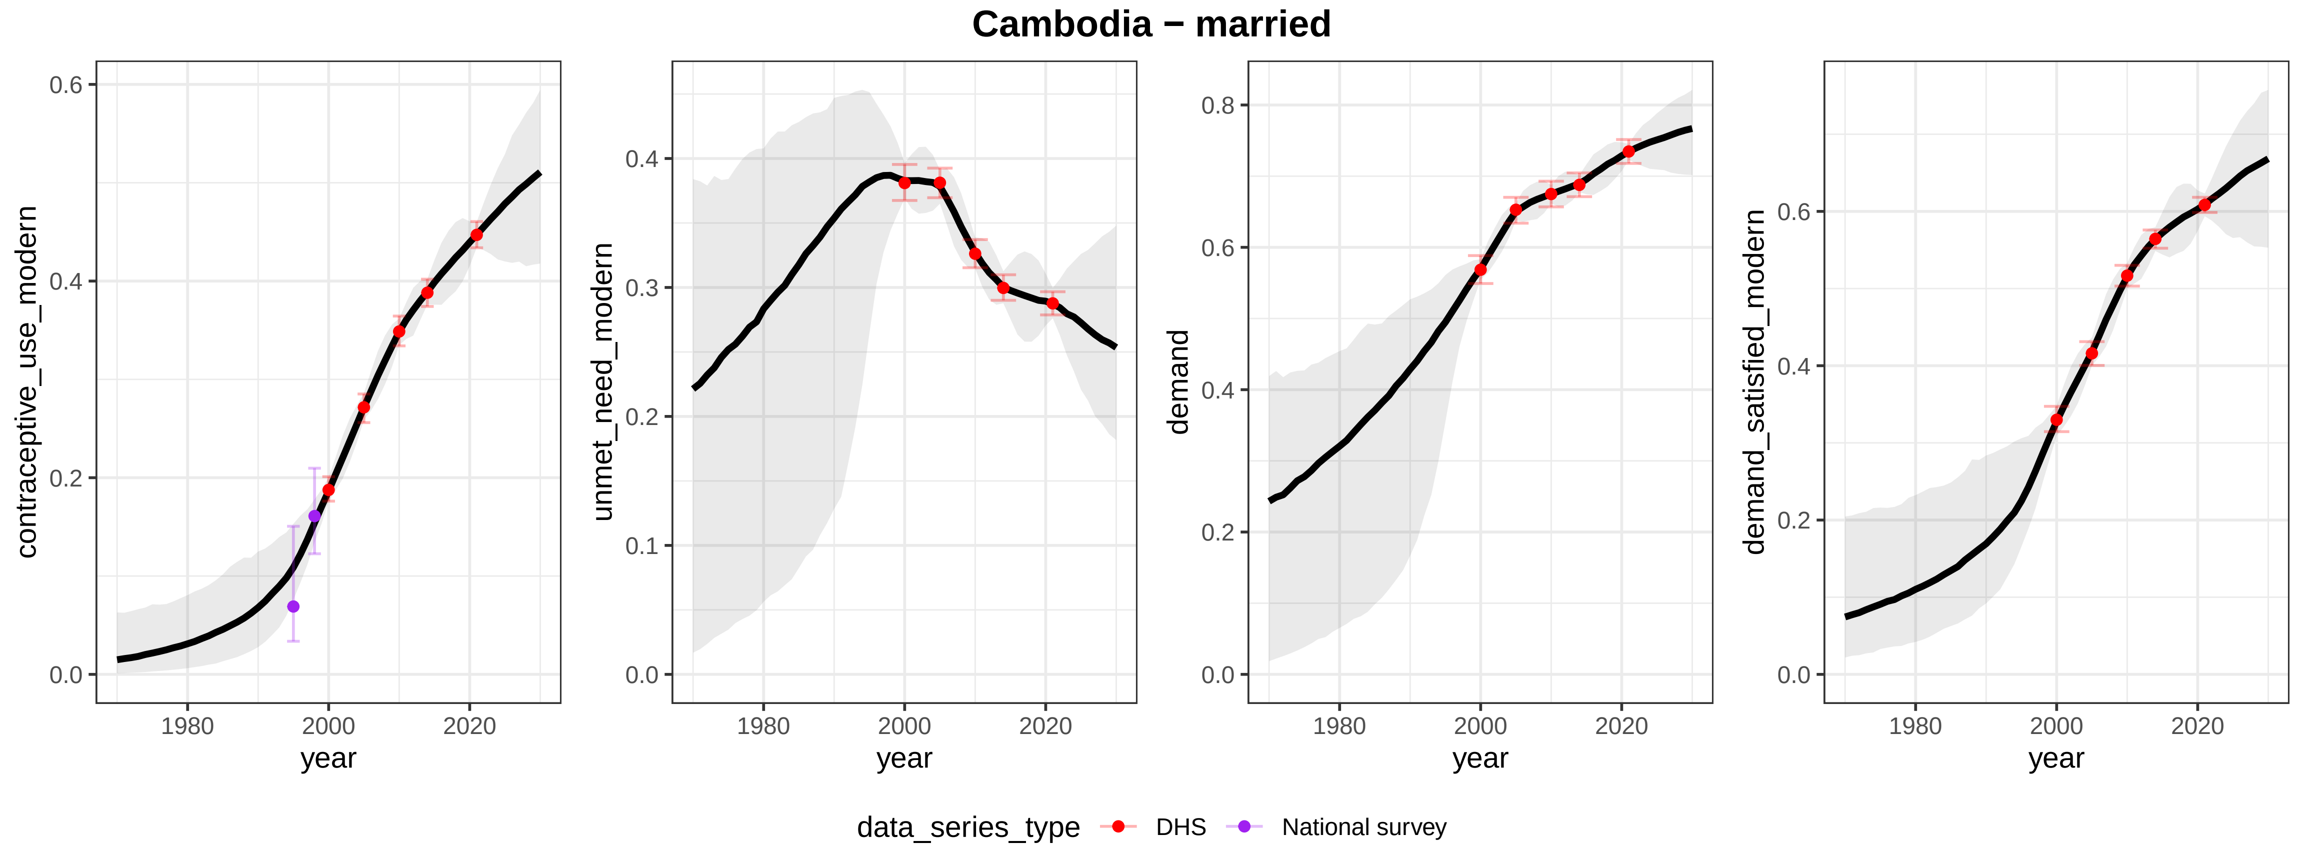
Cambodia − married
contraceptive_use_modern
unmet_need_modern
demand
demand_satisfied_modern
year
1980
2000
2020
0.0
0.2
0.4
0.6
0.1
0.3
0.8
data_series_type
DHS
National survey

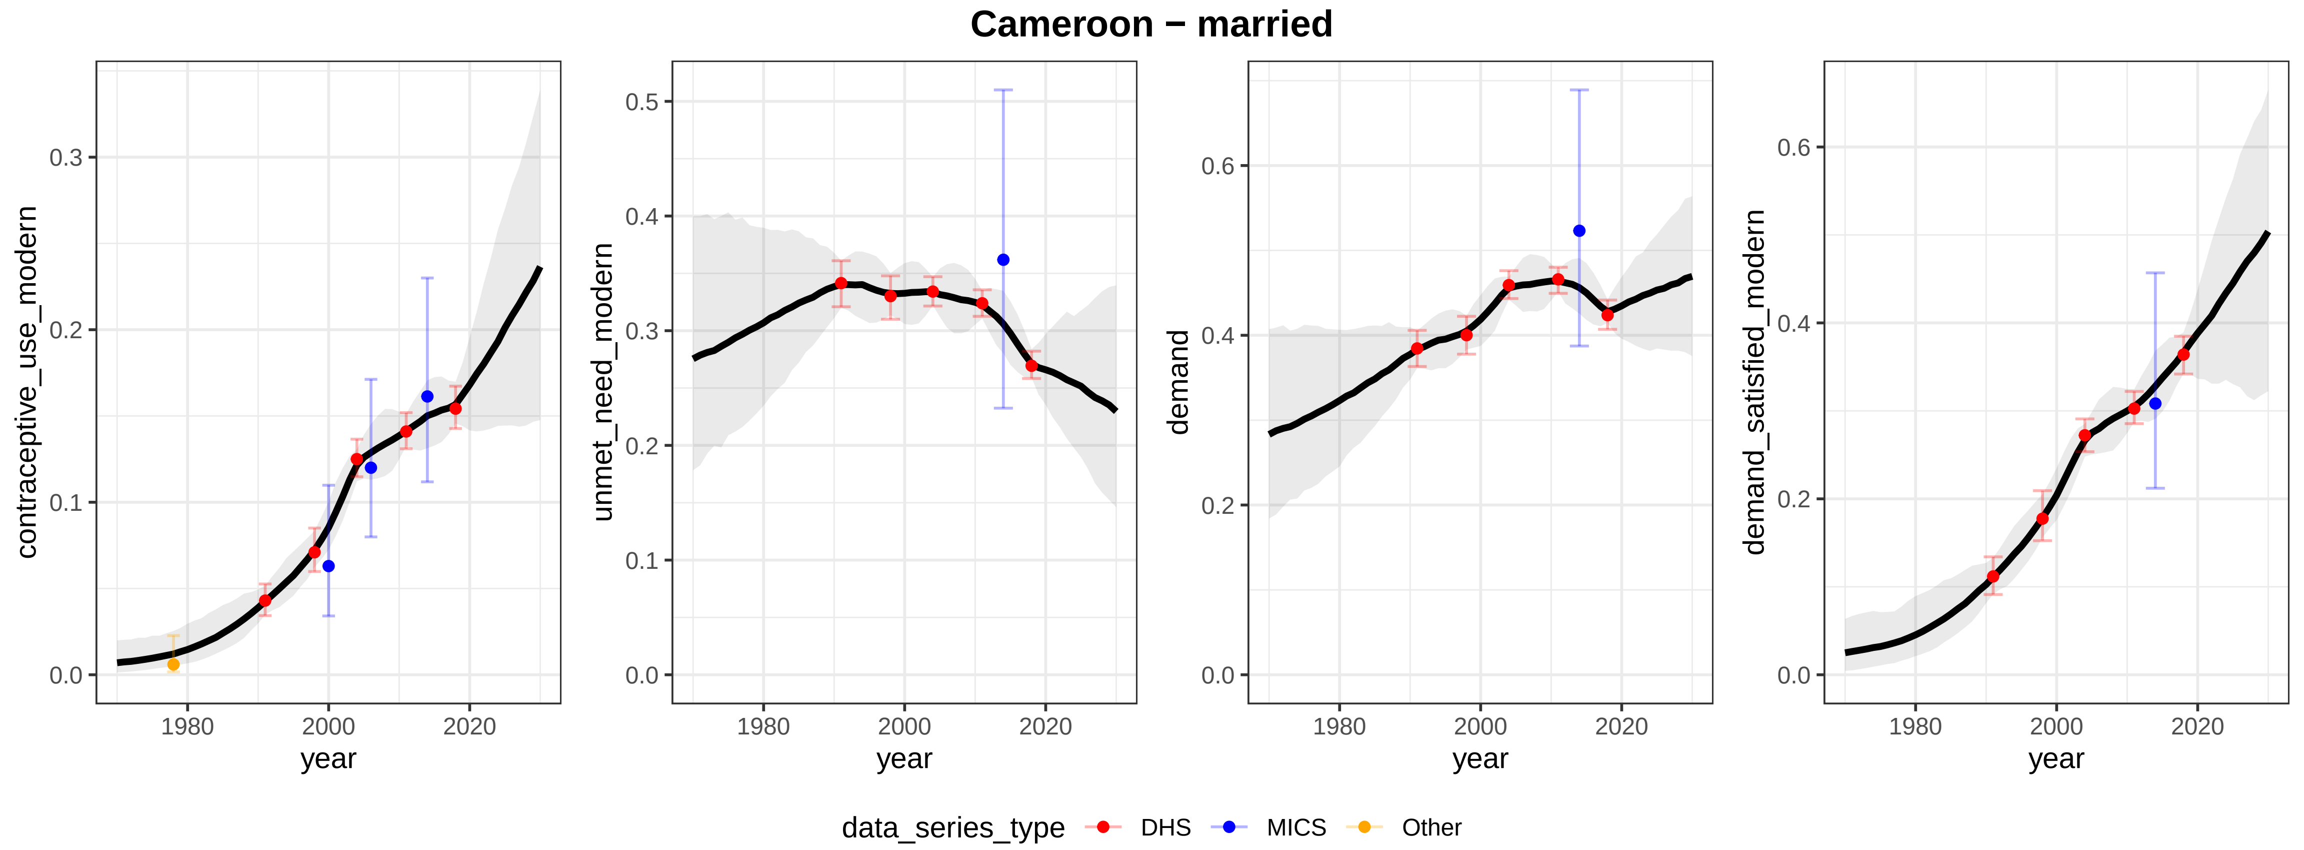

Cameroon − married
contraceptive_use_modern
unmet_need_modern
demand
demand_satisfied_modern
year
1980
2000
2020
0.0
0.1
0.2
0.3
0.4
0.5
0.6
data_series_type
DHS
MICS
Other

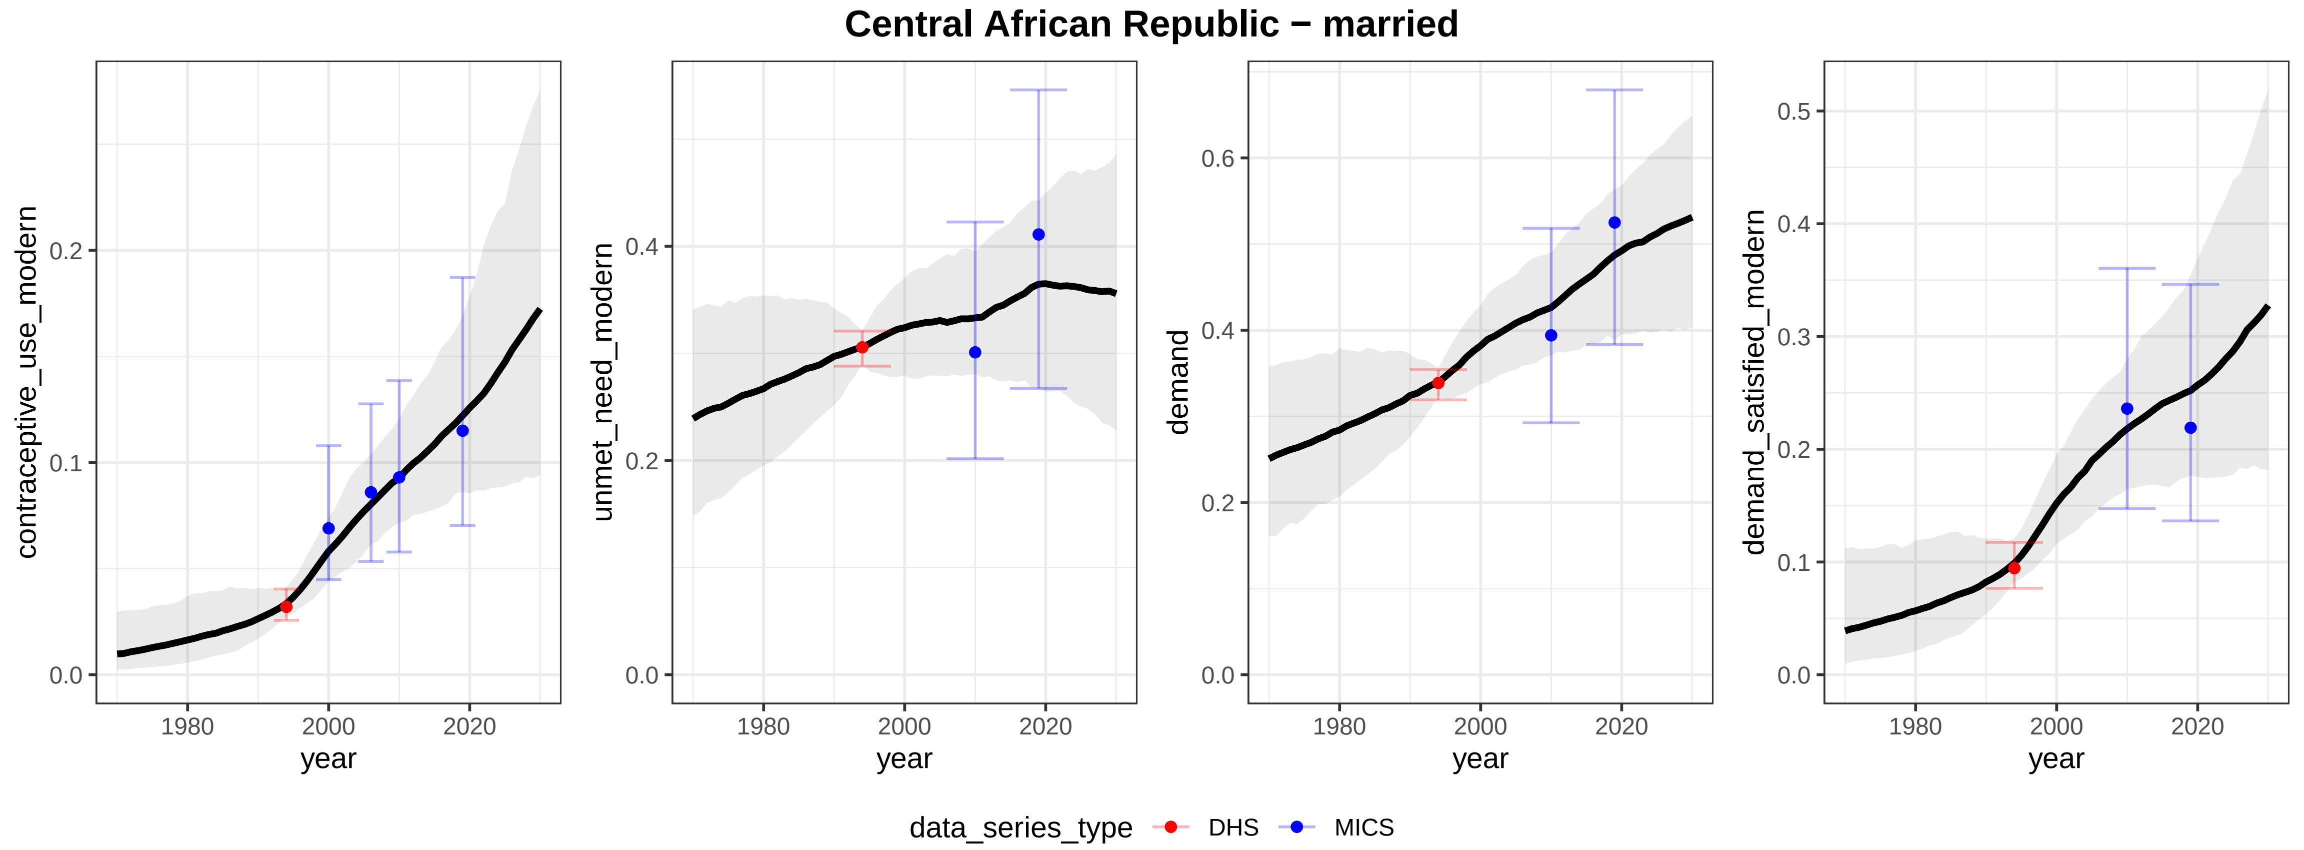

Central African Republic − married
contraceptive_use_modern
0.0
0.1
0.2
year
1980
2000
2020
unmet_need_modern
0.0
0.2
0.4
demand
0.0
0.2
0.4
0.6
demand_satisfied_modern
0.0
0.1
0.2
0.3
0.4
0.5
data_series_type
DHS
MICS

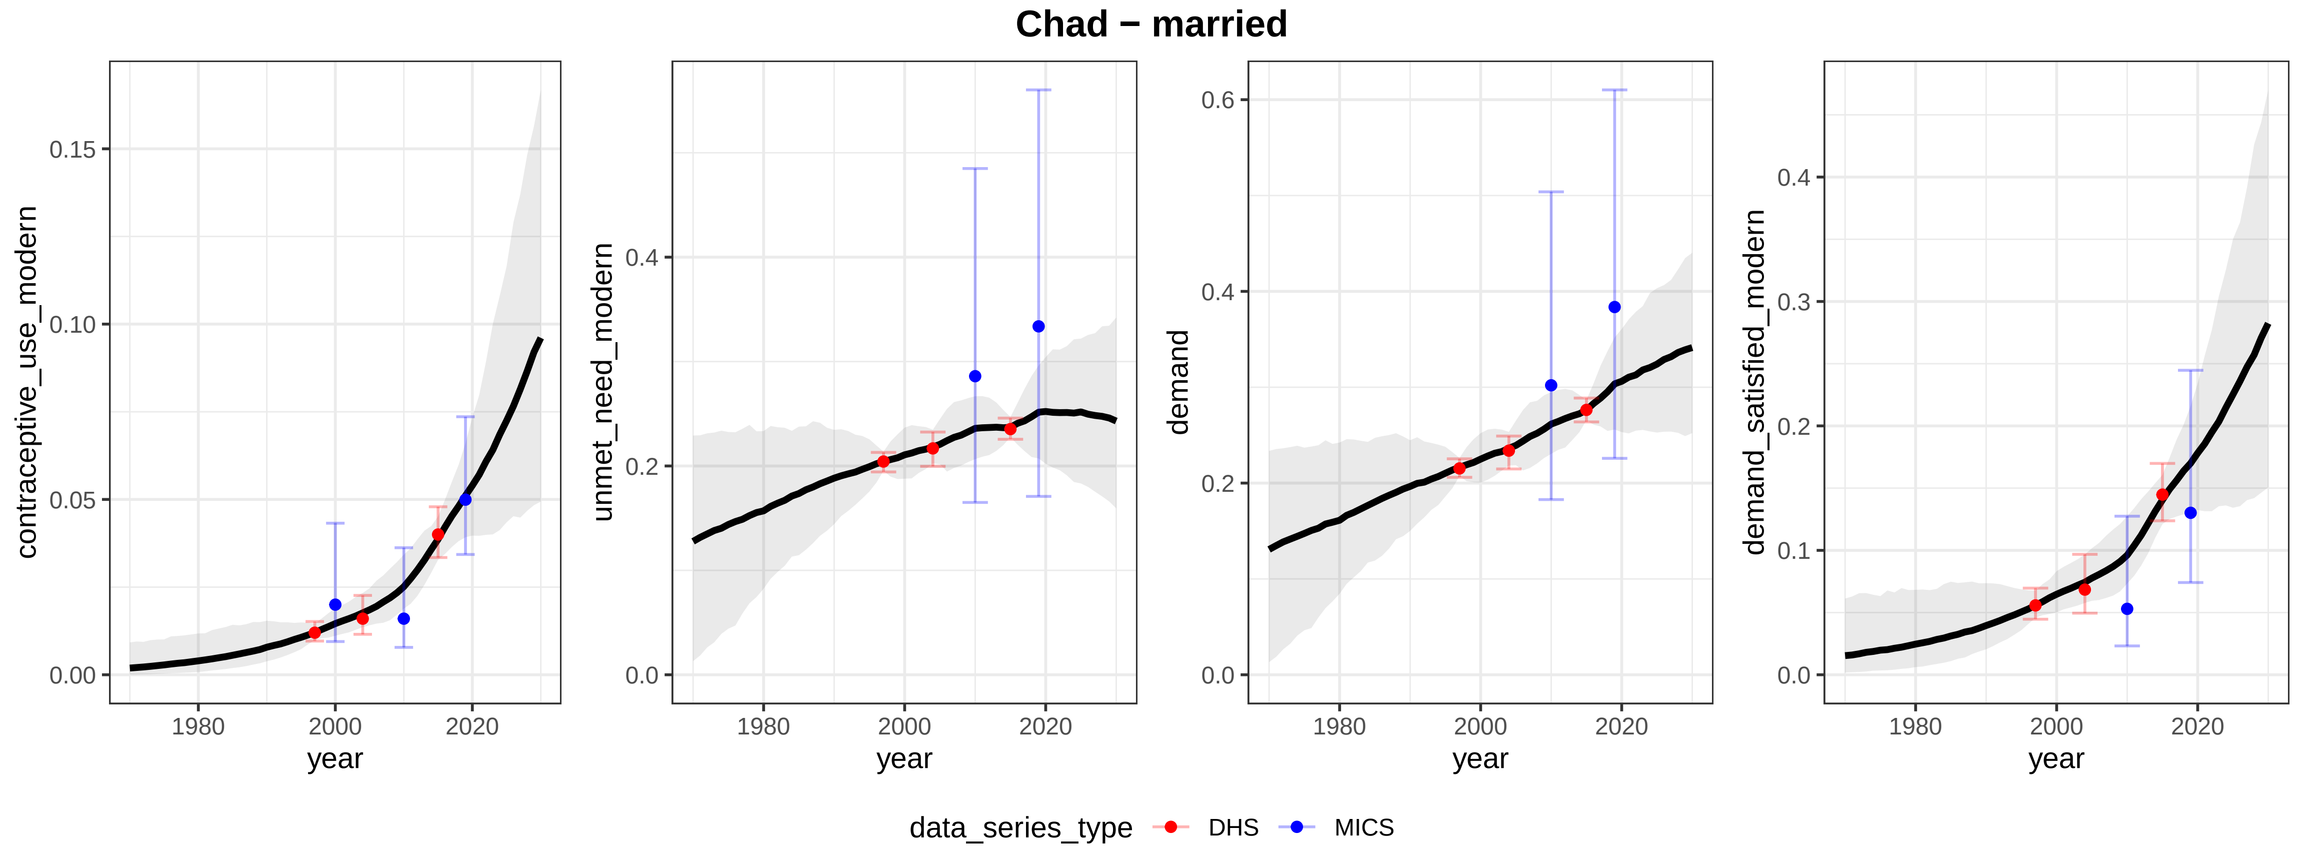
Chad − married
contraceptive_use_modern
0.00
0.05
0.10
0.15
unmet_need_modern
0.0
0.2
0.4
demand
0.0
0.2
0.4
0.6
demand_satisfied_modern
0.0
0.1
0.2
0.3
0.4
1980
2000
2020
year
data_series_type
DHS
MICS

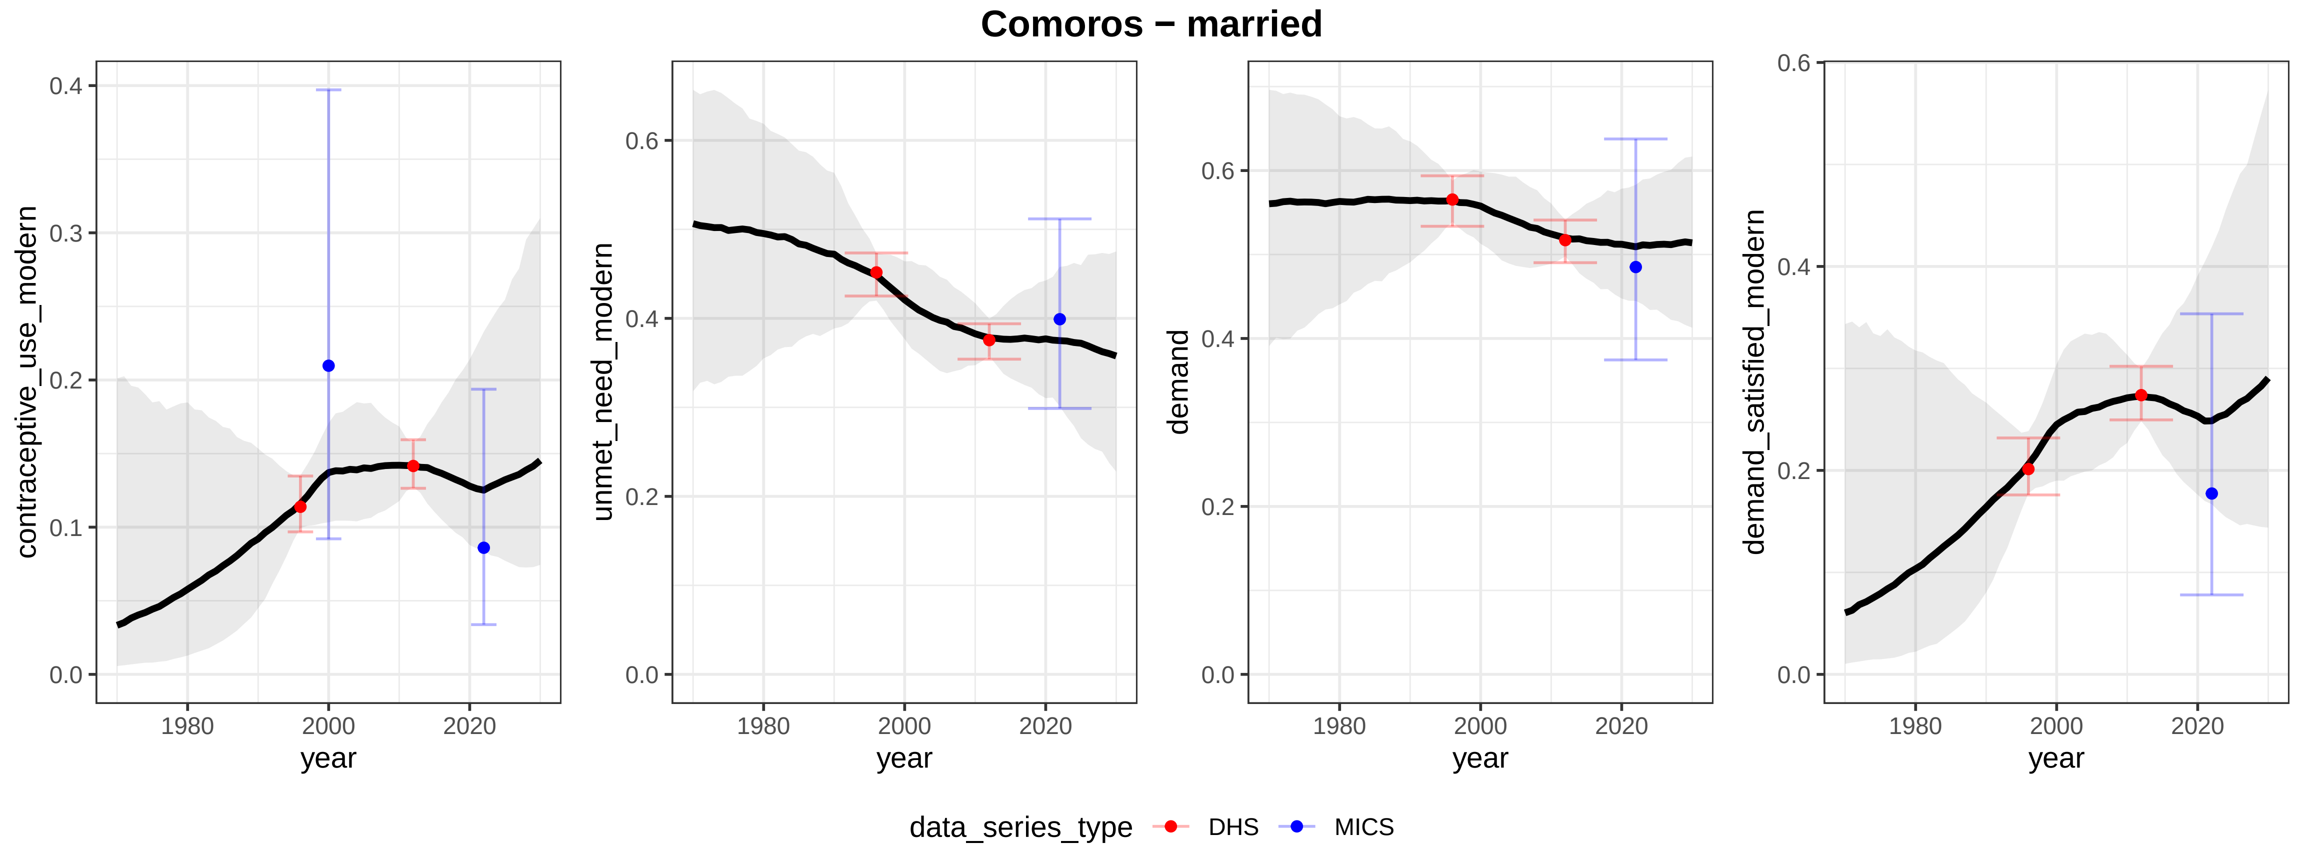

Comoros − married
contraceptive_use_modern
unmet_need_modern
demand
demand_satisfied_modern
year
0.0
0.1
0.2
0.3
0.4
0.6
1980
2000
2020
data_series_type
DHS
MICS

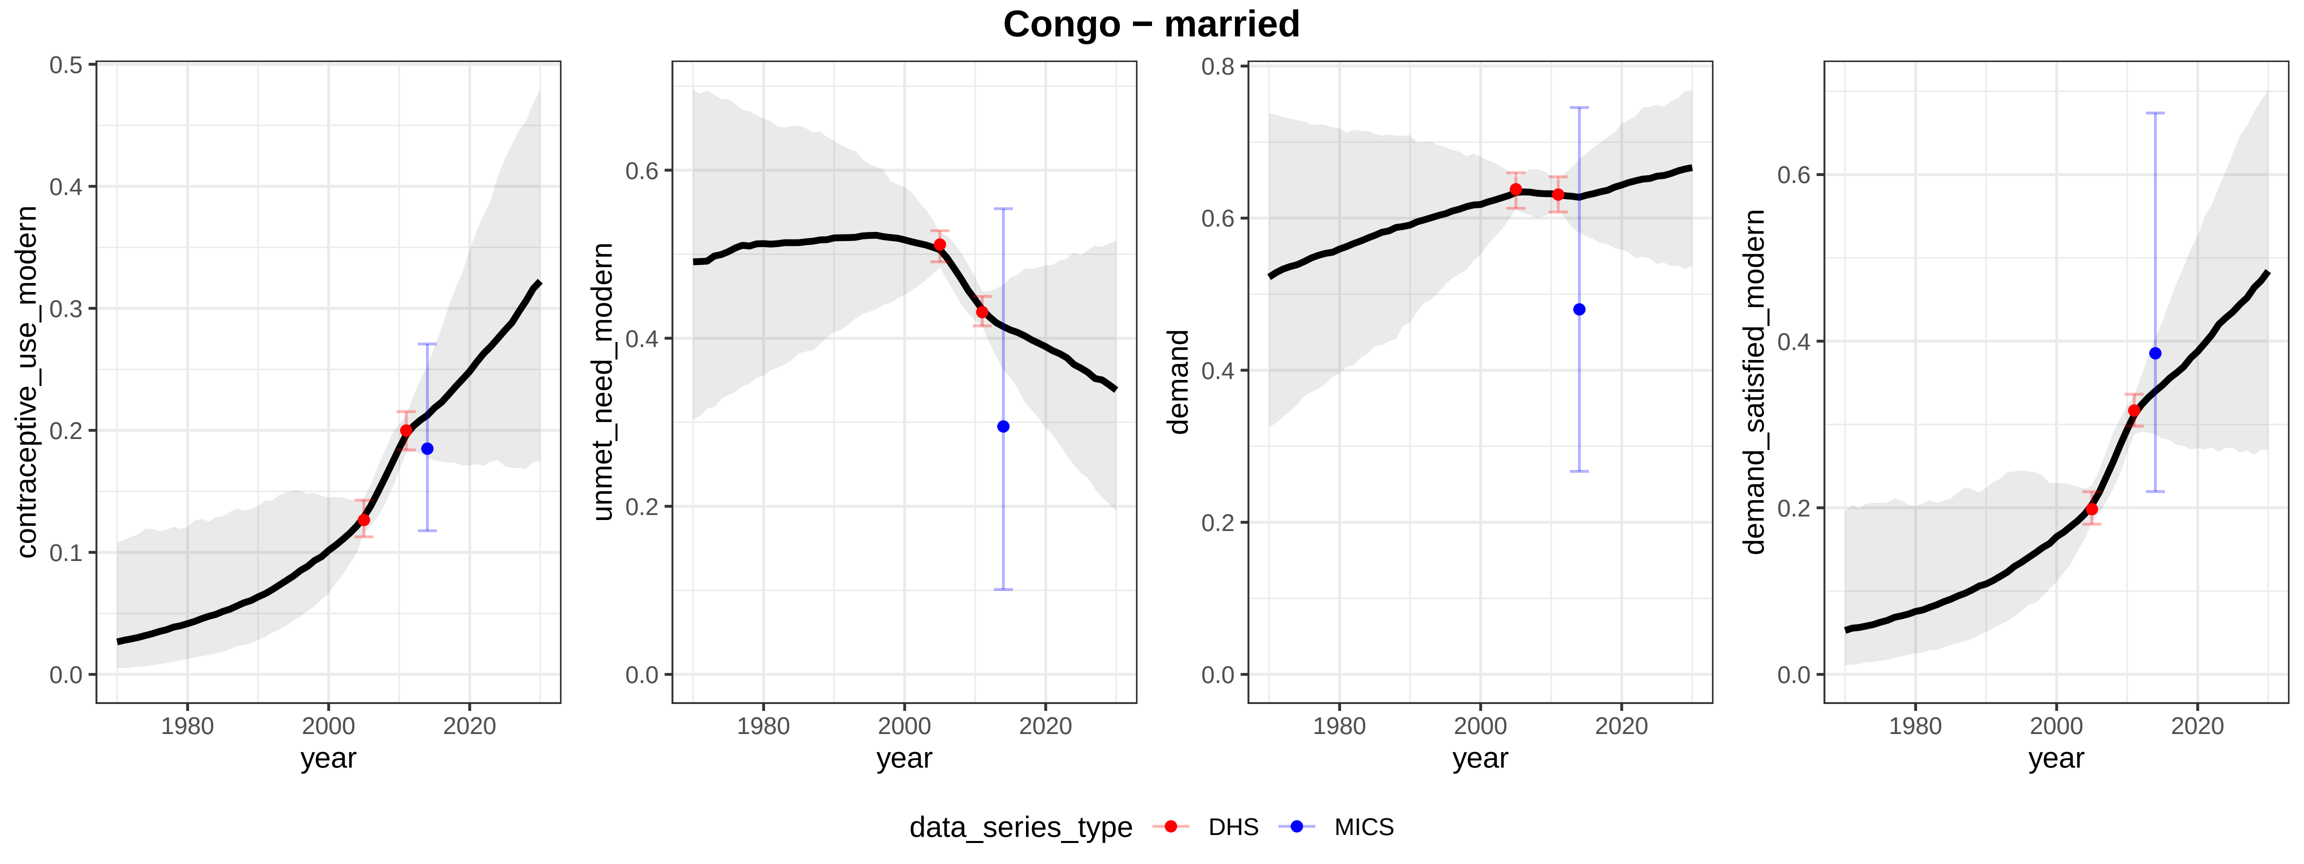
Congo − married
contraceptive_use_modern
unmet_need_modern
demand
demand_satisfied_modern
year
1980
2000
2020
0.0
0.1
0.2
0.3
0.4
0.5
0.6
0.8
data_series_type
DHS
MICS

# Côte d'Ivoire − married

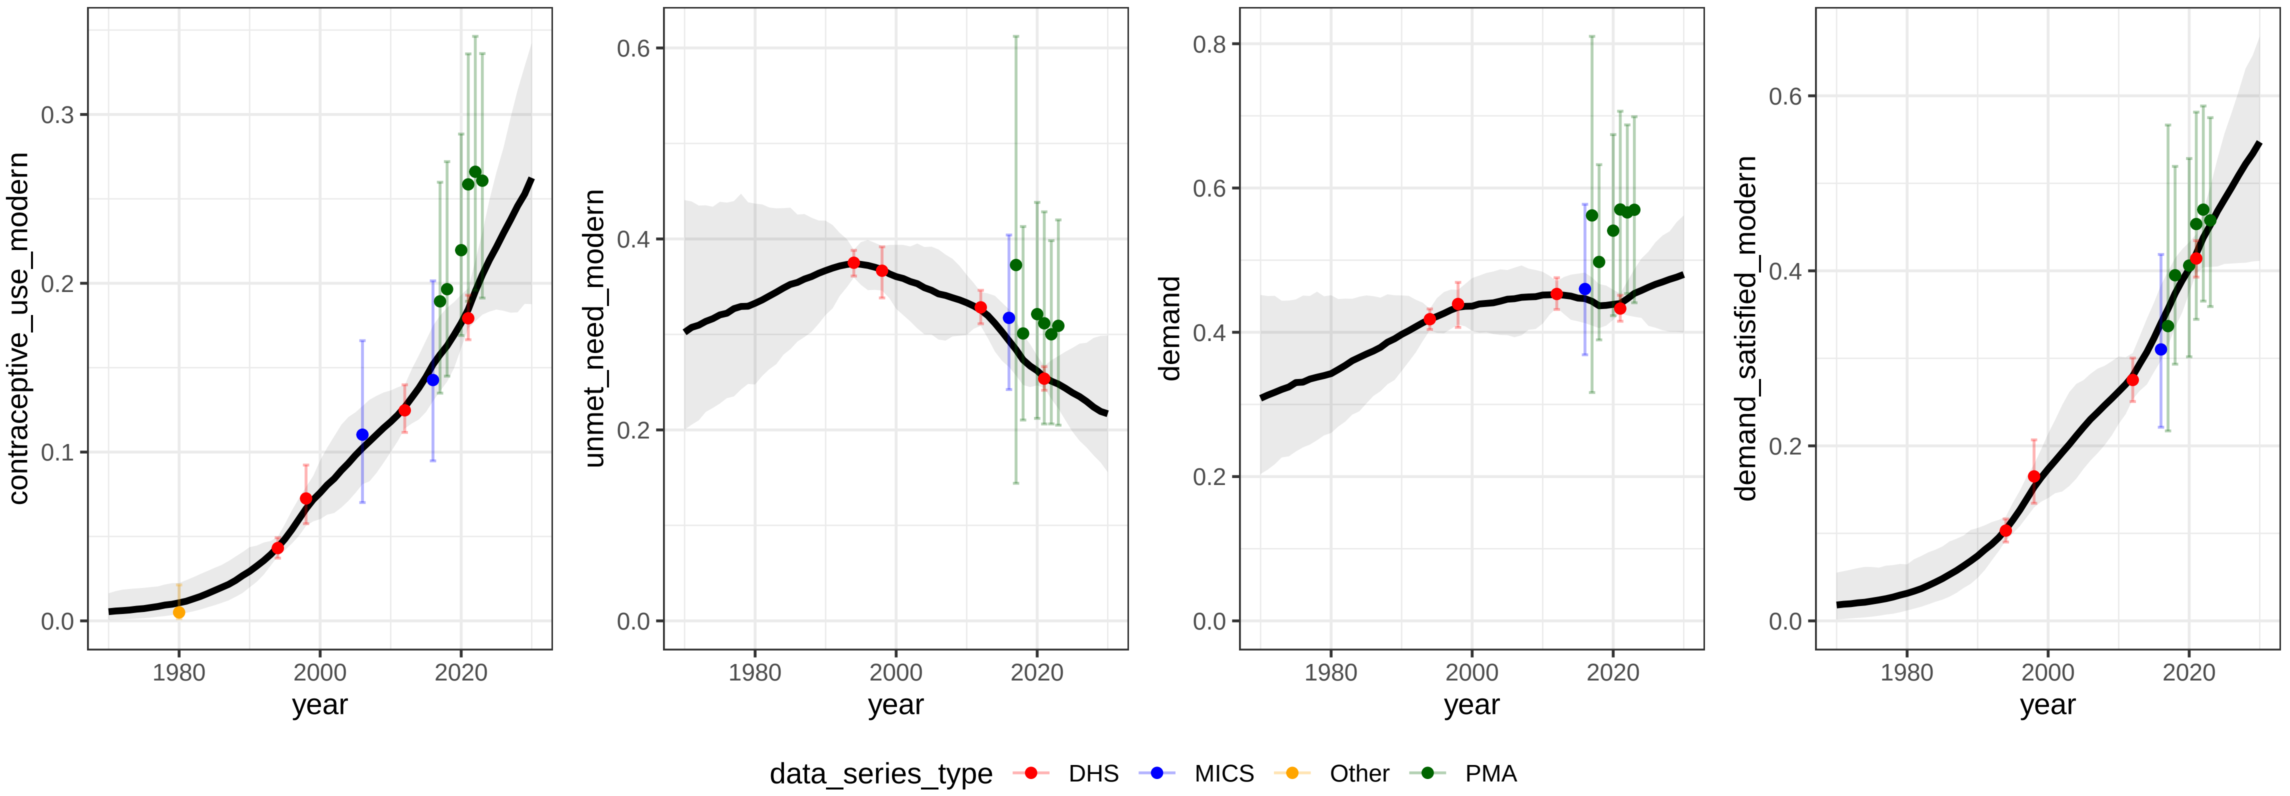

## Democratic People's Republic of Korea − married

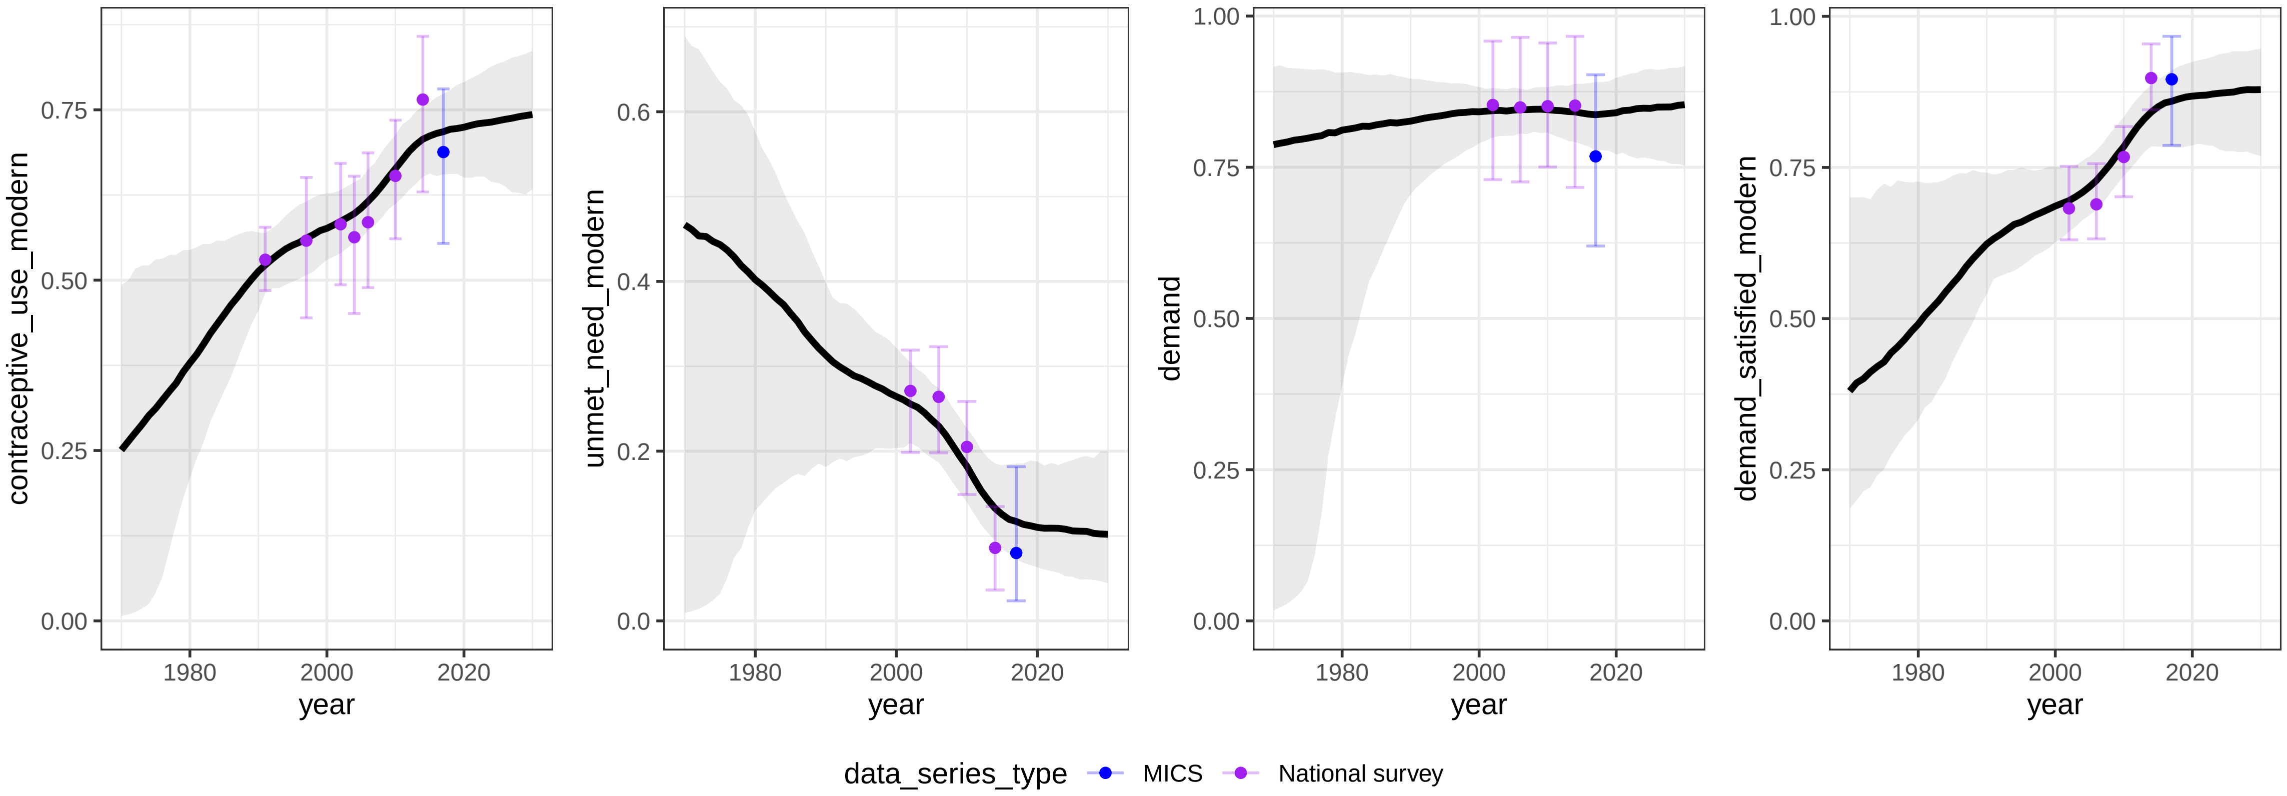

# Democratic Republic of the Congo − married

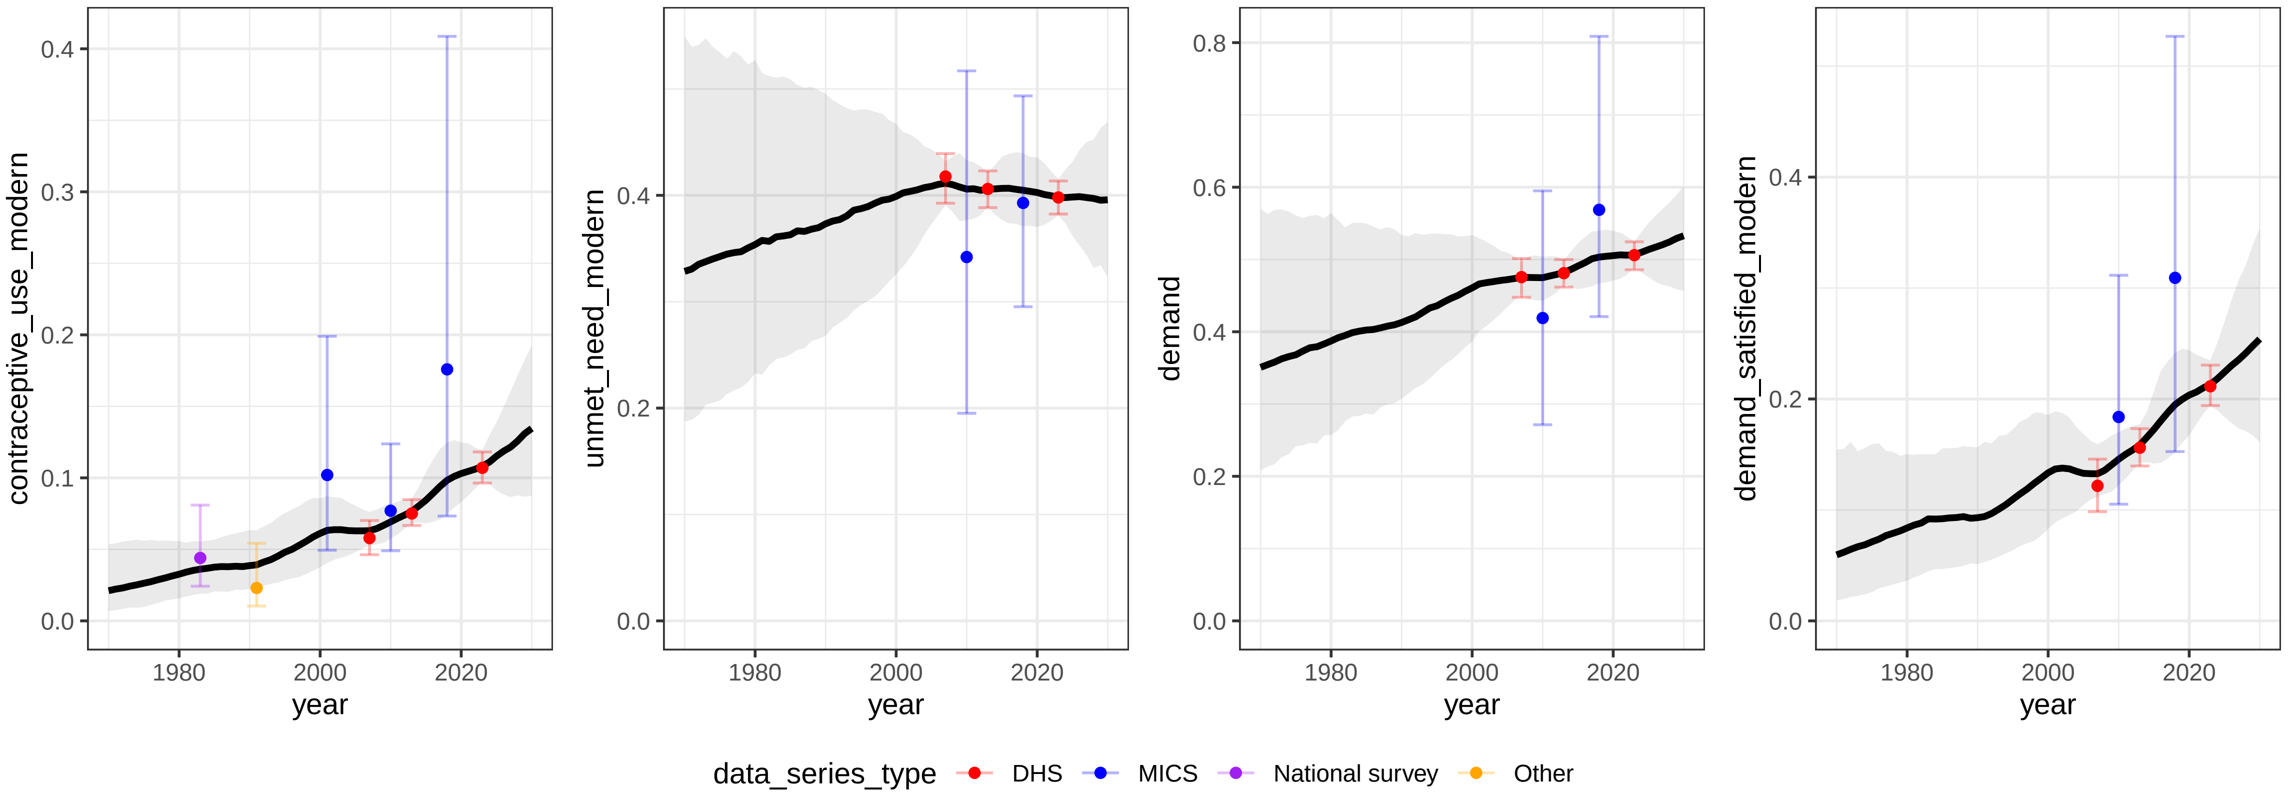

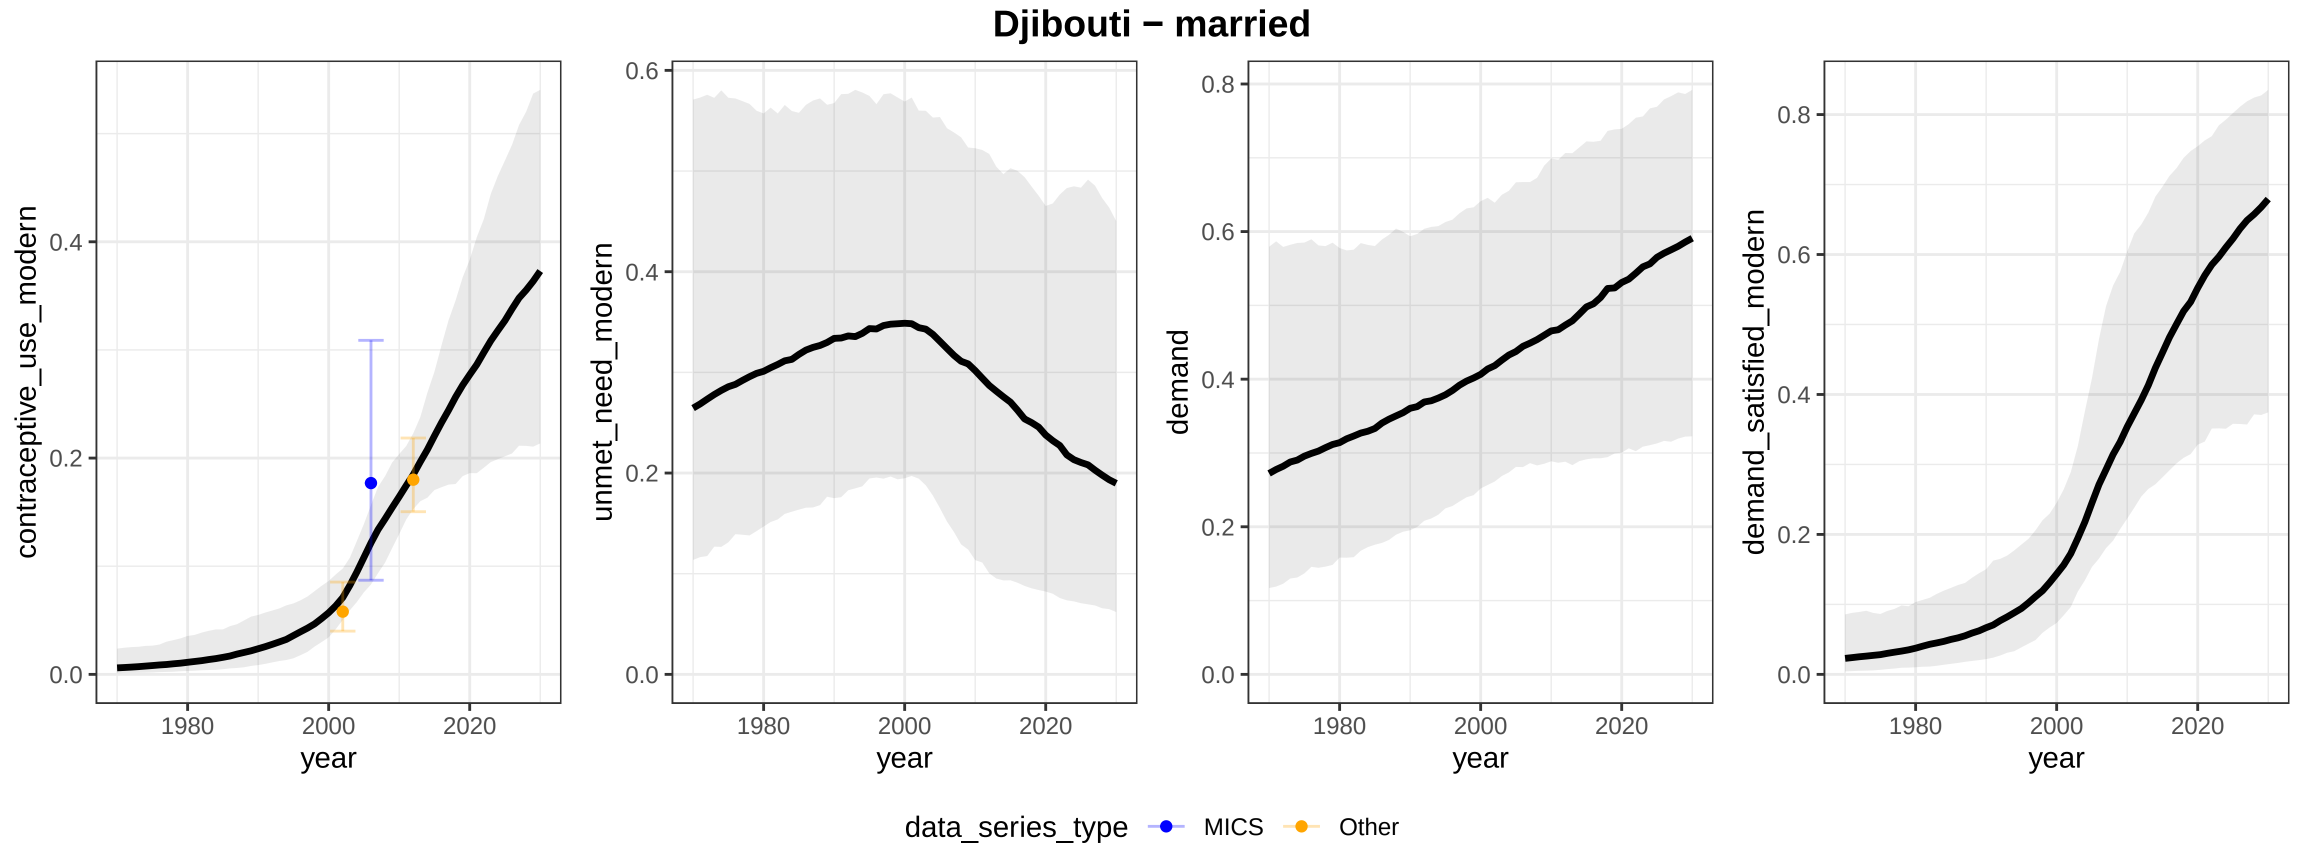
Djibouti − married
contraceptive_use_modern
unmet_need_modern
demand
demand_satisfied_modern
year
0.0
0.2
0.4
0.6
0.8
1980
2000
2020
data_series_type
MICS
Other

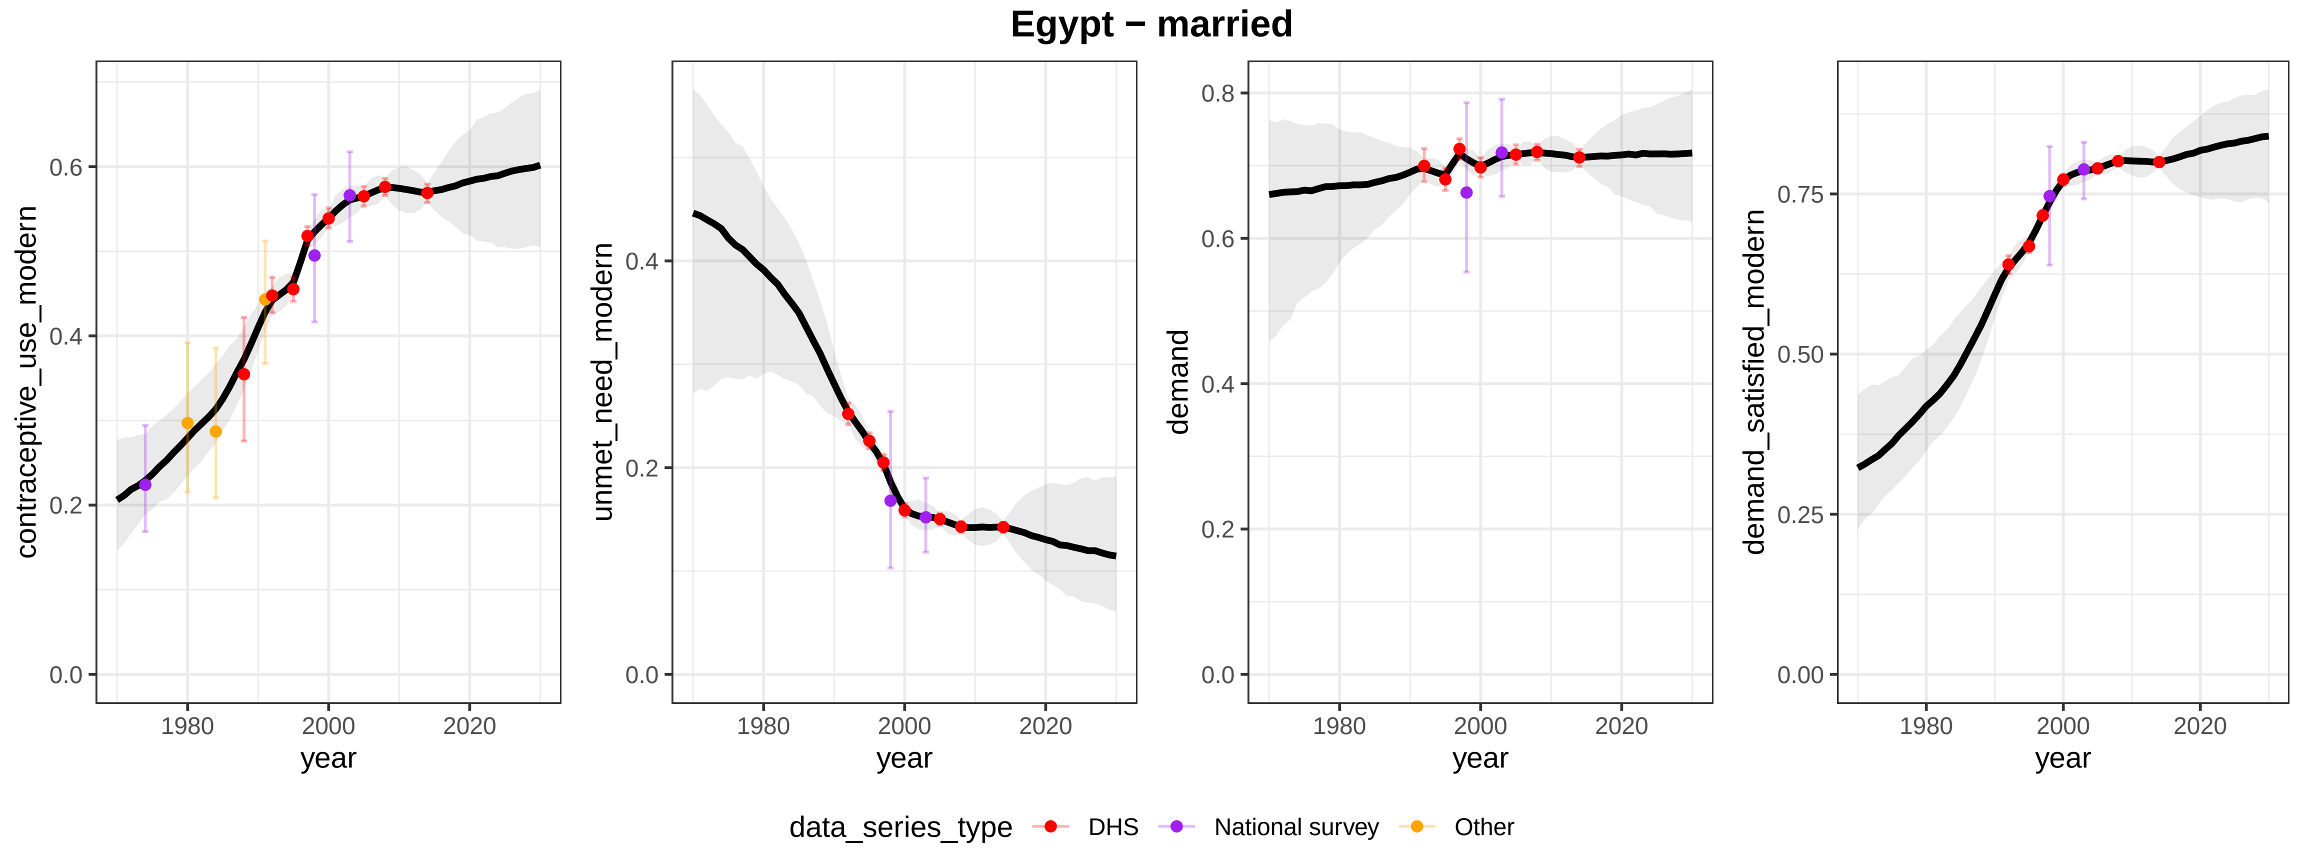
Egypt − married
contraceptive_use_modern
unmet_need_modern
demand
demand_satisfied_modern
year
0.0
0.2
0.4
0.6
0.8
0.00
0.25
0.50
0.75
1980
2000
2020
data_series_type
DHS
National survey
Other

# Eritrea − married

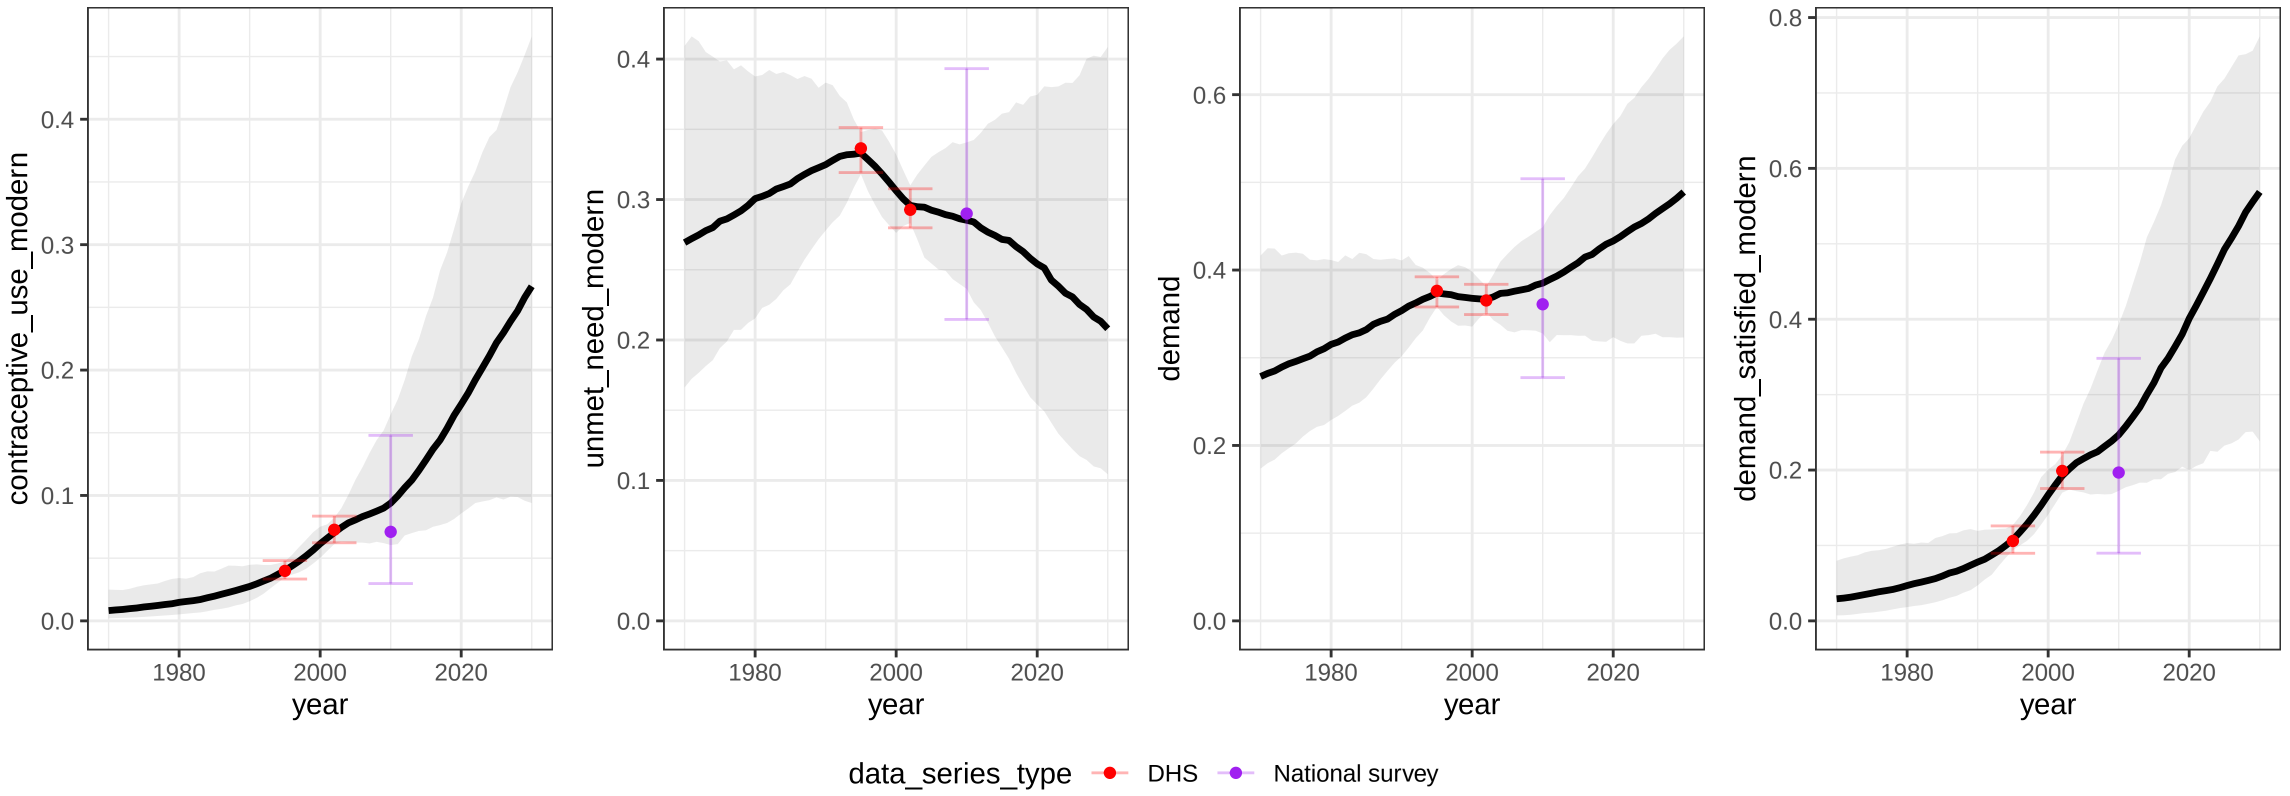

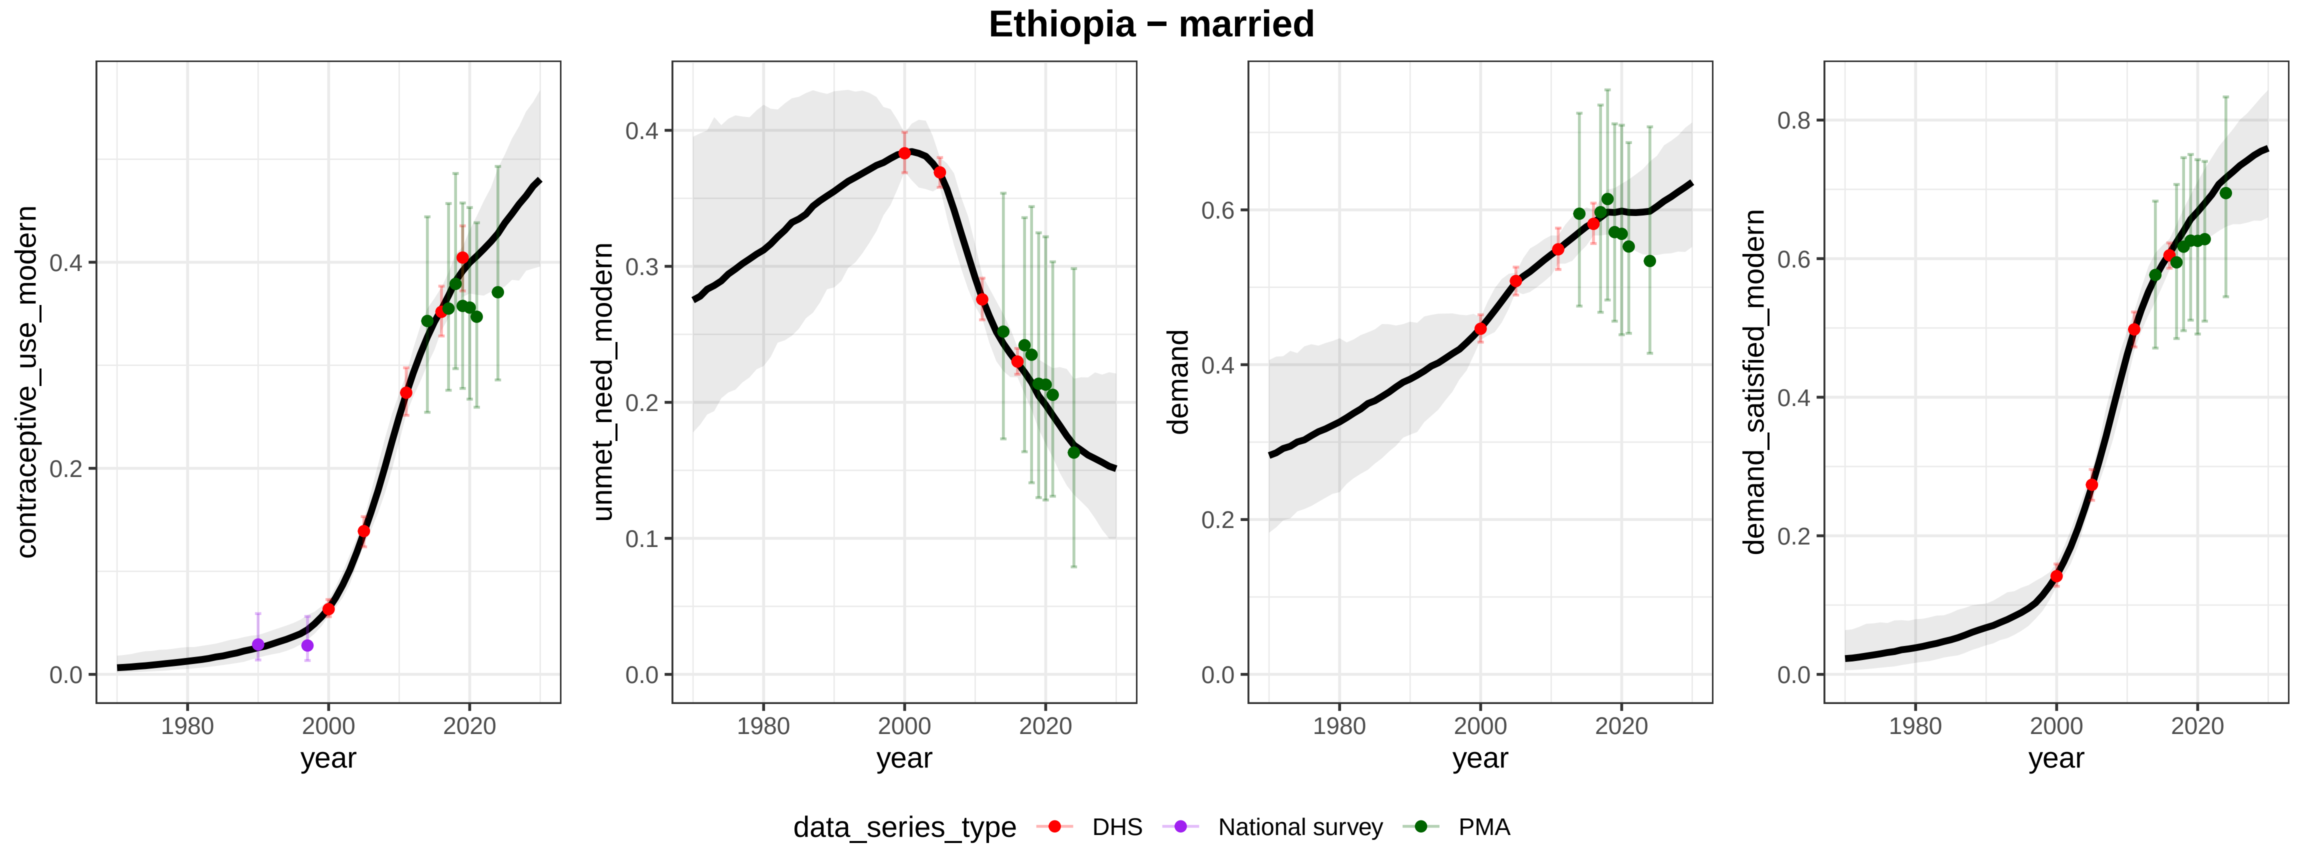

Ethiopia − married
contraceptive_use_modern
unmet_need_modern
demand
demand_satisfied_modern
year
1980
2000
2020
0.0
0.2
0.4
0.6
0.8
0.1
0.3
data_series_type
DHS
National survey
PMA

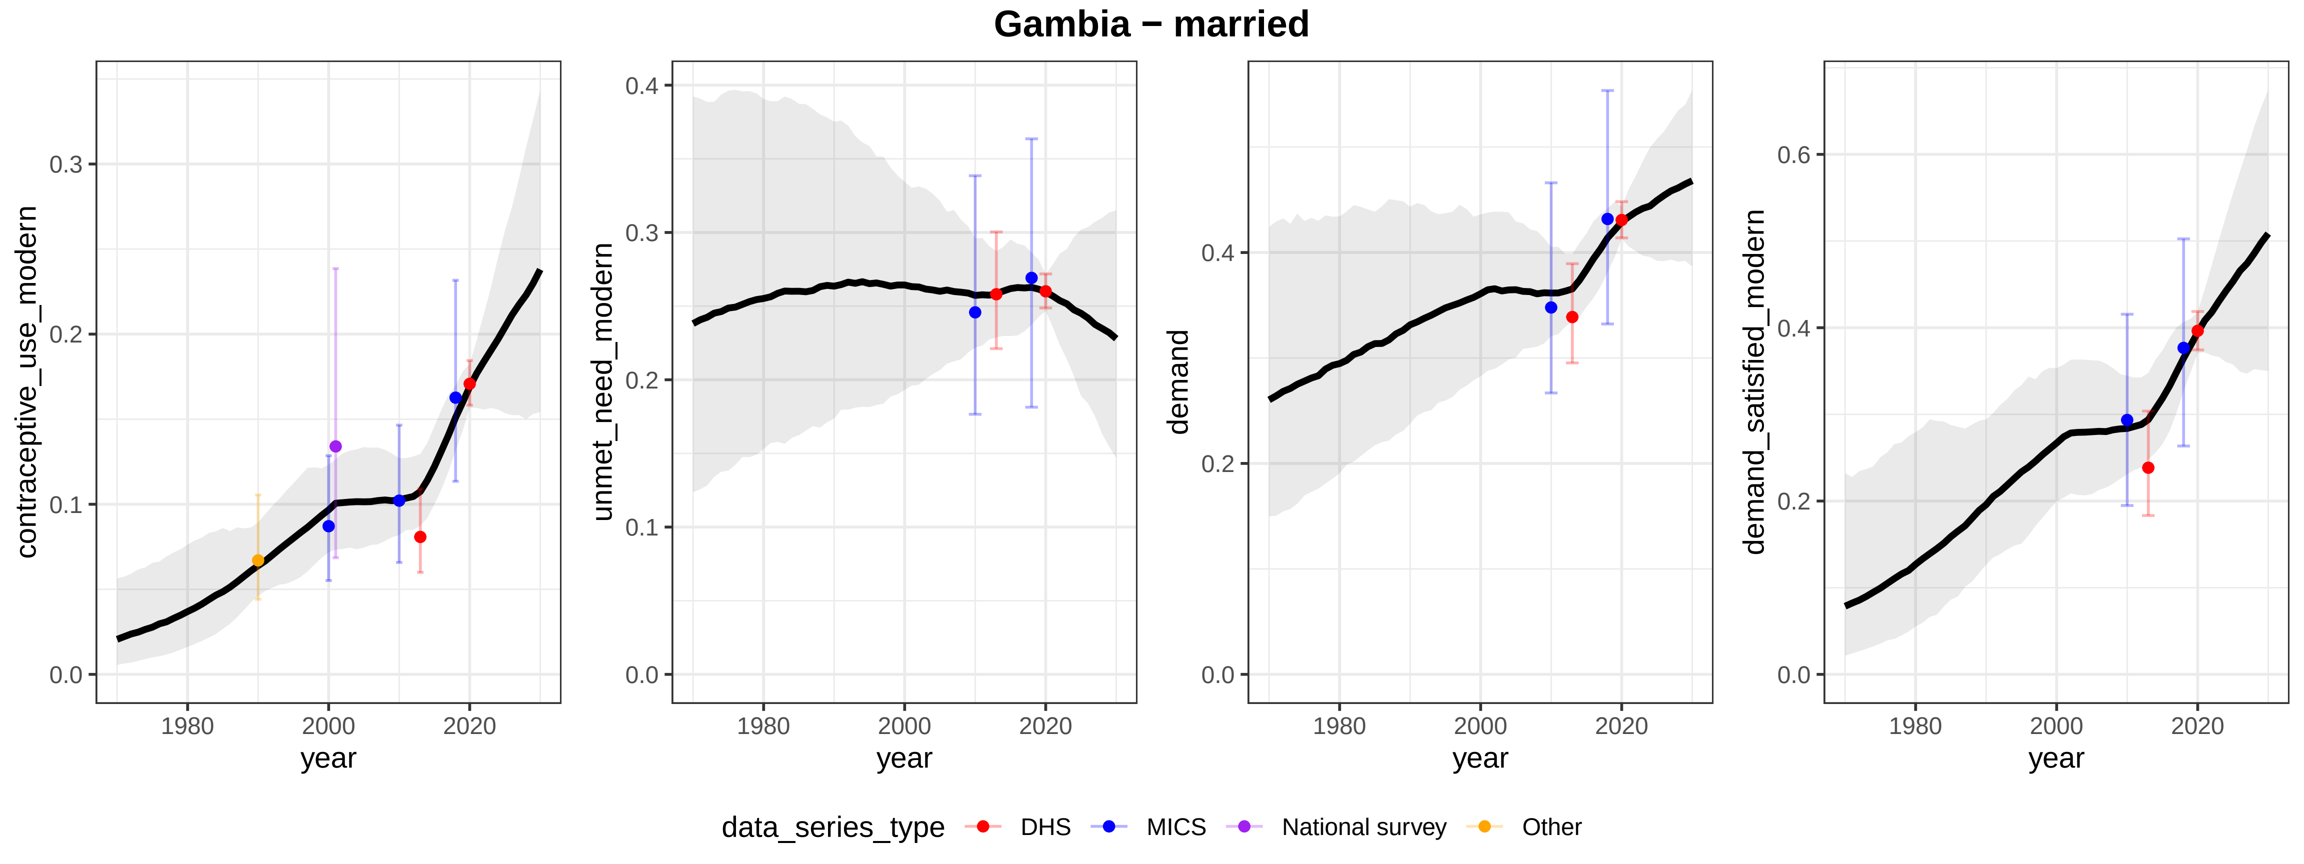

Gambia − married
contraceptive_use_modern
unmet_need_modern
demand
demand_satisfied_modern
year
0.0
0.1
0.2
0.3
0.4
0.6
1980
2000
2020
data_series_type
DHS
MICS
National survey
Other

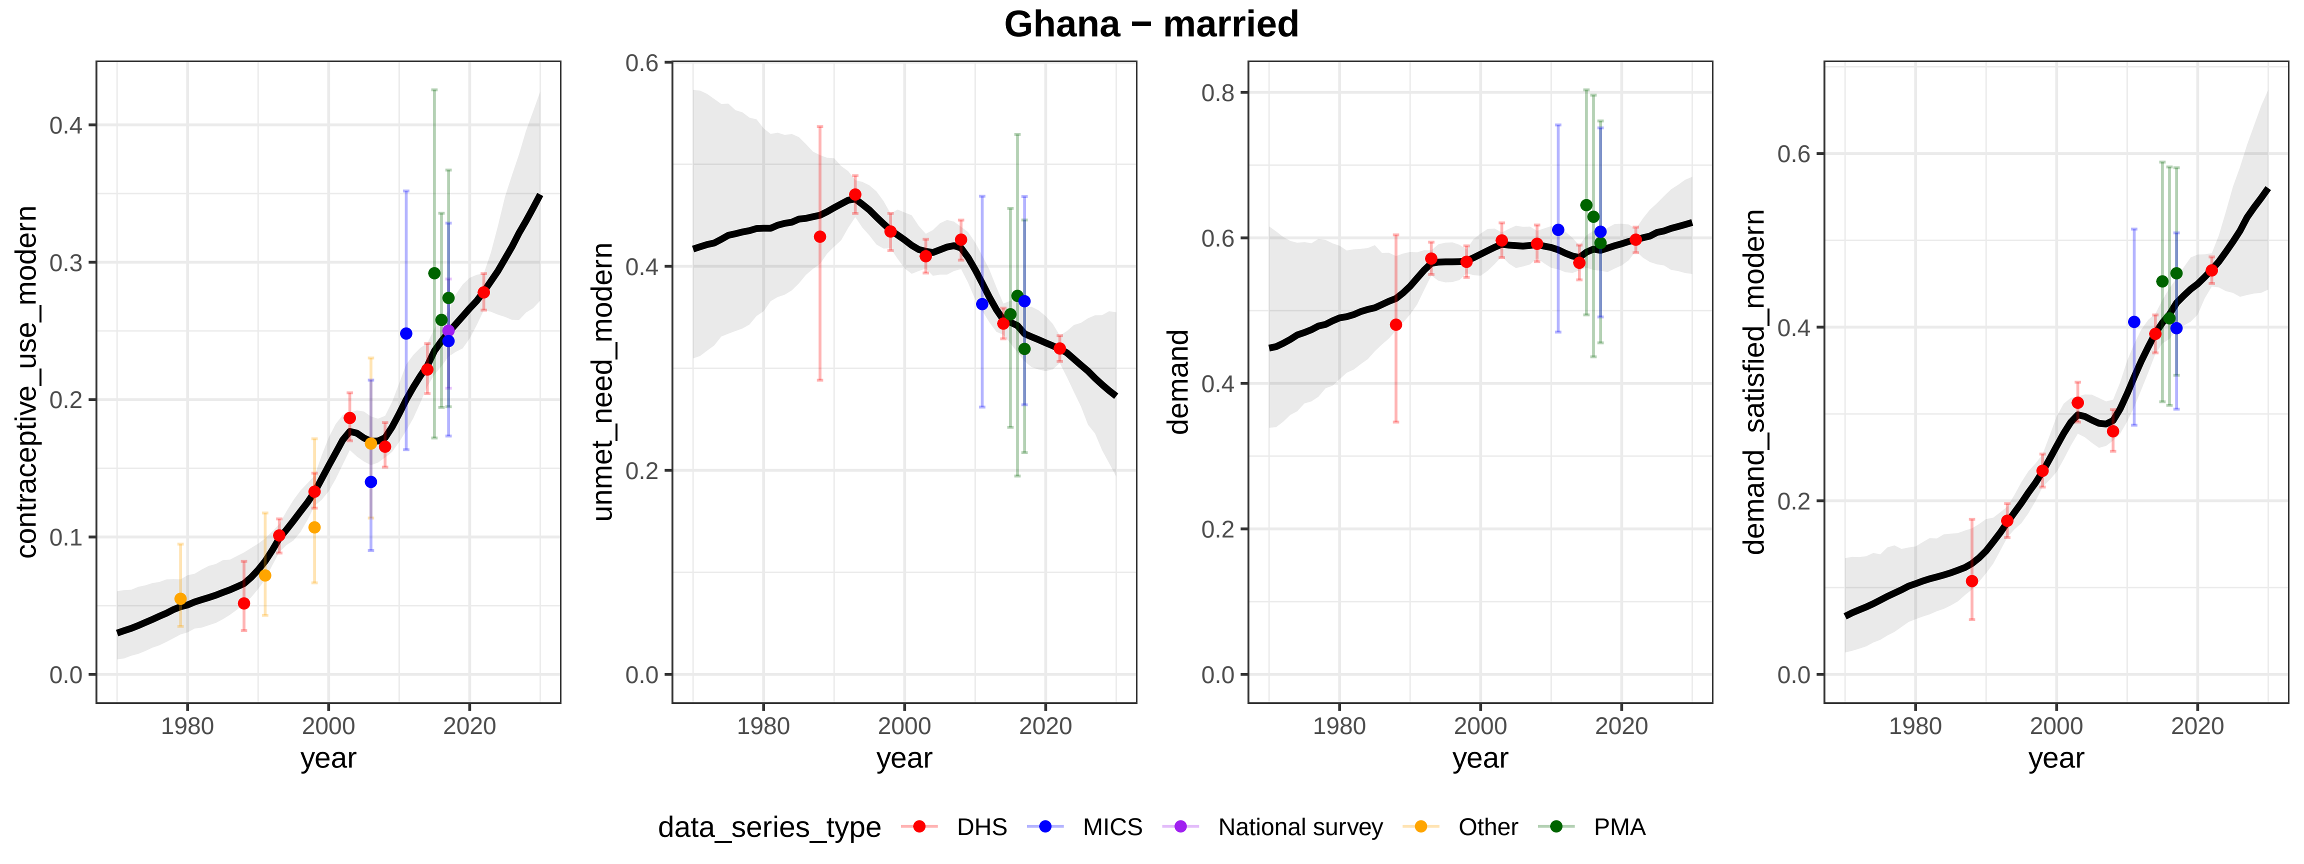

Ghana − married
contraceptive_use_modern
unmet_need_modern
demand
demand_satisfied_modern
year
0.0
0.1
0.2
0.3
0.4
0.6
0.8
1980
2000
2020
data_series_type
DHS
MICS
National survey
Other
PMA

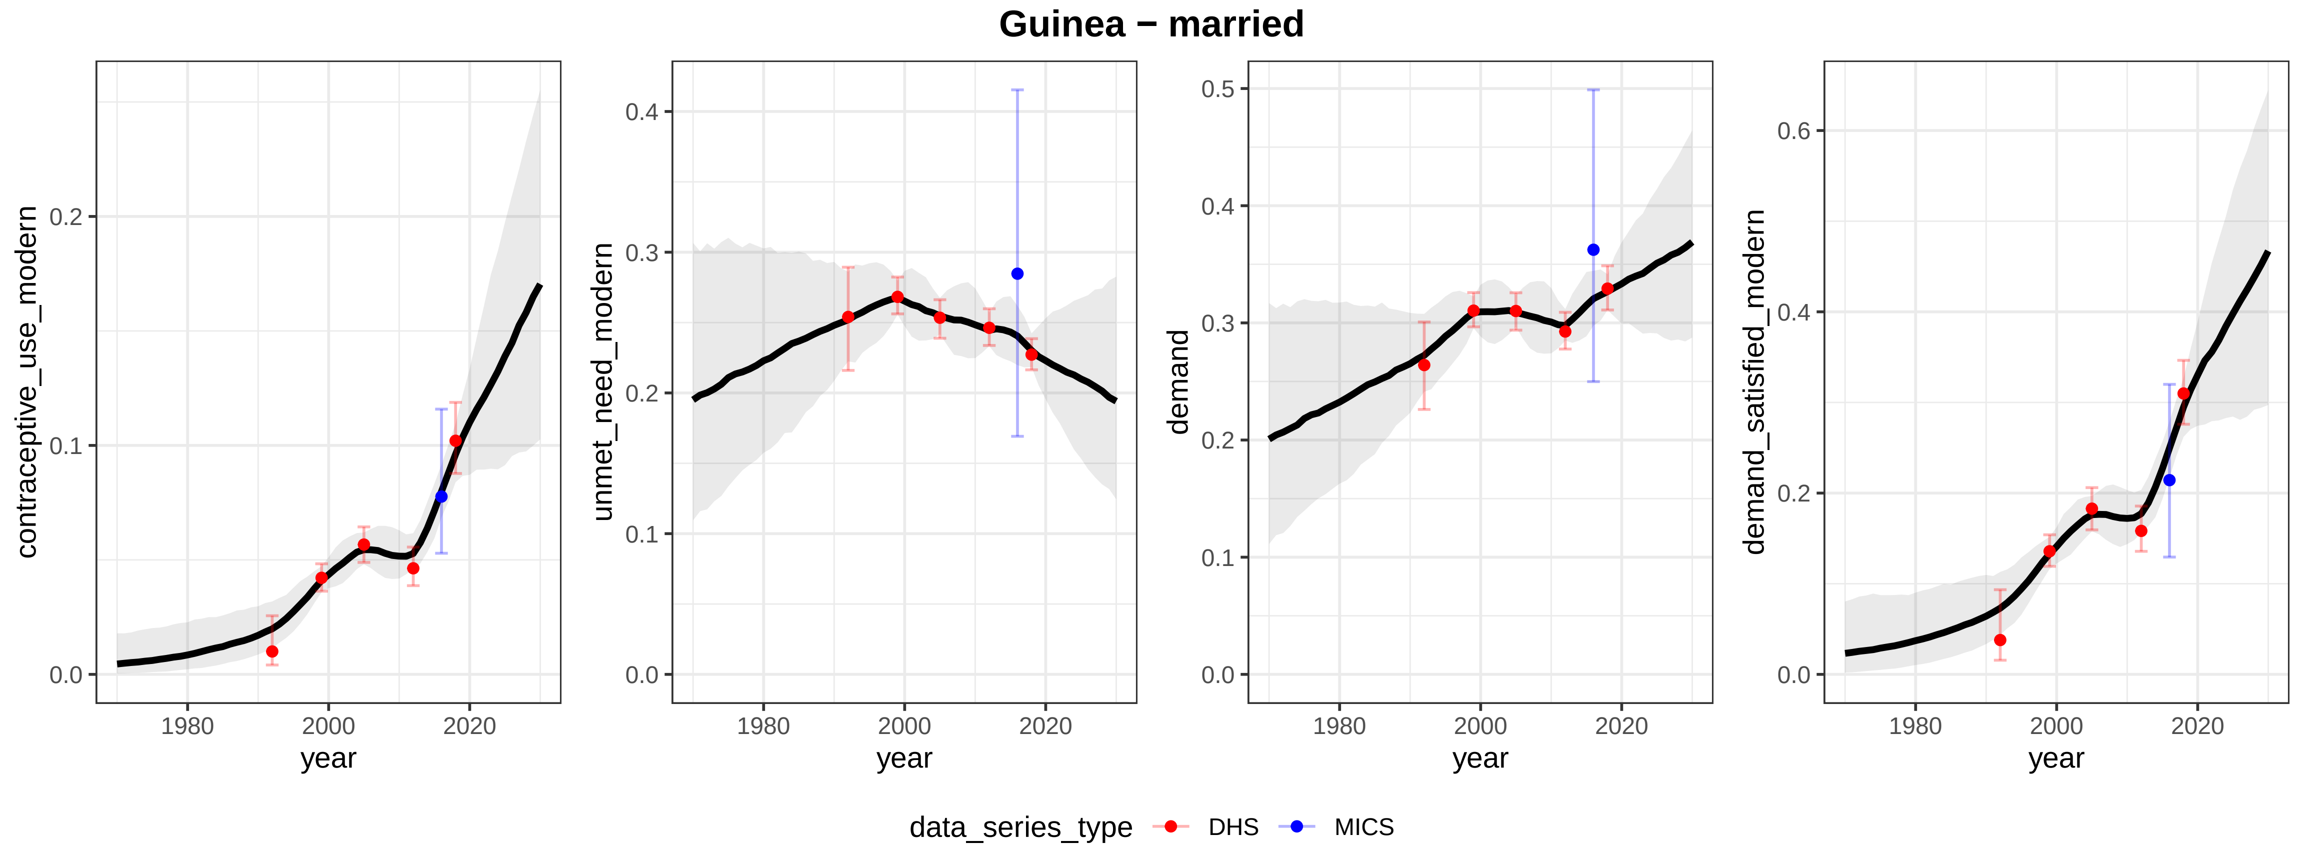

Guinea − married
contraceptive_use_modern
unmet_need_modern
demand
demand_satisfied_modern
year
0.0
0.1
0.2
0.3
0.4
0.5
0.6
1980
2000
2020
data_series_type
DHS
MICS

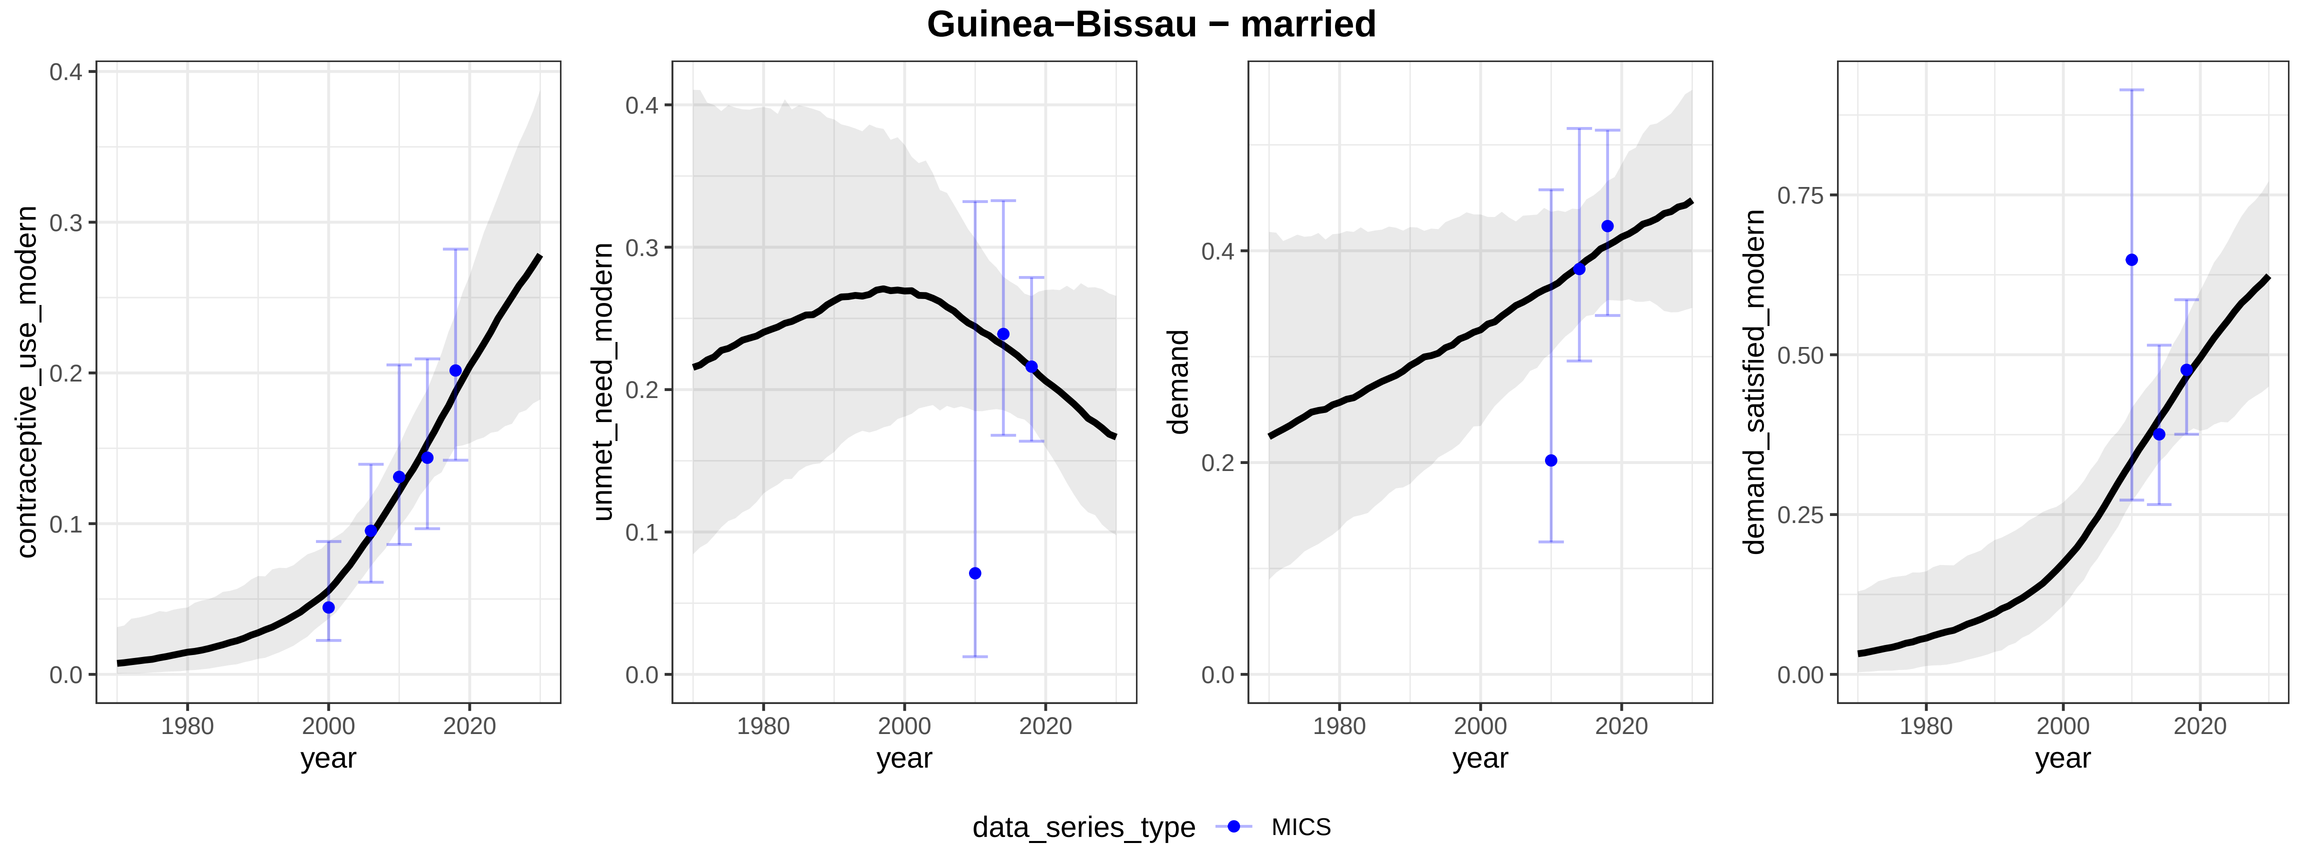
Guinea−Bissau − married
contraceptive_use_modern
unmet_need_modern
demand
demand_satisfied_modern
year
1980
2000
2020
0.0
0.1
0.2
0.3
0.4
0.00
0.25
0.50
0.75
data_series_type
MICS

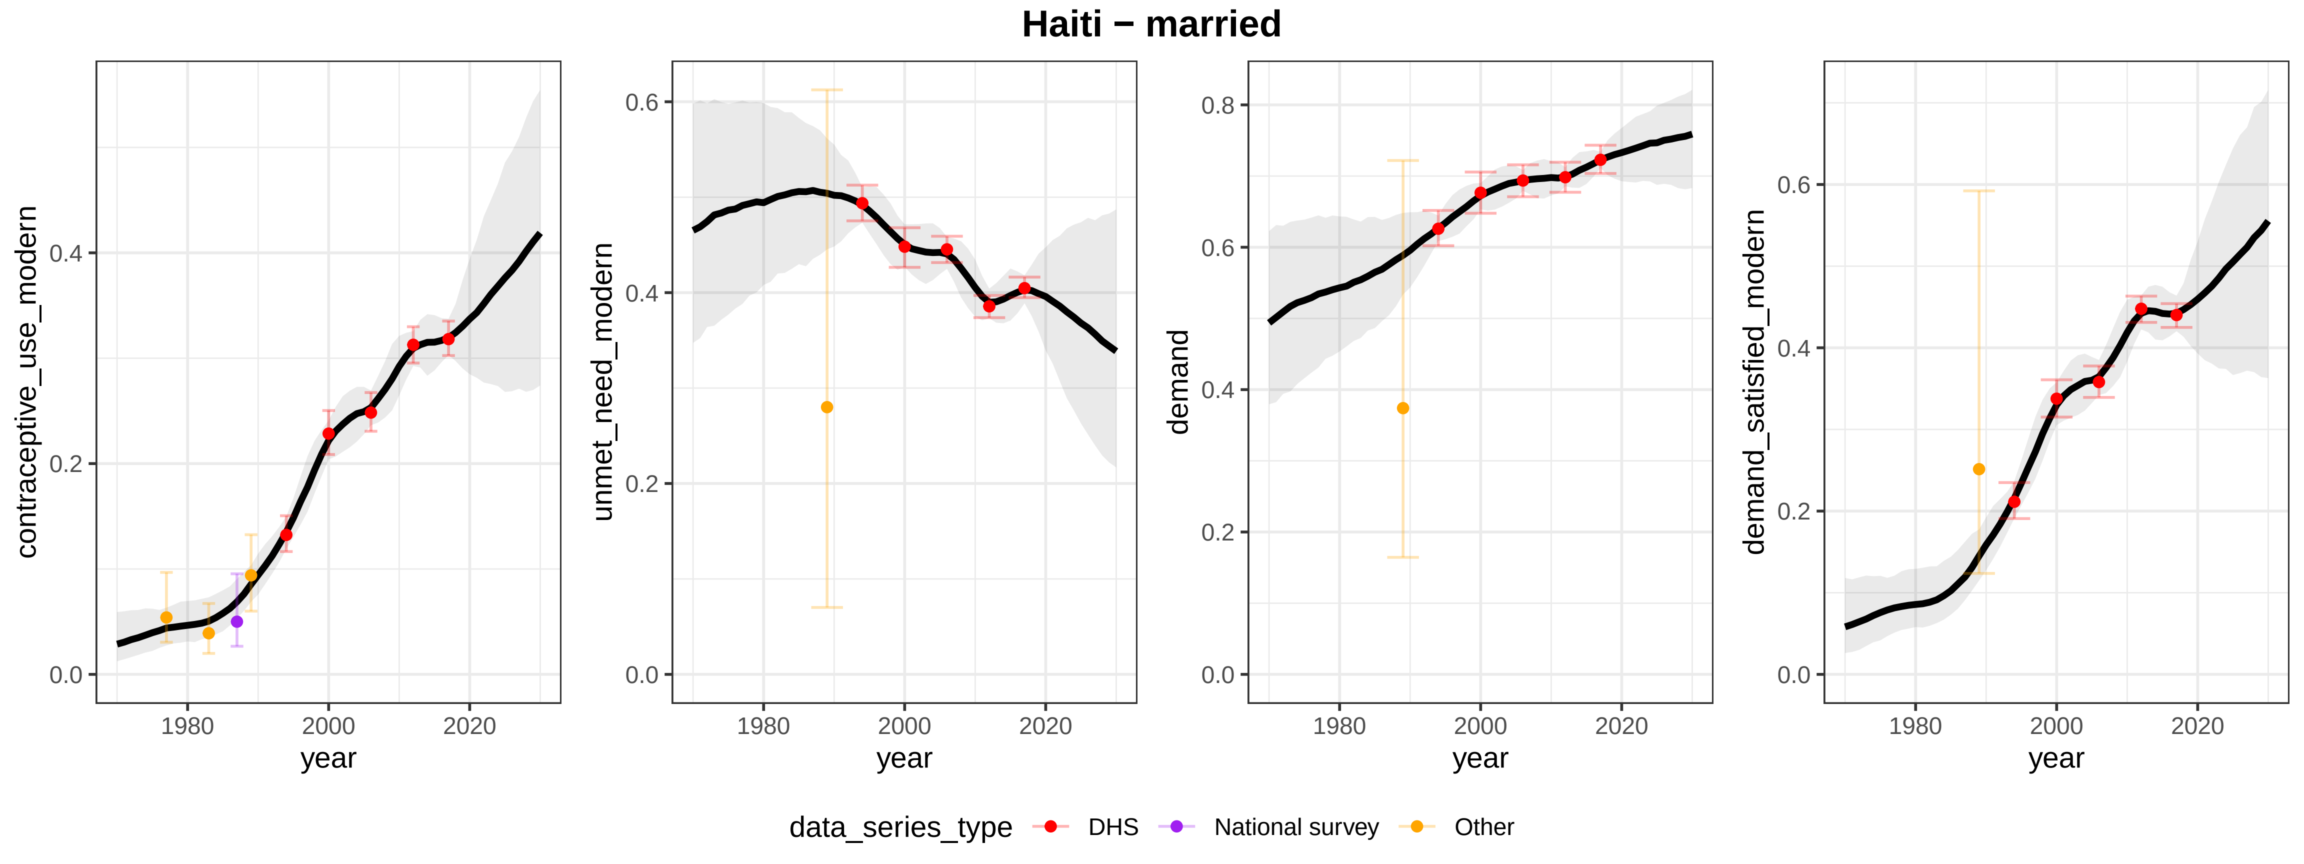

Haiti − married
contraceptive_use_modern
unmet_need_modern
demand
demand_satisfied_modern
year
0.0
0.2
0.4
0.6
0.8
1980
2000
2020
data_series_type
DHS
National survey
Other

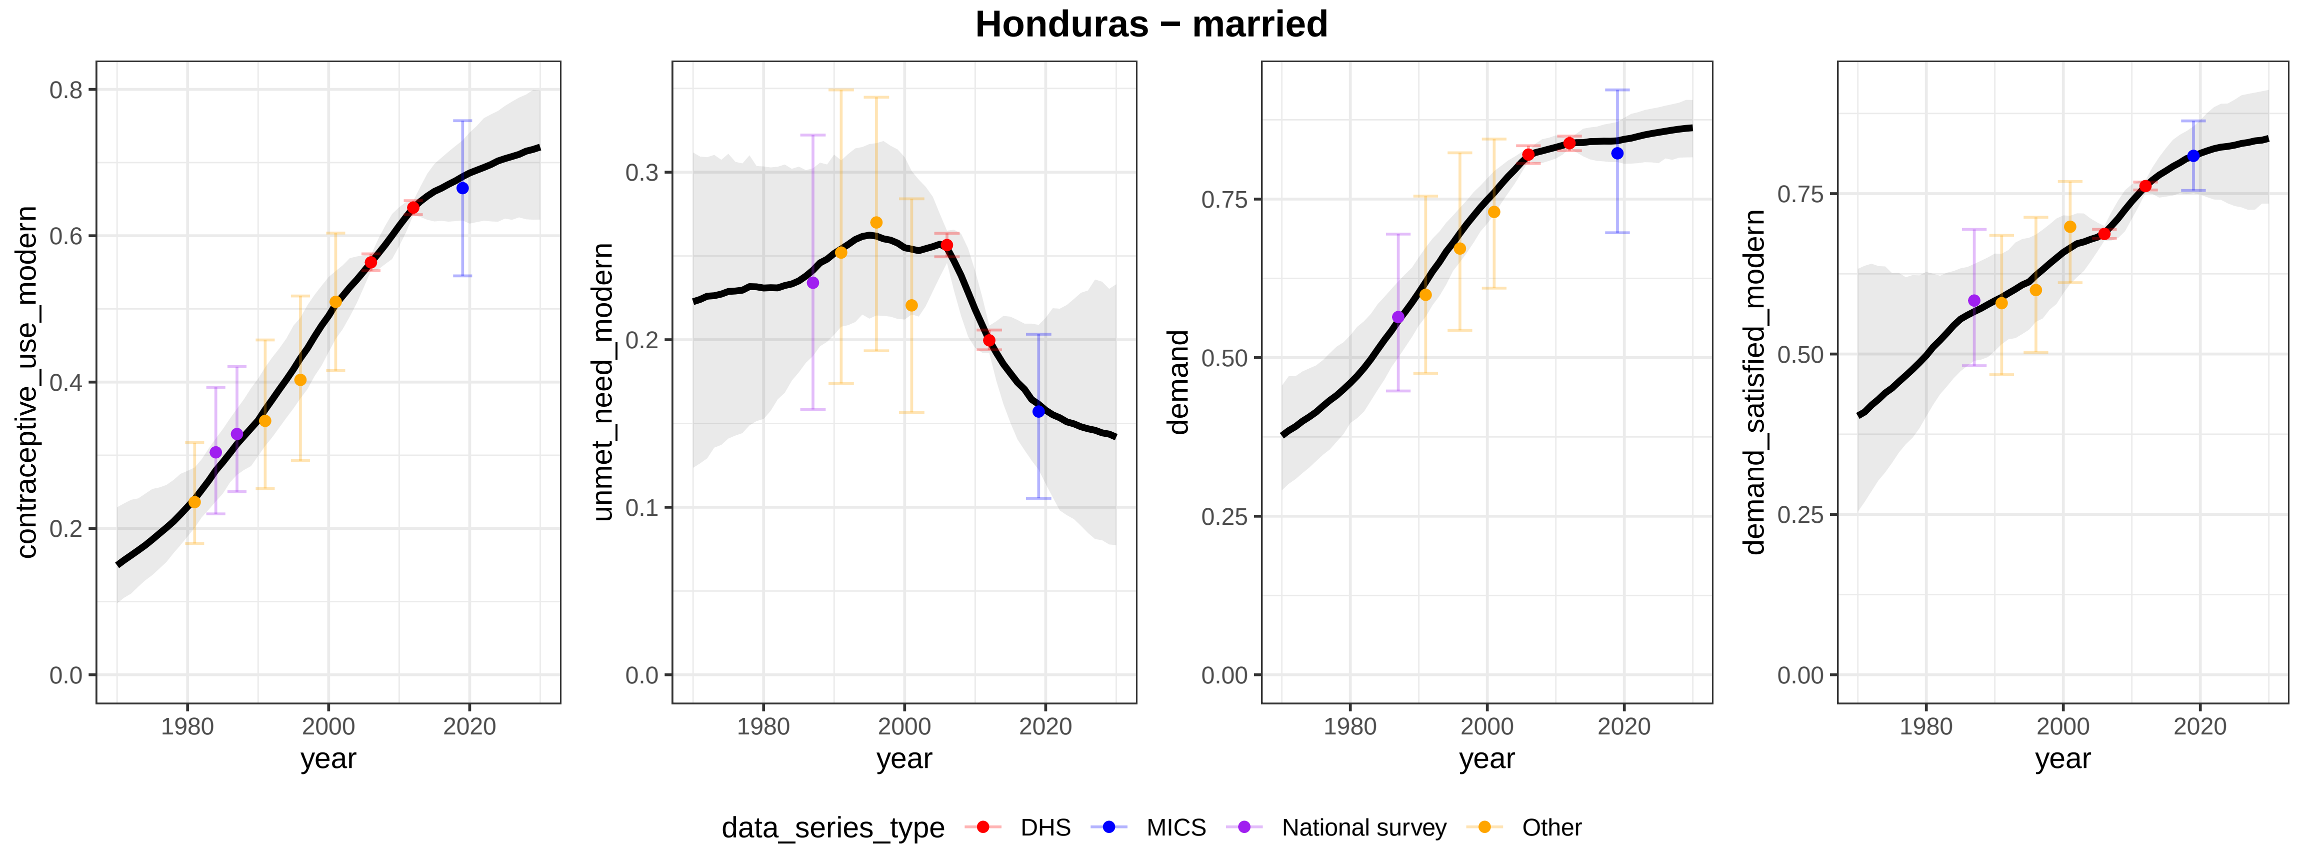

Honduras − married
contraceptive_use_modern
unmet_need_modern
demand
demand_satisfied_modern
year
1980
2000
2020
0.0
0.2
0.4
0.6
0.8
0.1
0.3
0.00
0.25
0.50
0.75
data_series_type
DHS
MICS
National survey
Other

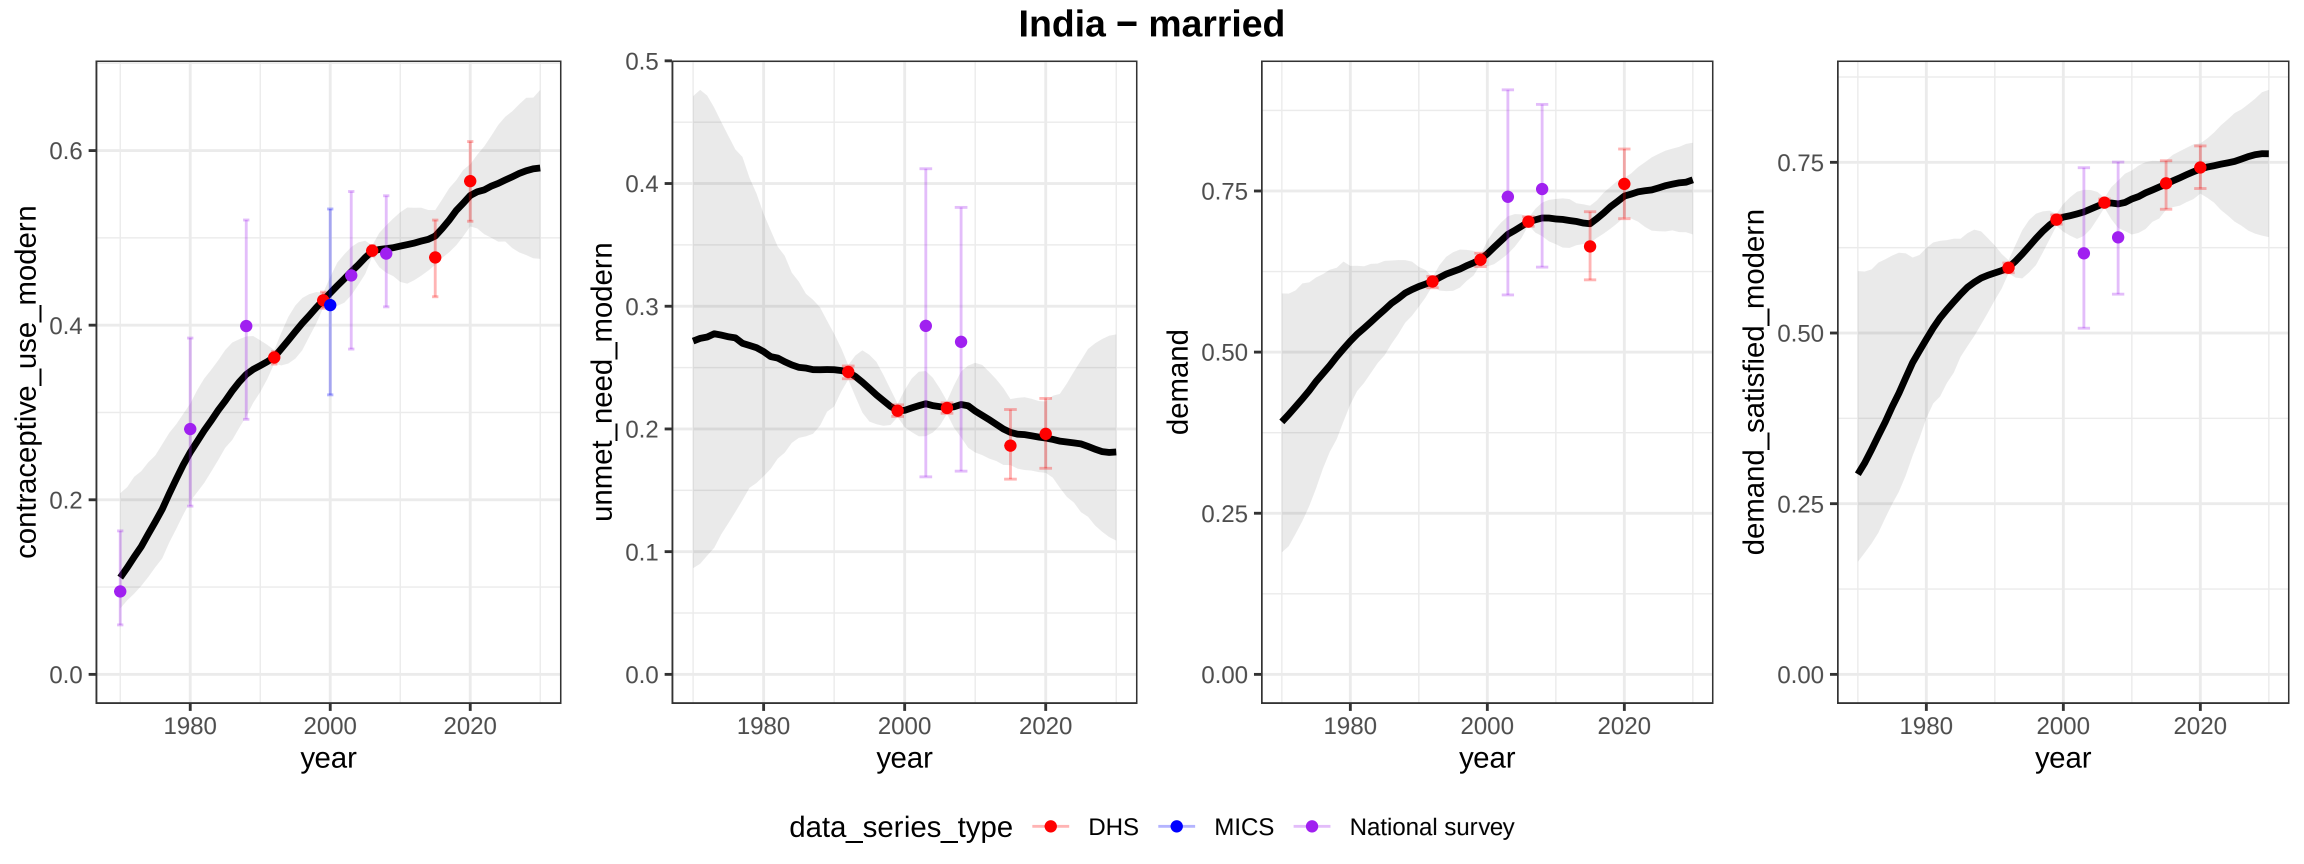
India − married
contraceptive_use_modern
unmet_need_modern
demand
demand_satisfied_modern
year
0.0
0.2
0.4
0.6
0.1
0.3
0.5
0.00
0.25
0.50
0.75
1980
2000
2020
data_series_type
DHS
MICS
National survey

# Indonesia − married

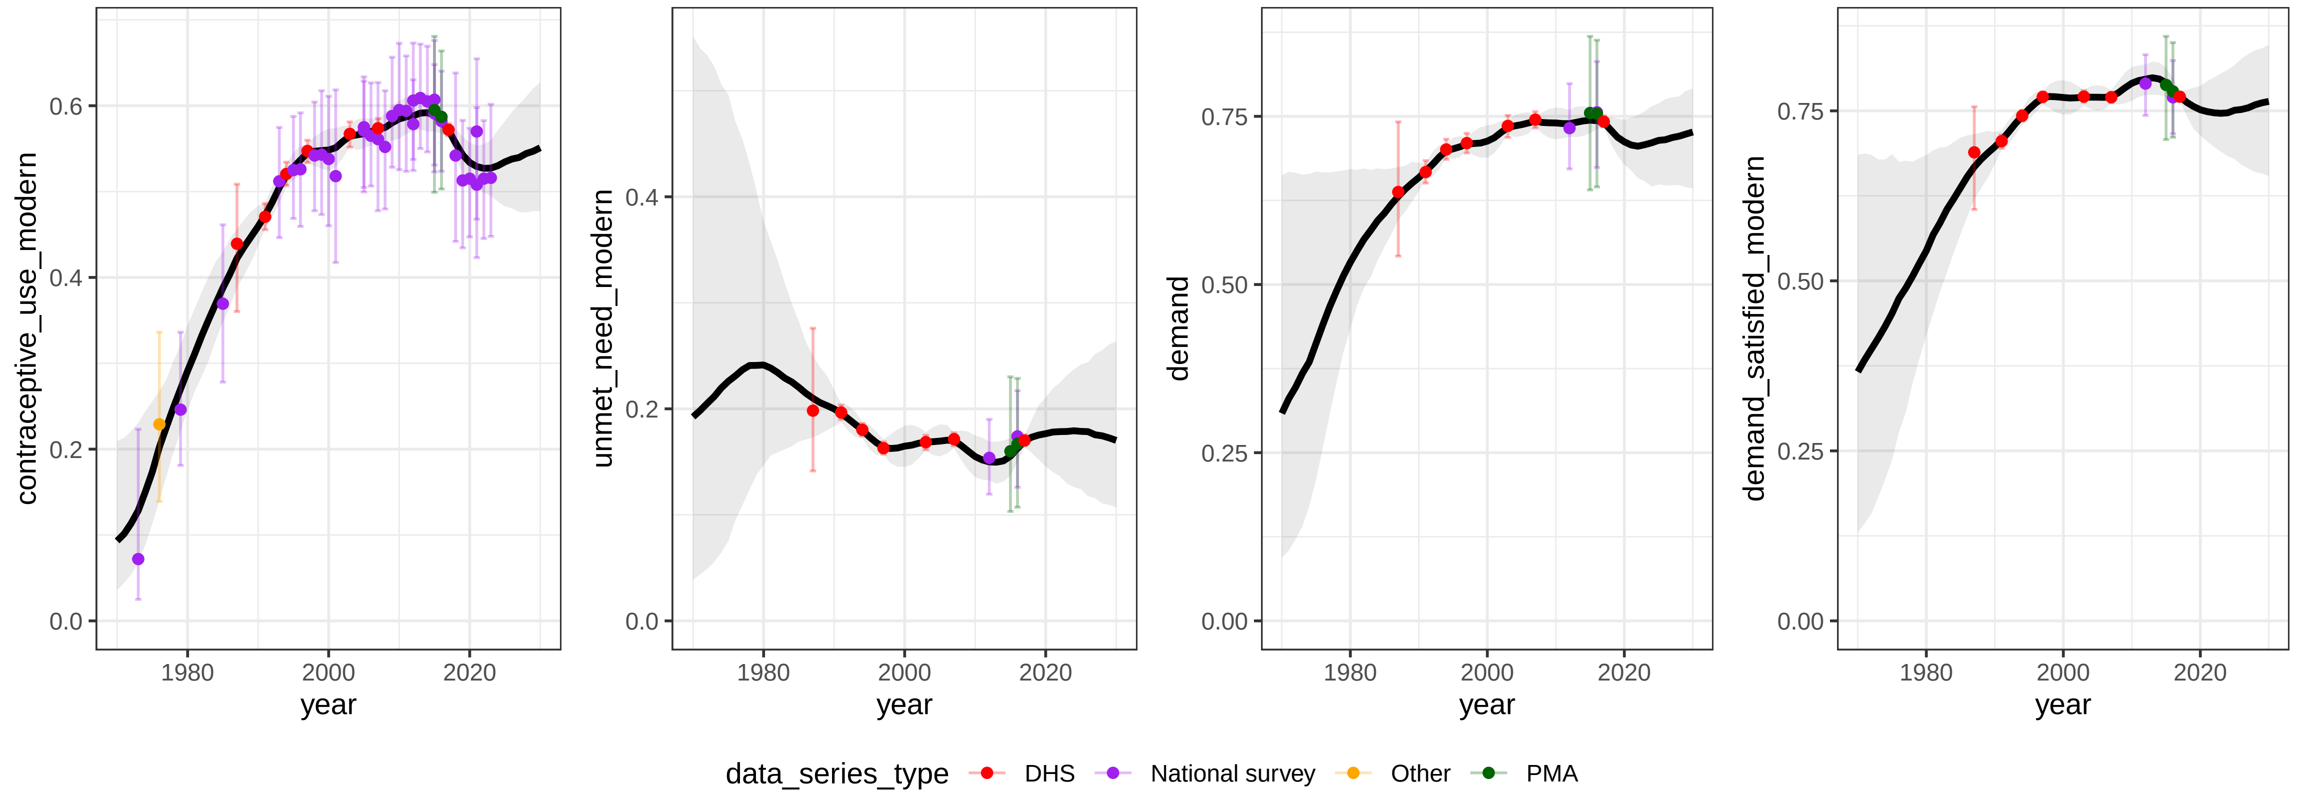

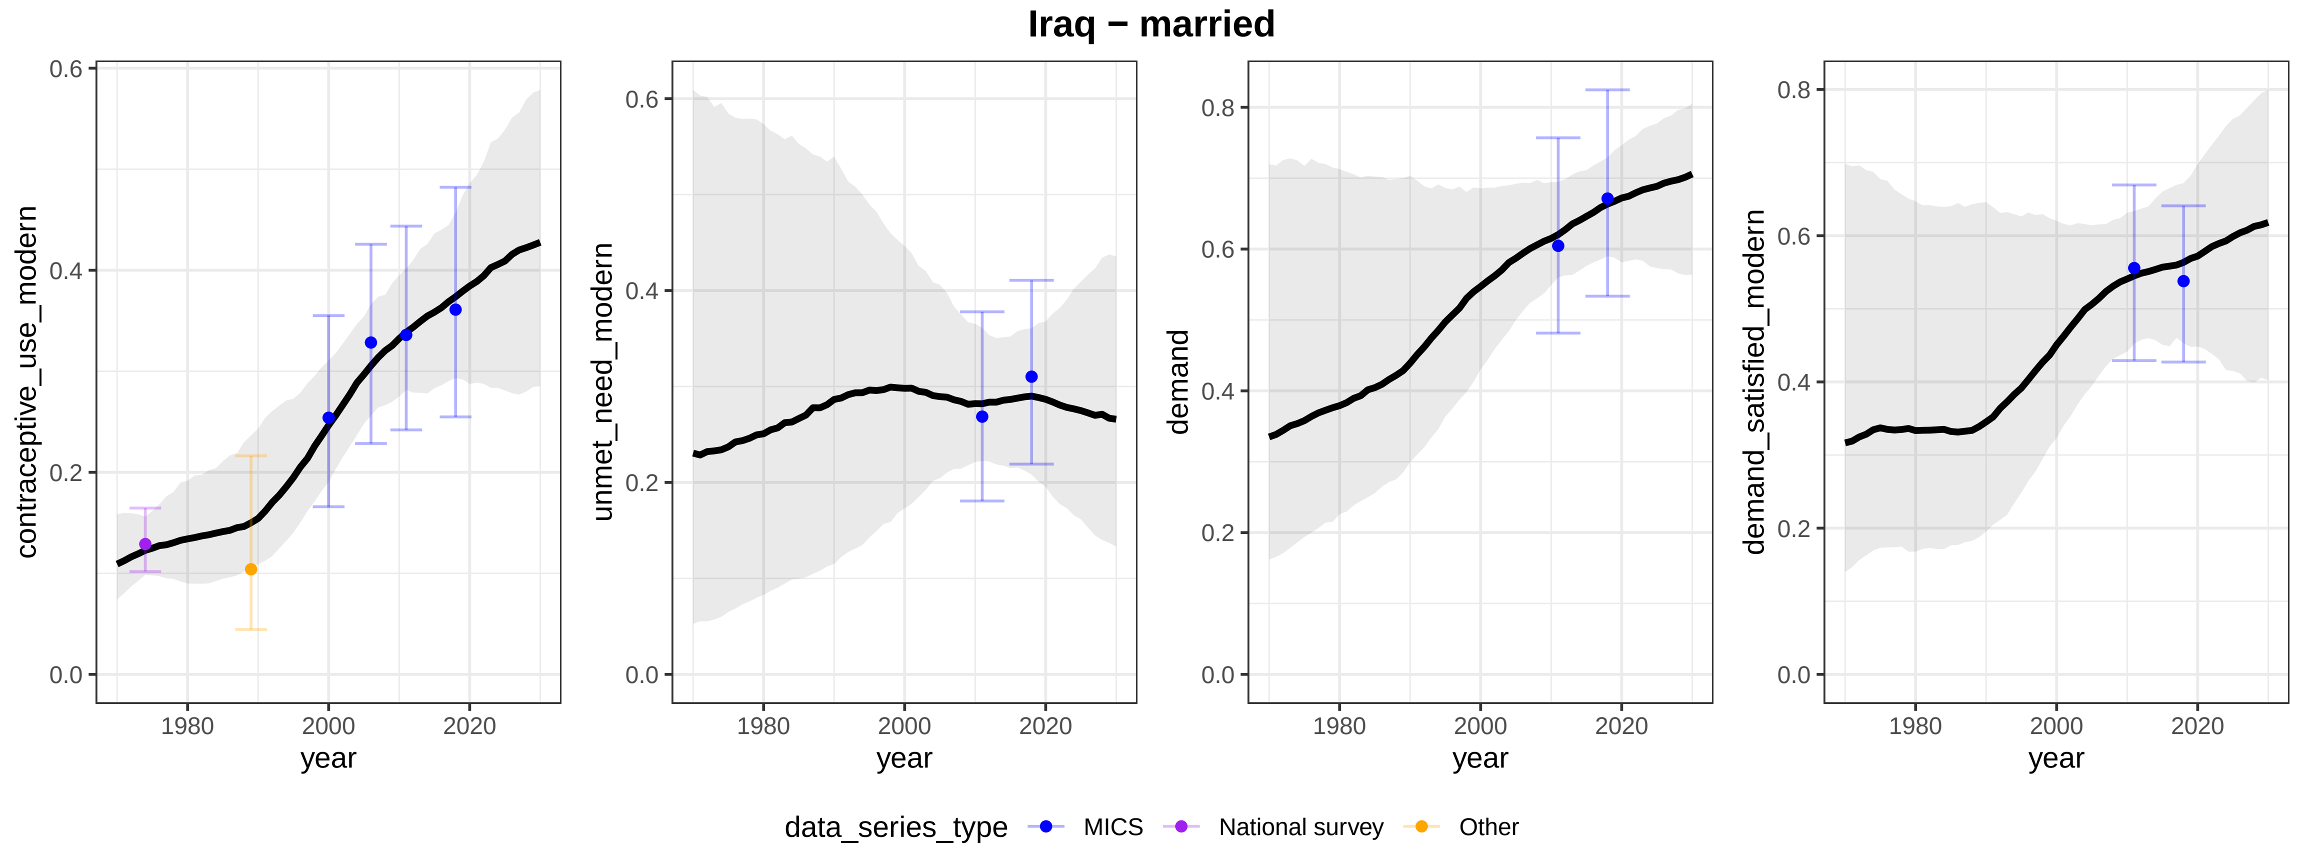

Iraq − married
contraceptive_use_modern
unmet_need_modern
demand
demand_satisfied_modern
0.0
0.2
0.4
0.6
0.8
1980
2000
2020
year
data_series_type
MICS
National survey
Other

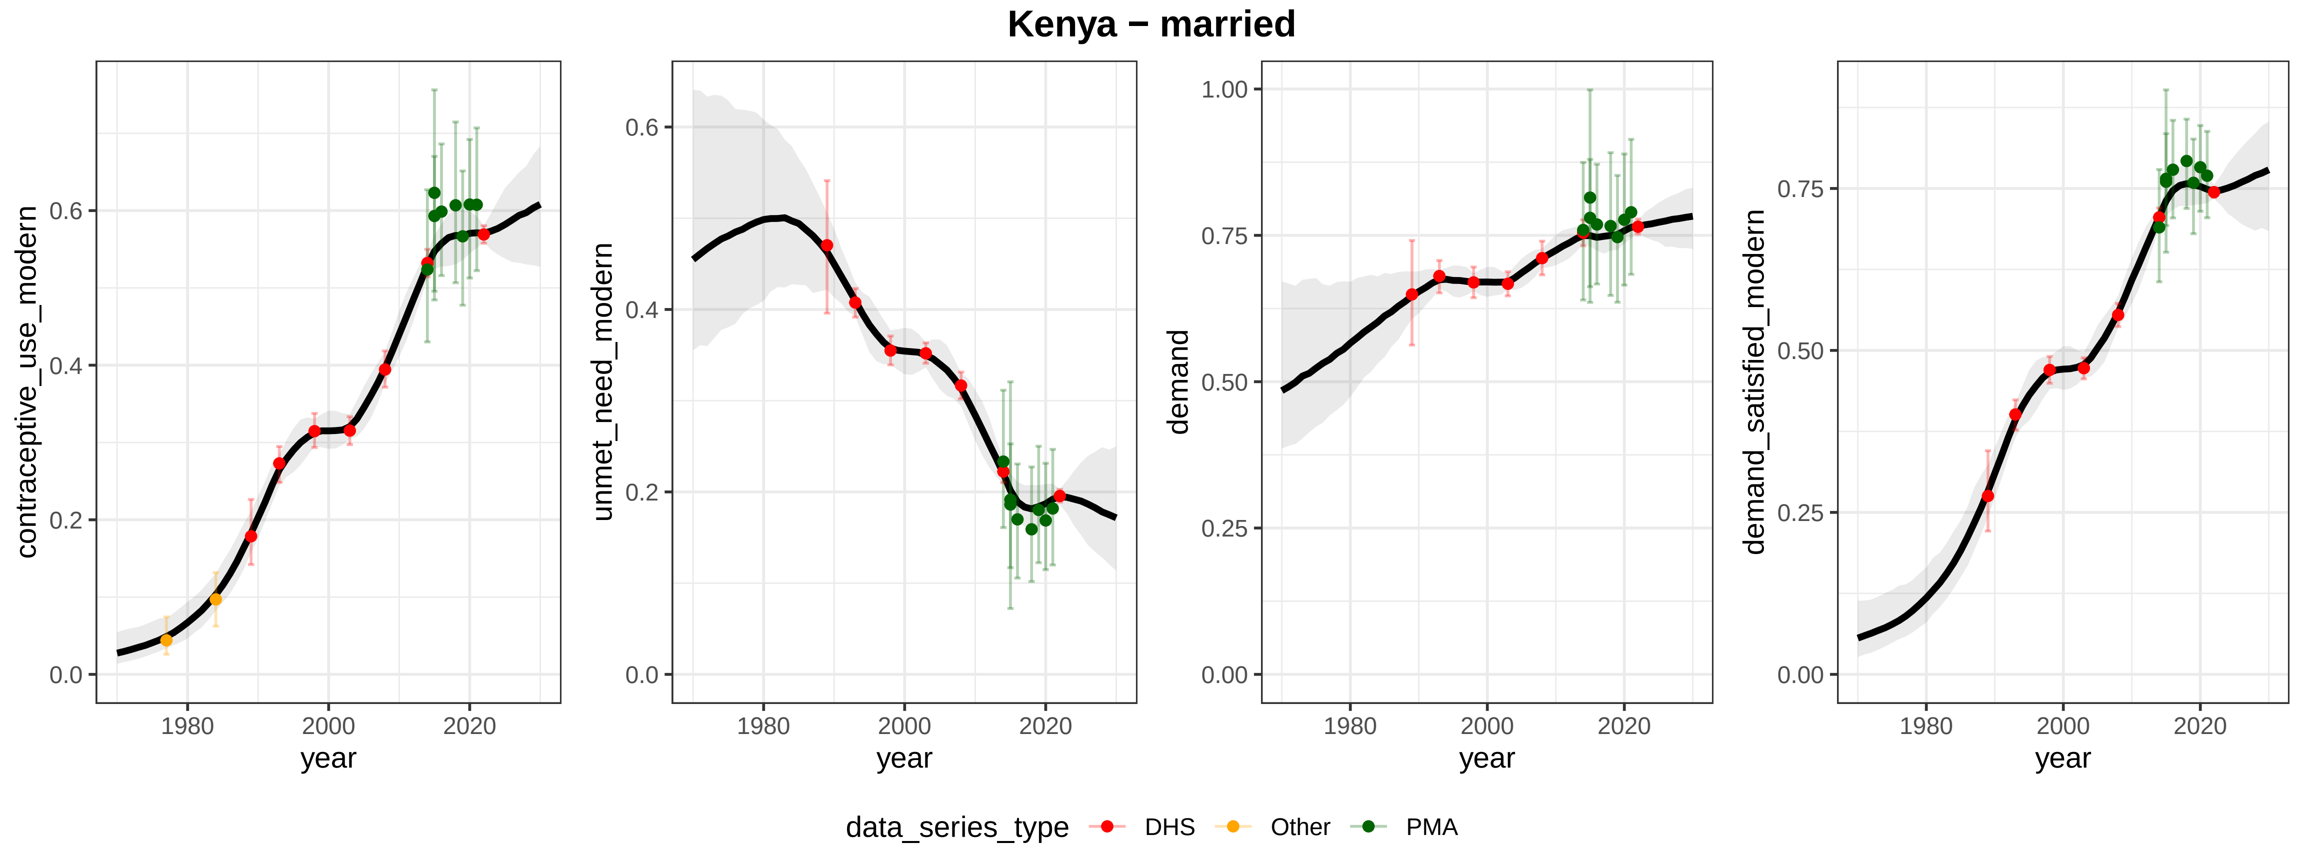
Kenya − married
contraceptive_use_modern
unmet_need_modern
demand
demand_satisfied_modern
year
1980
2000
2020
0.0
0.2
0.4
0.6
0.00
0.25
0.50
0.75
1.00
data_series_type
DHS
Other
PMA

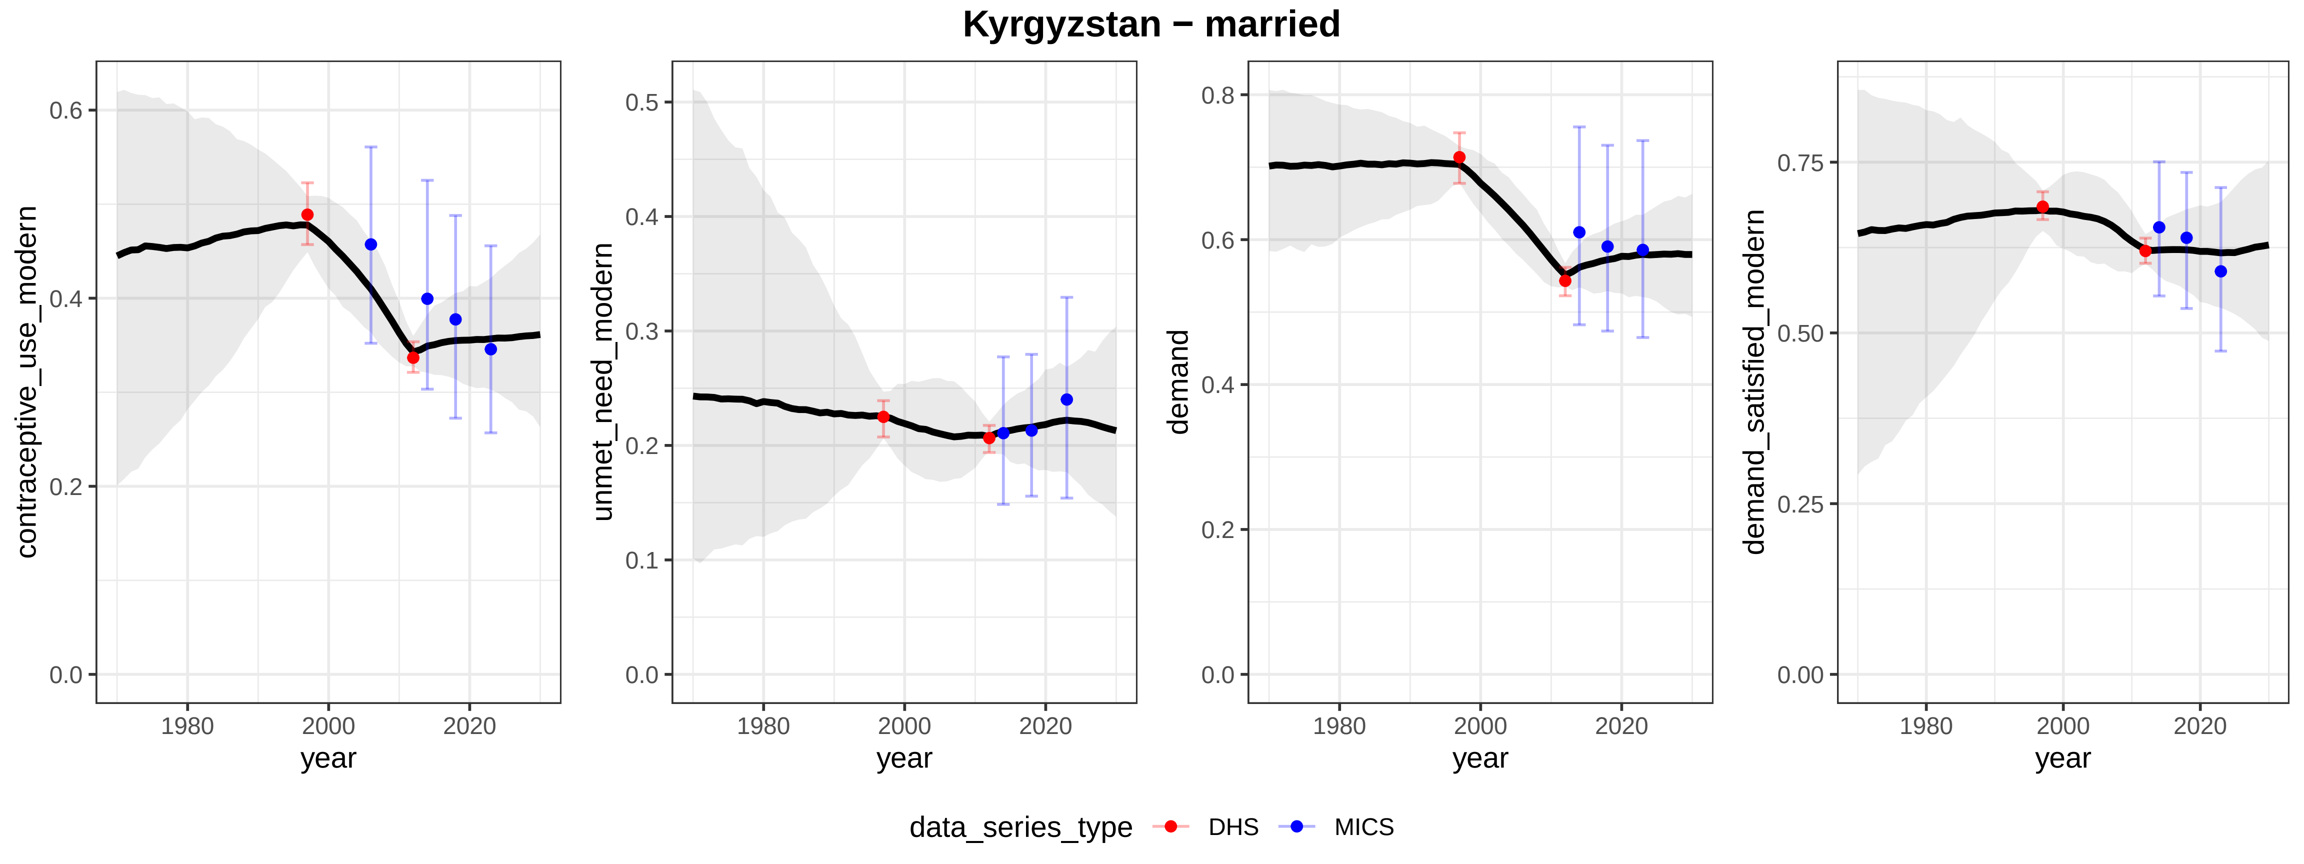

Kyrgyzstan − married
contraceptive_use_modern
unmet_need_modern
demand
demand_satisfied_modern
0.0
0.2
0.4
0.6
0.1
0.3
0.5
0.8
0.00
0.25
0.50
0.75
1980
2000
2020
year
data_series_type
DHS
MICS

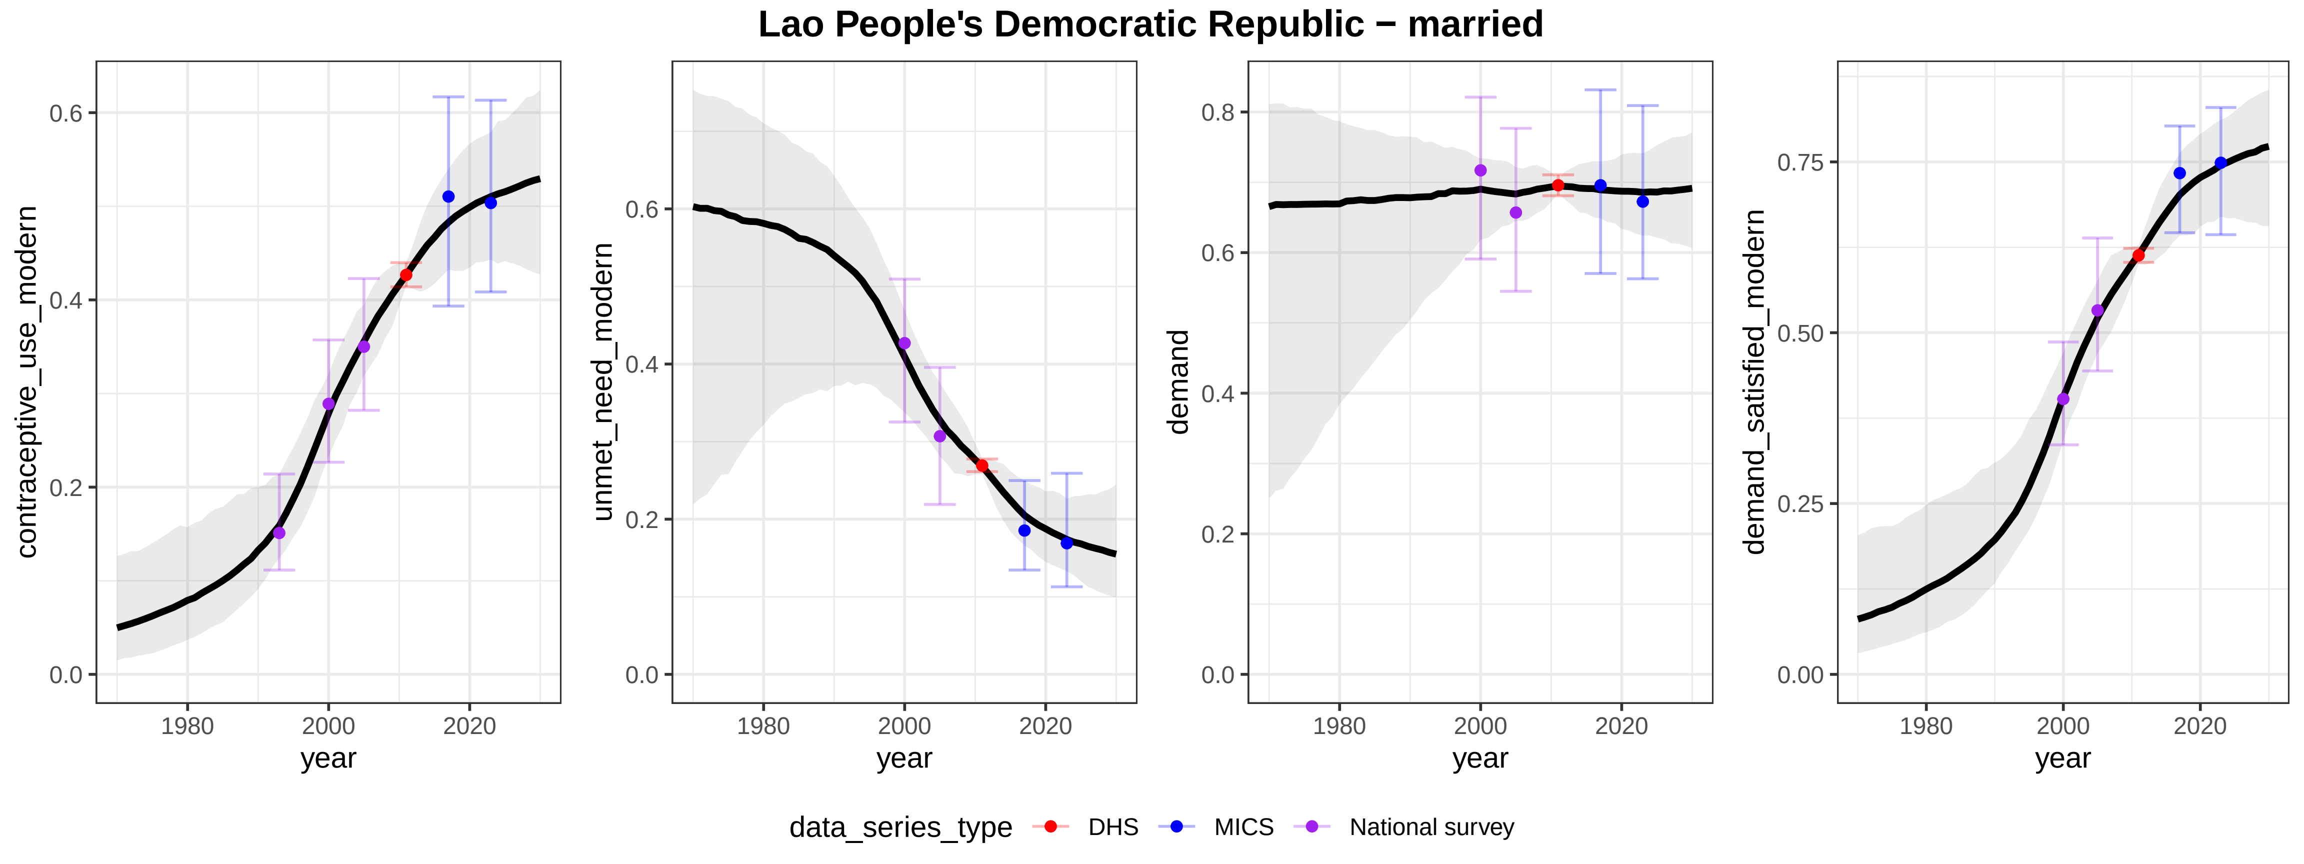

Lao People's Democratic Republic − married
contraceptive_use_modern
unmet_need_modern
demand
demand_satisfied_modern
0.0
0.2
0.4
0.6
0.8
0.00
0.25
0.50
0.75
1980
2000
2020
year
data_series_type
DHS
MICS
National survey

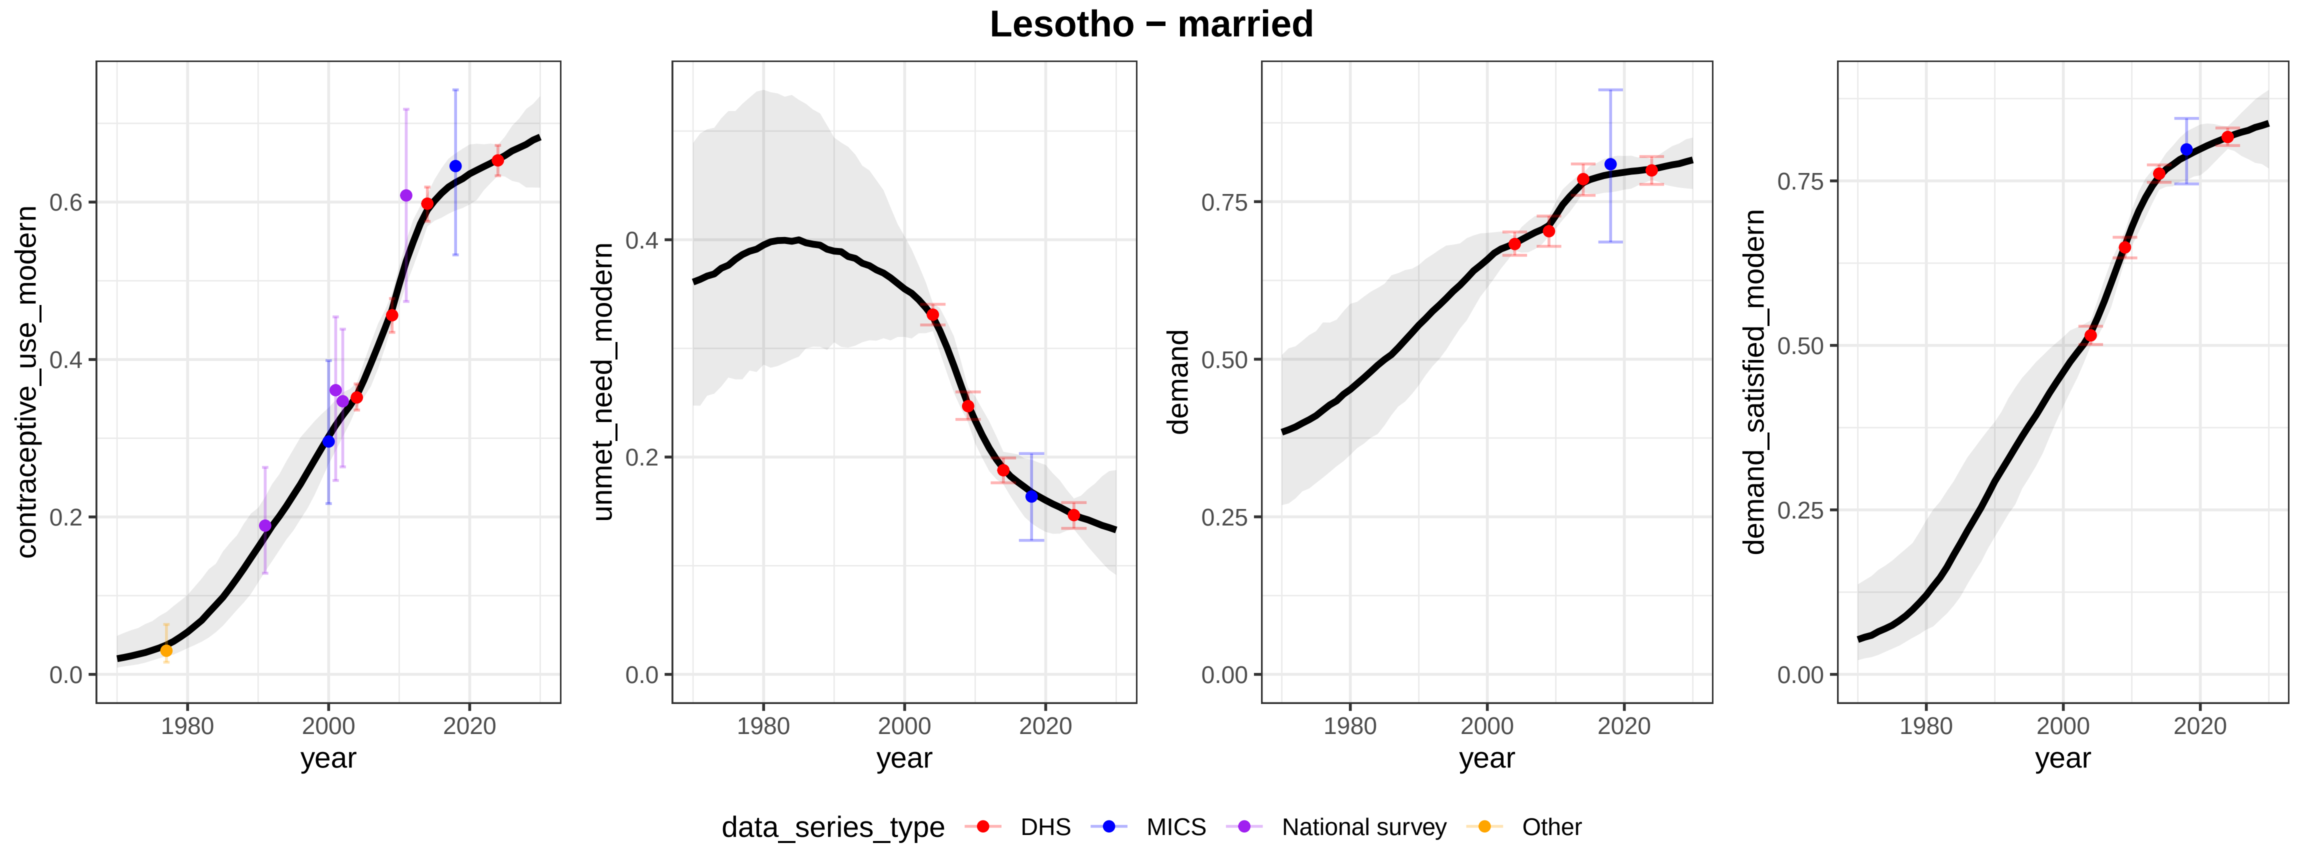

Lesotho − married
contraceptive_use_modern
unmet_need_modern
demand
demand_satisfied_modern
year
0.0
0.2
0.4
0.6
0.00
0.25
0.50
0.75
1980
2000
2020
data_series_type
DHS
MICS
National survey
Other

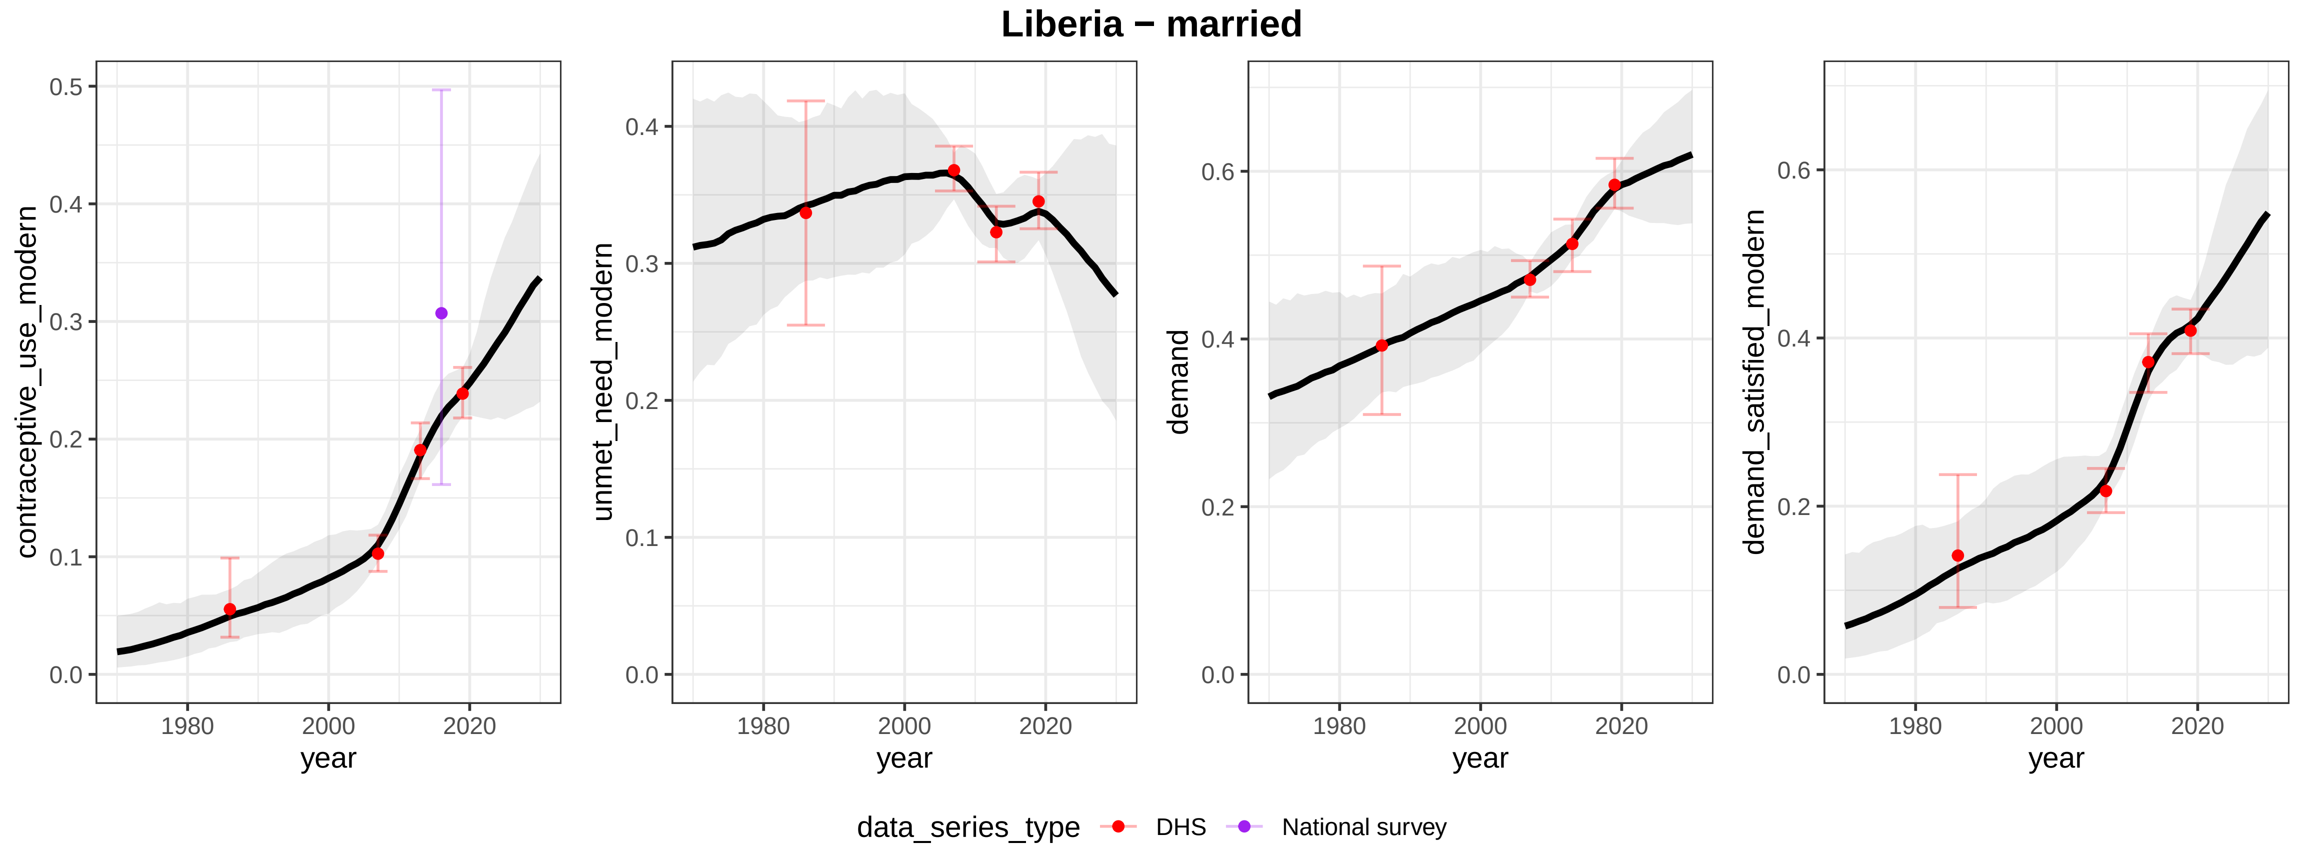

Liberia − married
contraceptive_use_modern
unmet_need_modern
demand
demand_satisfied_modern
year
1980
2000
2020
0.0
0.1
0.2
0.3
0.4
0.5
0.6
data_series_type
DHS
National survey

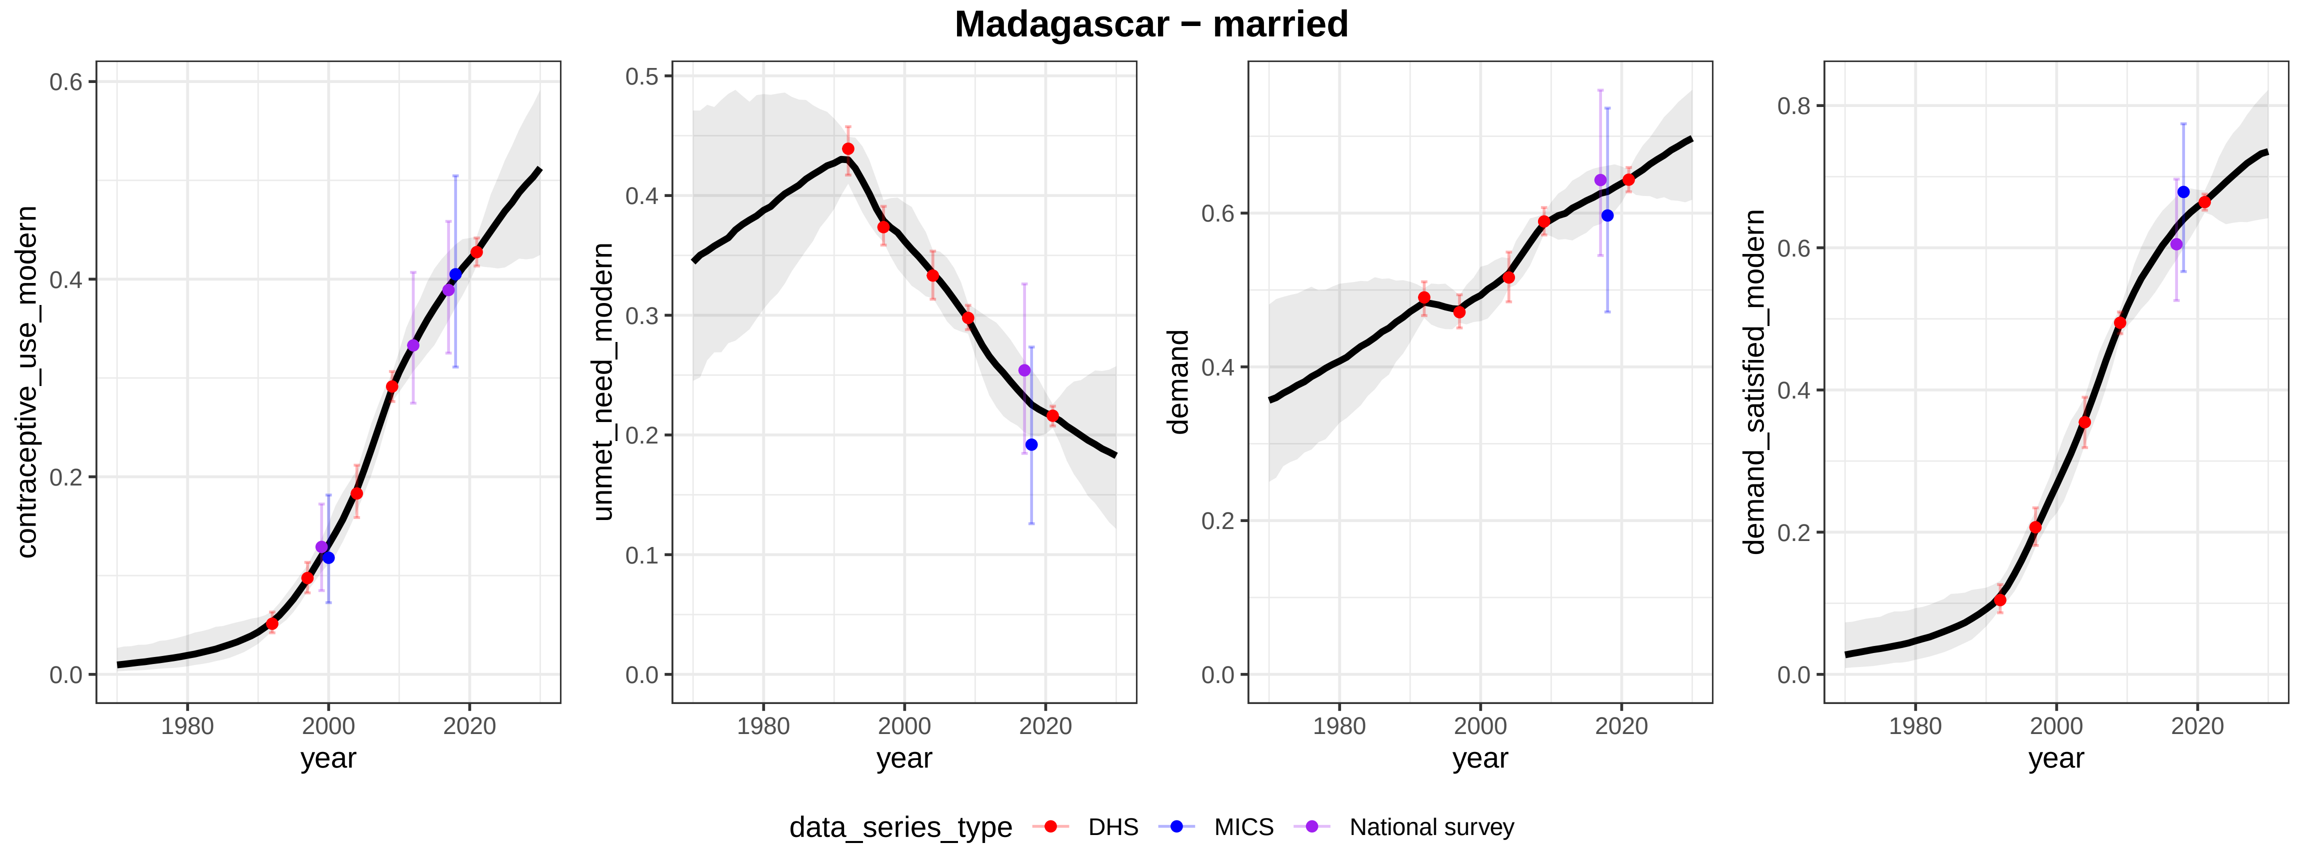

Madagascar − married
contraceptive_use_modern
unmet_need_modern
demand
demand_satisfied_modern
year
1980
2000
2020
0.0
0.2
0.4
0.6
0.1
0.3
0.5
0.8
data_series_type
DHS
MICS
National survey

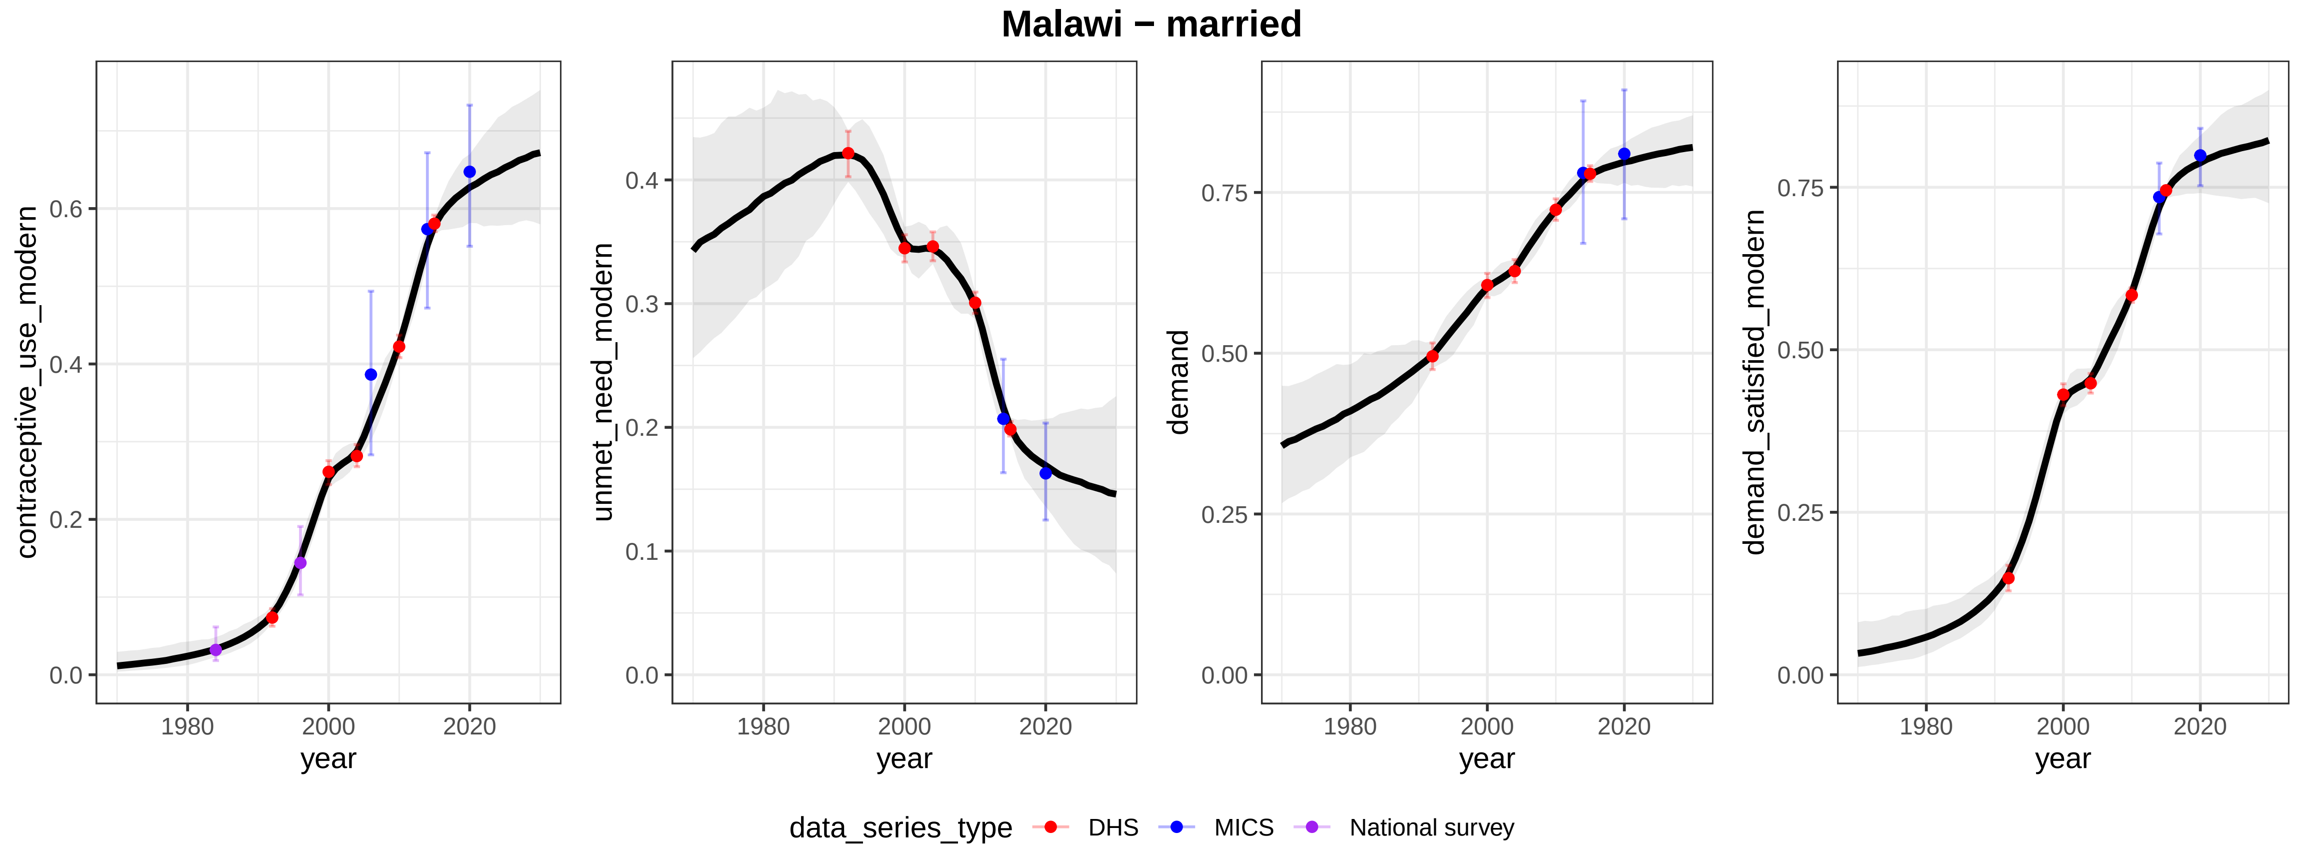

Malawi − married
contraceptive_use_modern
unmet_need_modern
demand
demand_satisfied_modern
year
1980
2000
2020
0.0
0.2
0.4
0.6
0.1
0.3
0.00
0.25
0.50
0.75
data_series_type
DHS
MICS
National survey

# Mali − married

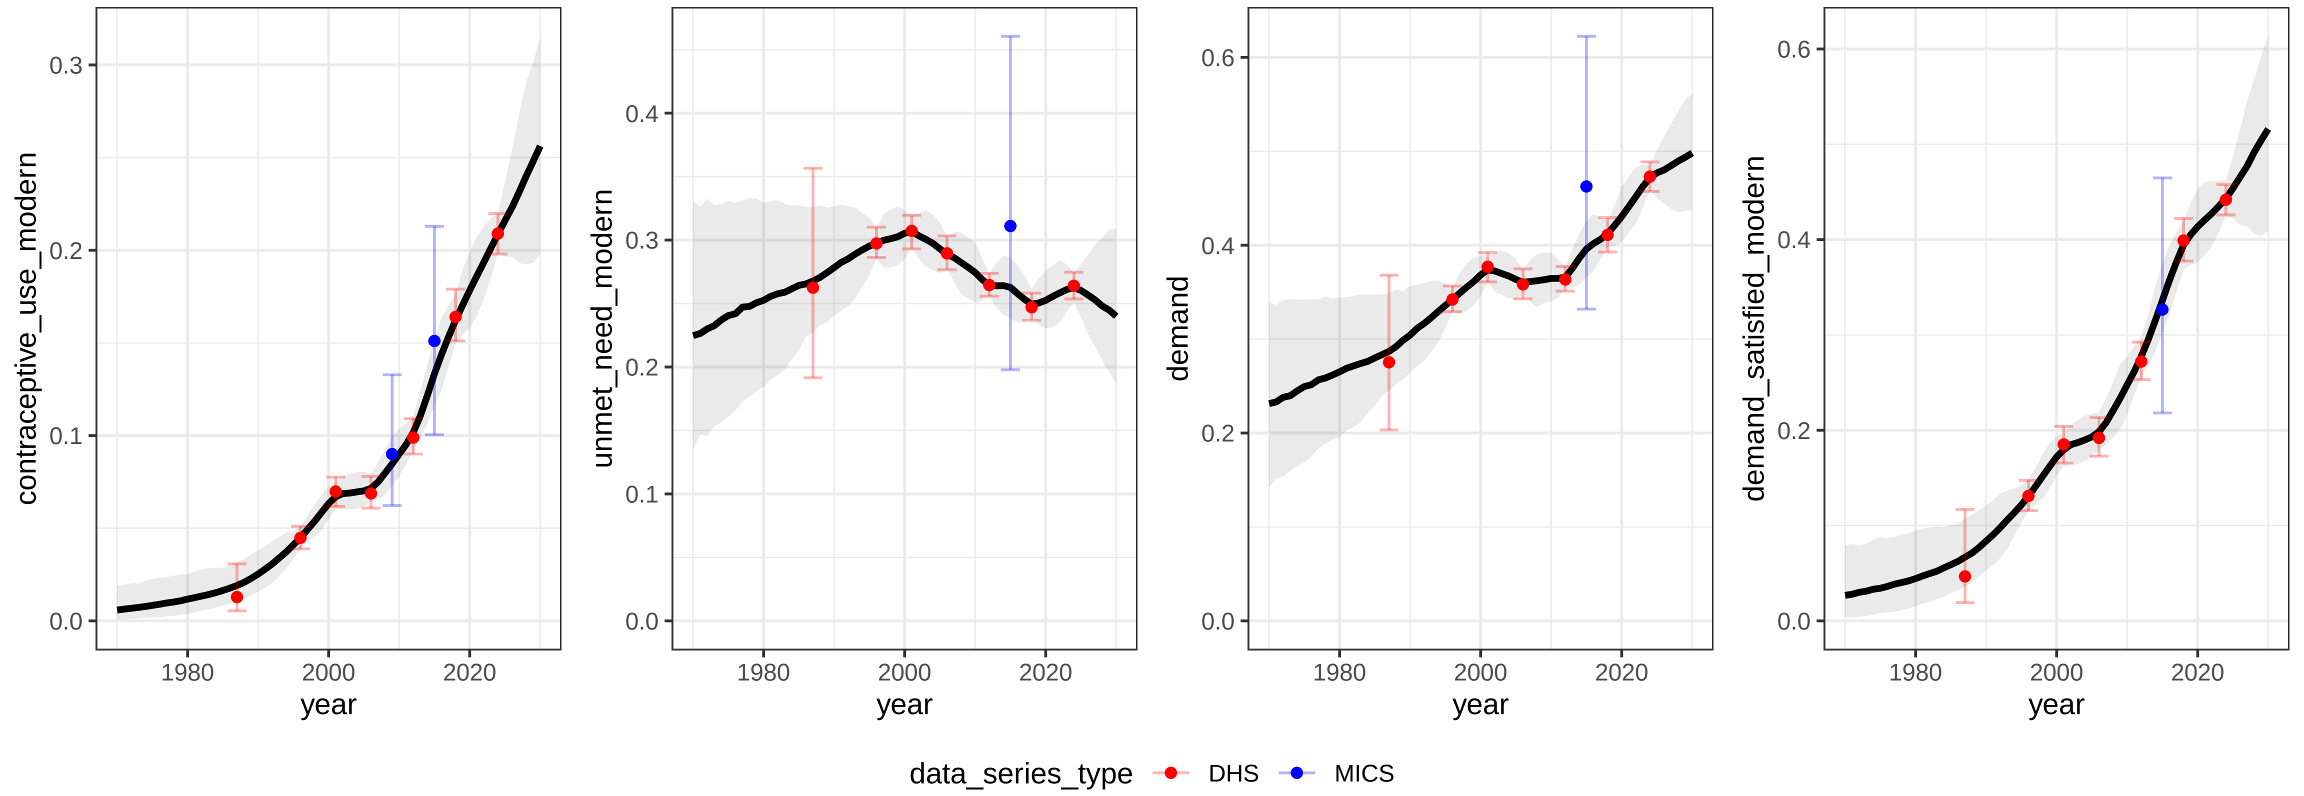

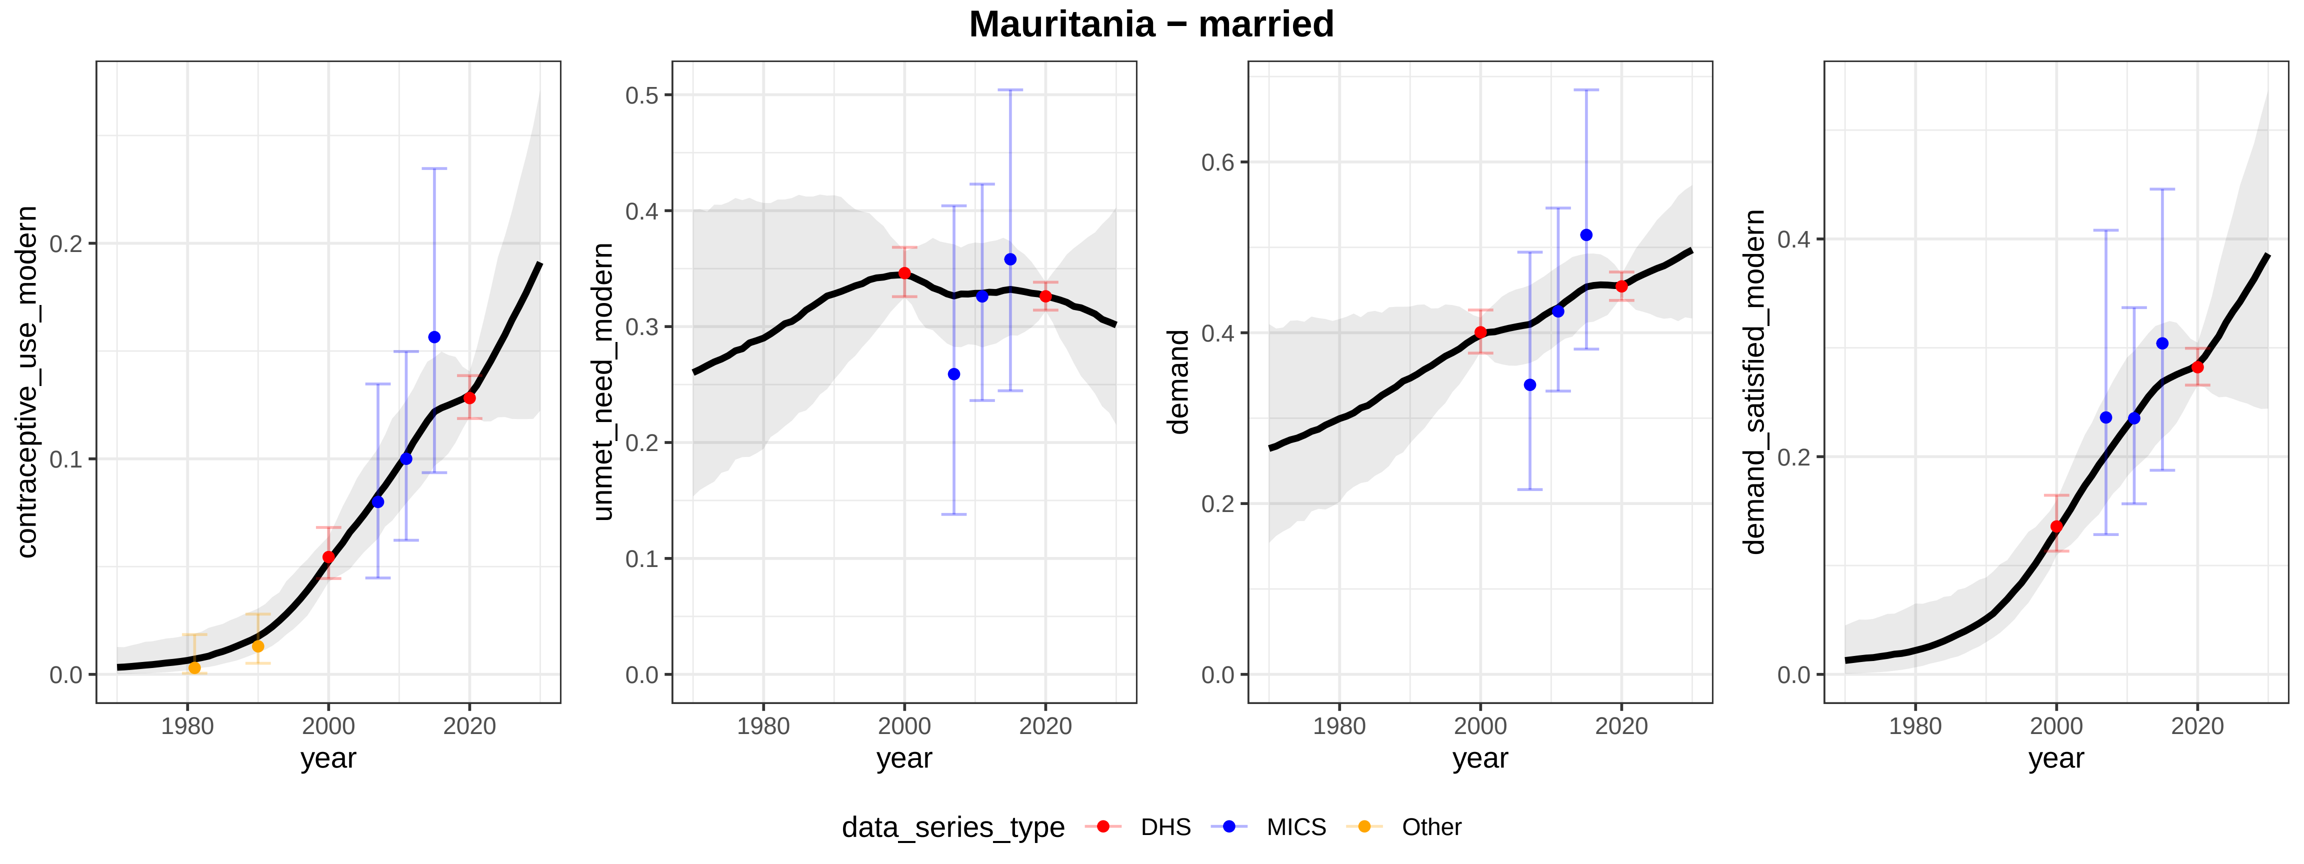

Mauritania − married
contraceptive_use_modern
unmet_need_modern
demand
demand_satisfied_modern
year
data_series_type
DHS
MICS
Other

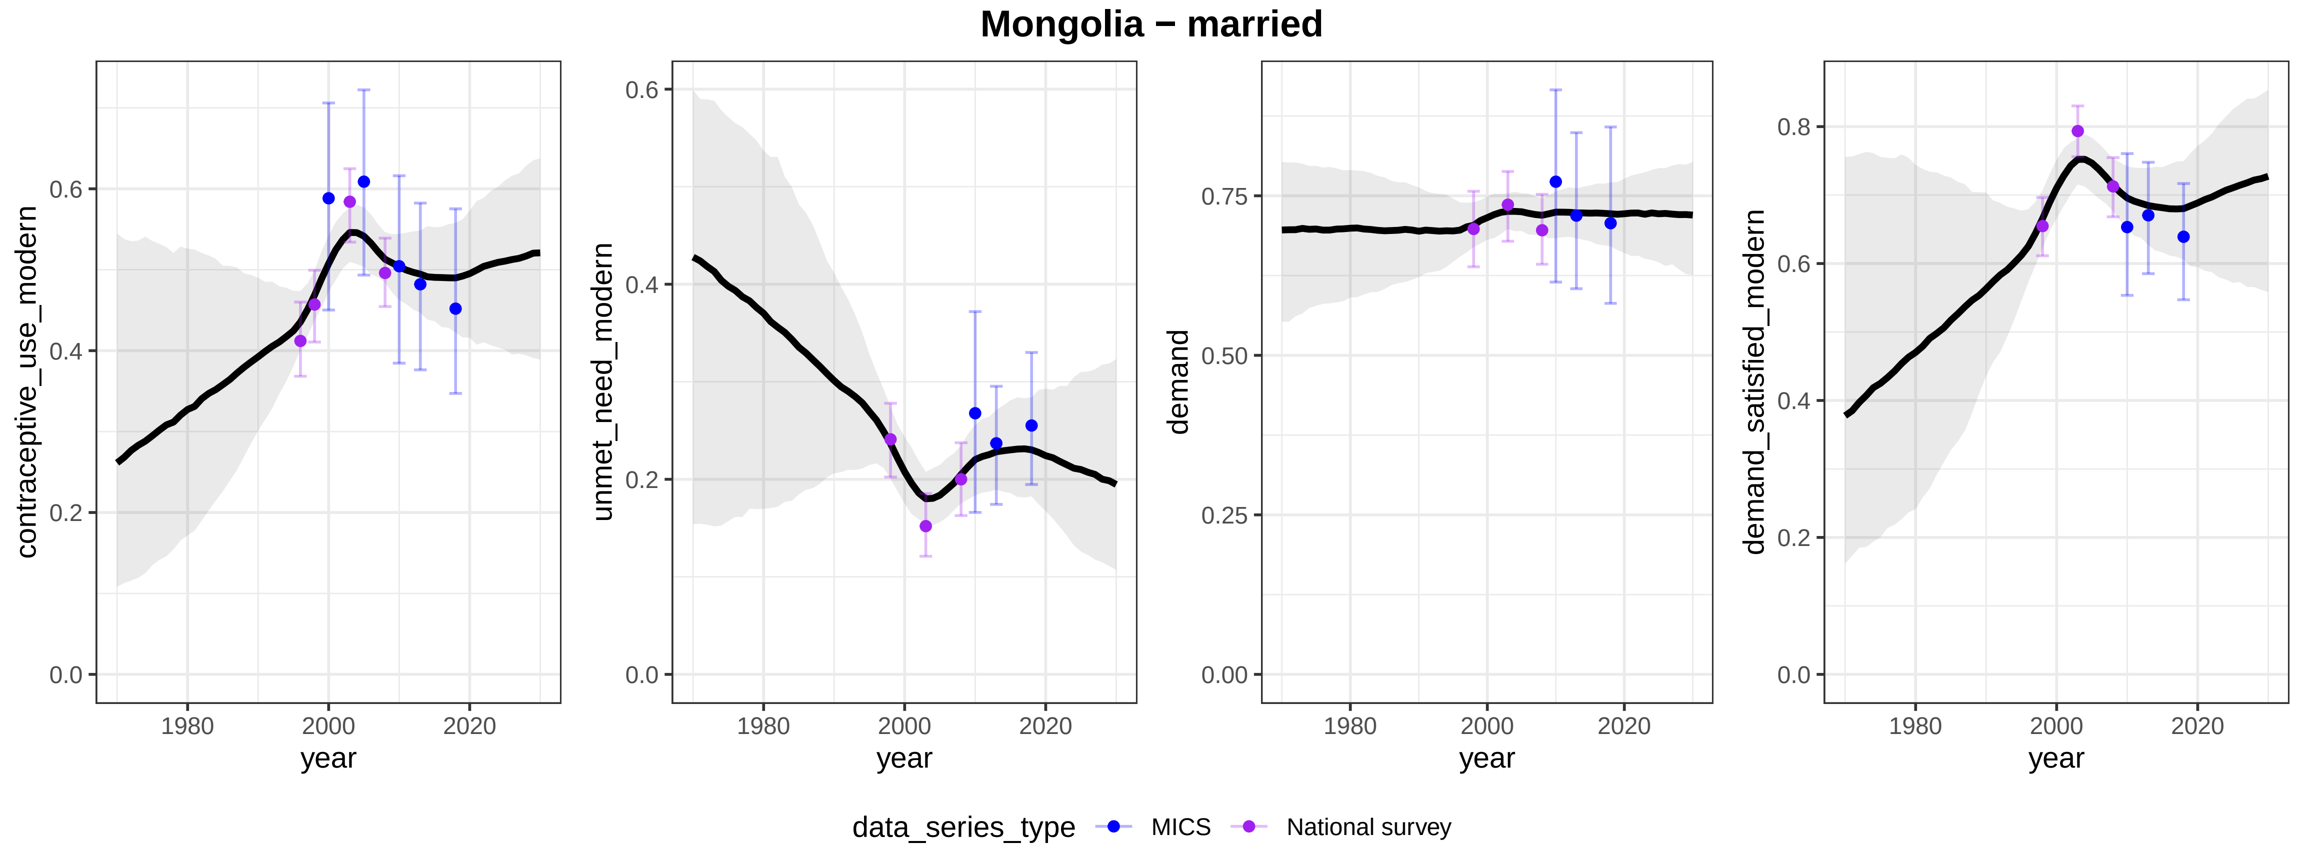
Mongolia − married
contraceptive_use_modern
unmet_need_modern
demand
demand_satisfied_modern
year
data_series_type
MICS
National survey

# Mozambique − married

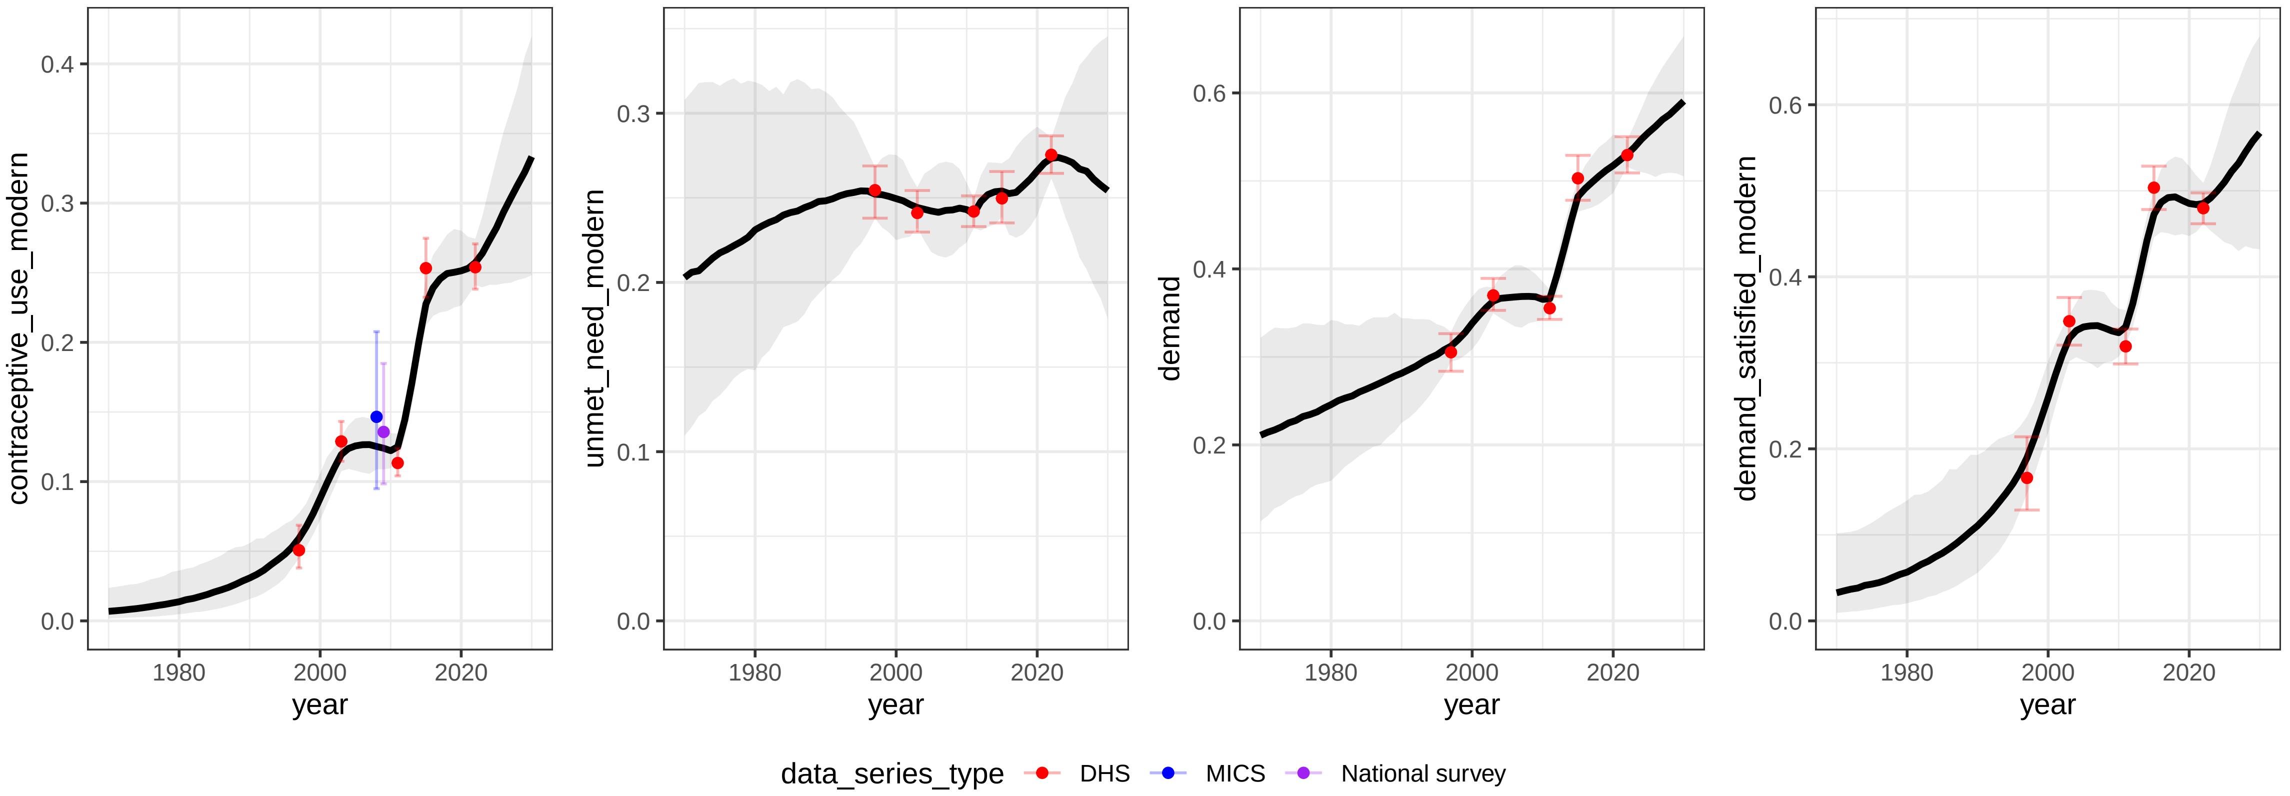

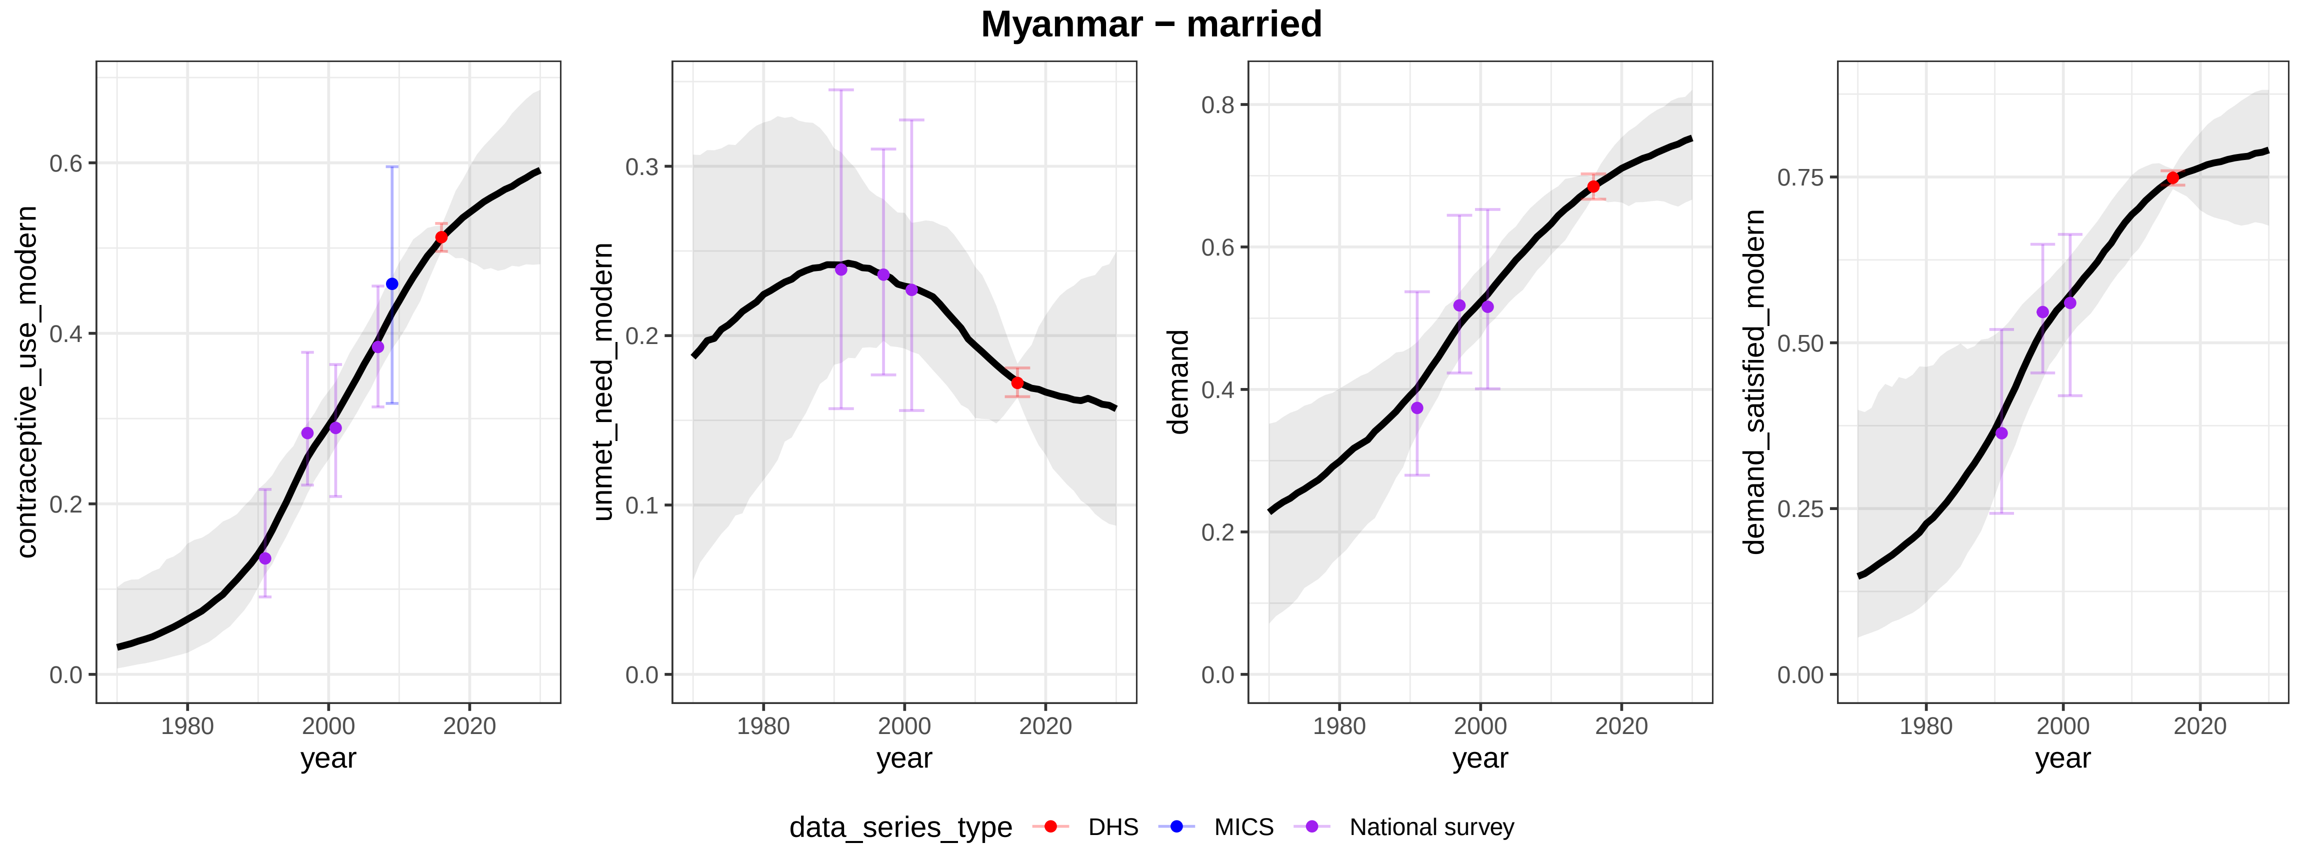

Myanmar − married
contraceptive_use_modern
unmet_need_modern
demand
demand_satisfied_modern
year
data_series_type
DHS
MICS
National survey

# Nepal − married

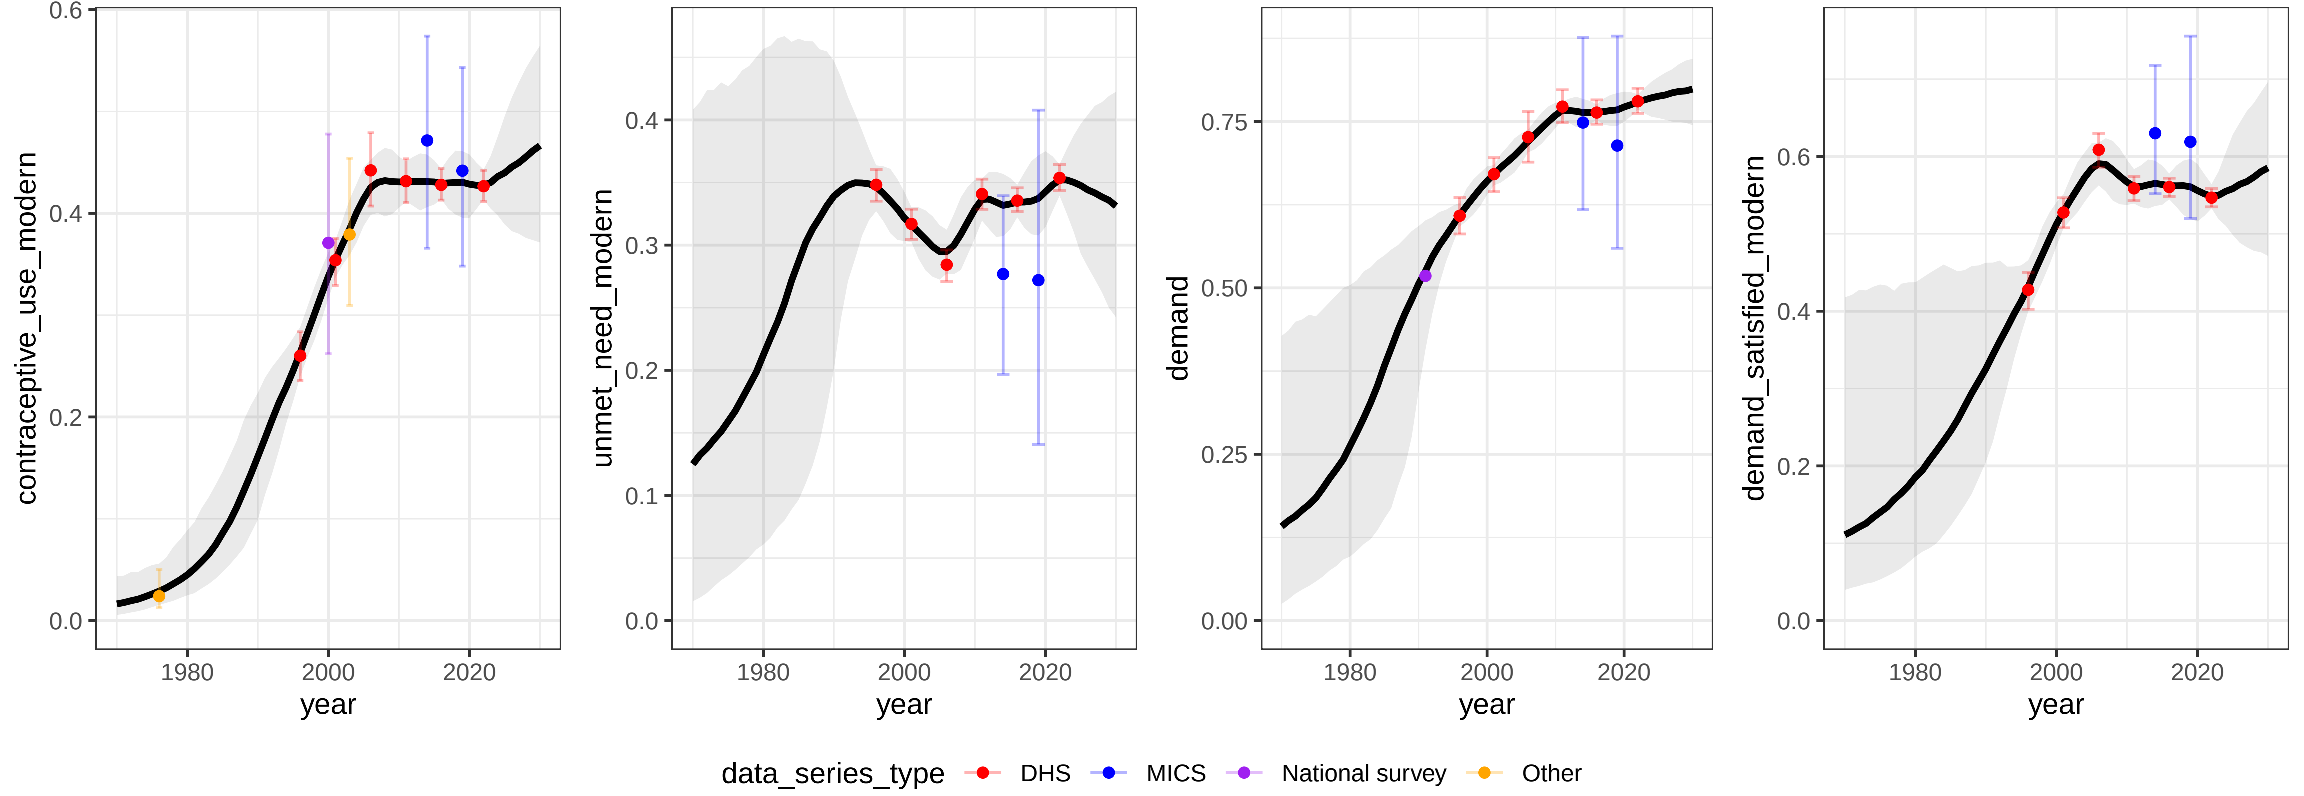

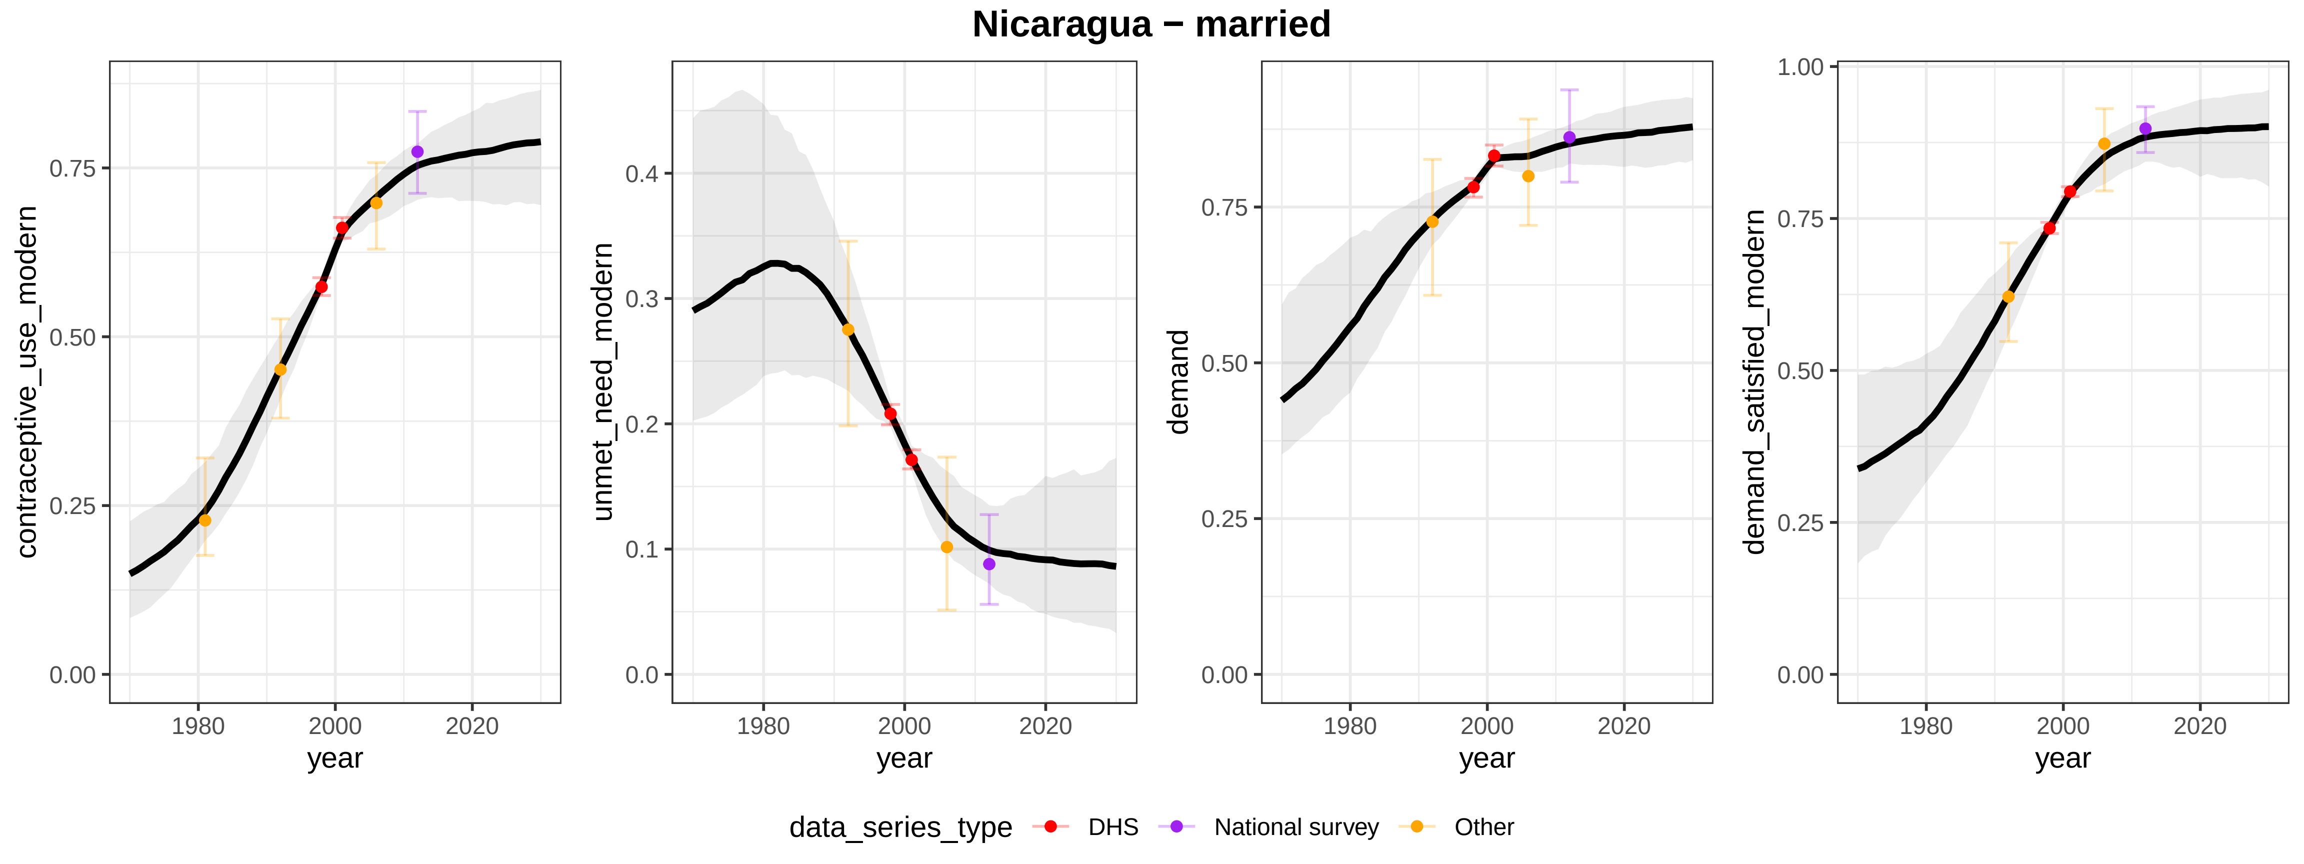

Nicaragua − married
contraceptive_use_modern
unmet_need_modern
demand
demand_satisfied_modern
0.00
0.25
0.50
0.75
1.00
0.0
0.1
0.2
0.3
0.4
1980
2000
2020
year
data_series_type
DHS
National survey
Other

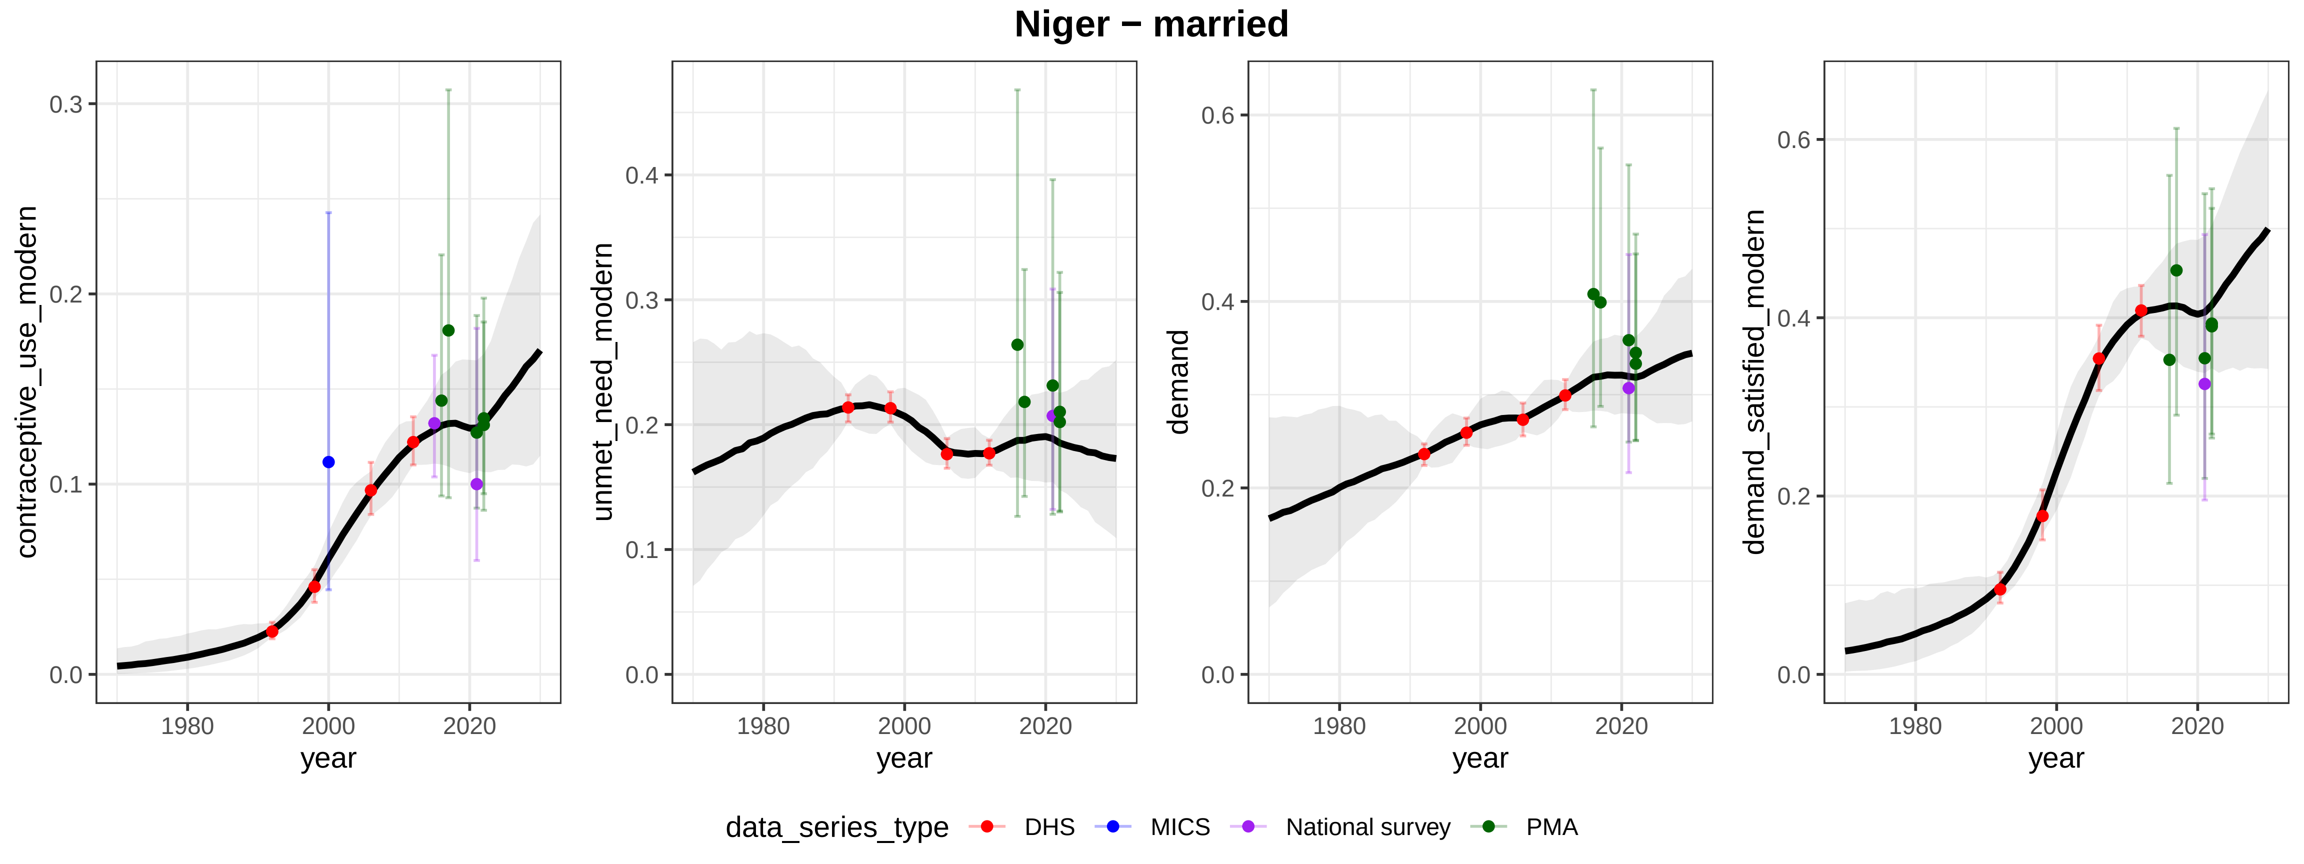

Niger − married
contraceptive_use_modern
unmet_need_modern
demand
demand_satisfied_modern
year
data_series_type
DHS
MICS
National survey
PMA

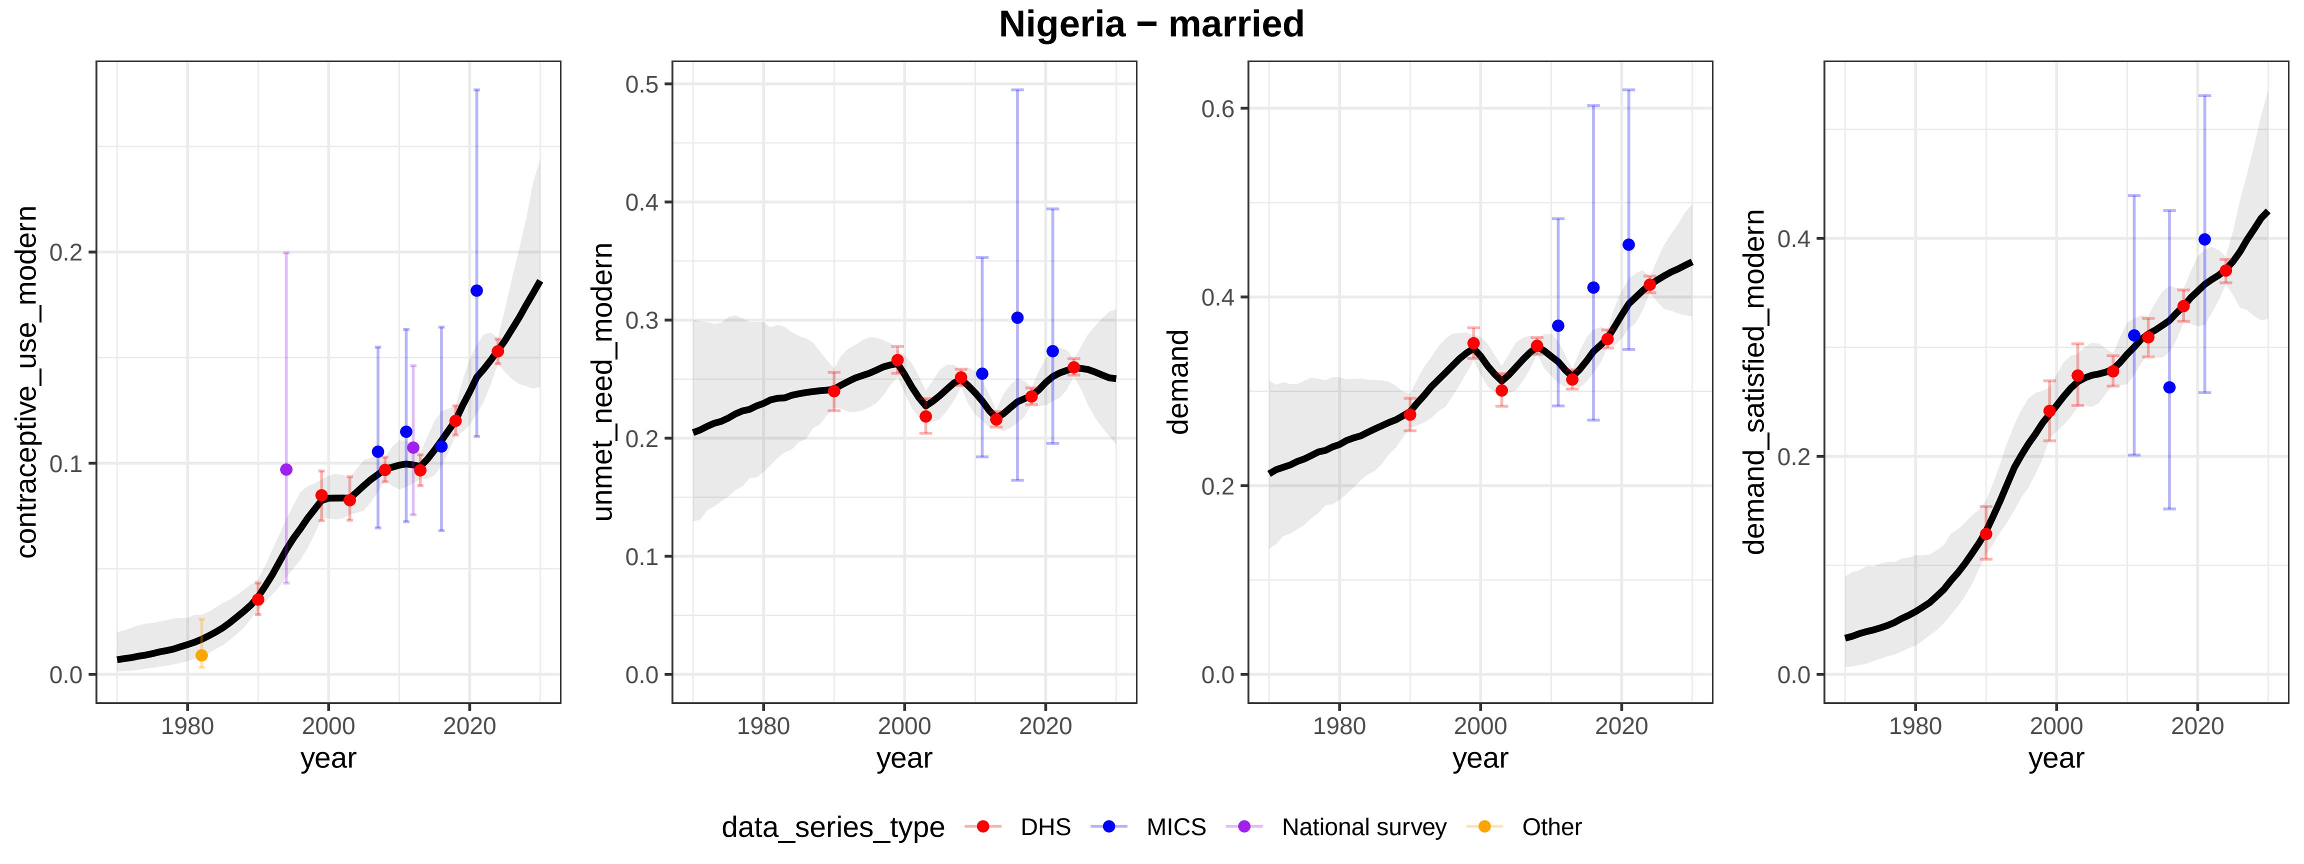

Nigeria − married
contraceptive_use_modern
unmet_need_modern
demand
demand_satisfied_modern
year
1980
2000
2020
0.0
0.1
0.2
0.3
0.4
0.5
0.6
data_series_type
DHS
MICS
National survey
Other

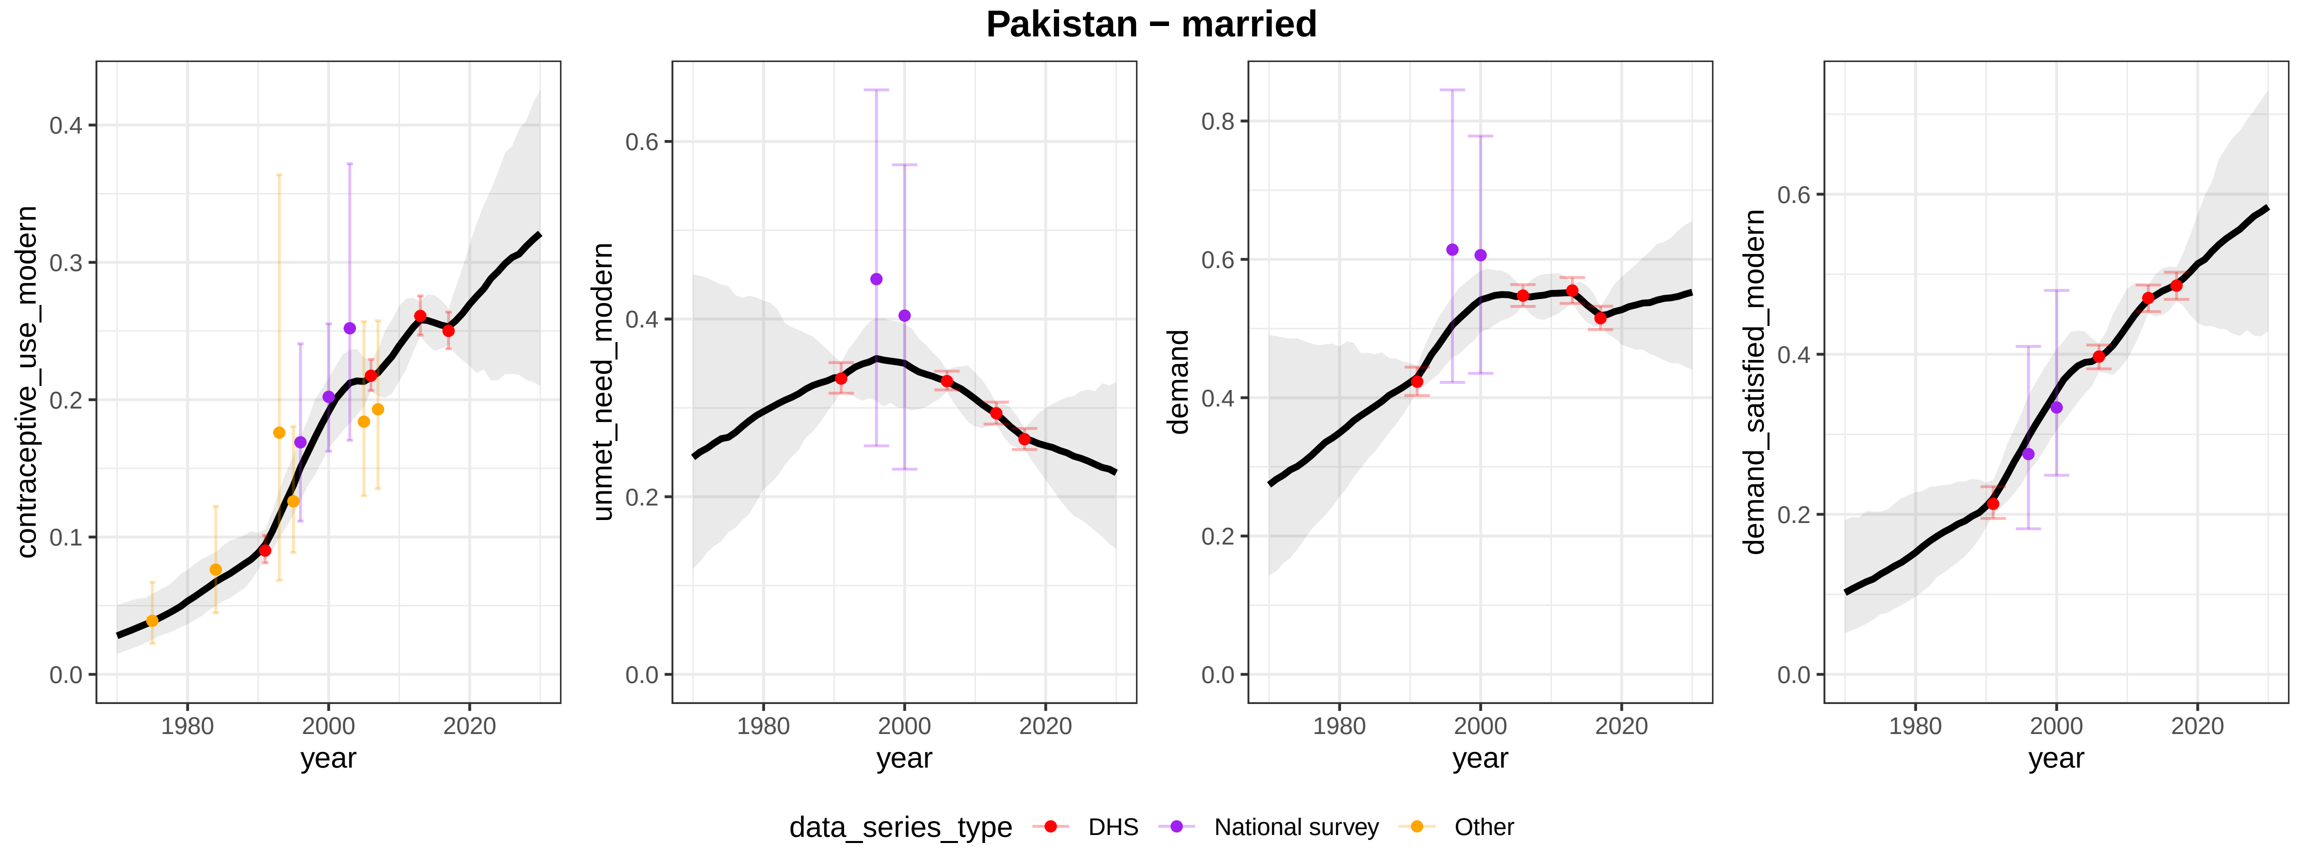

Pakistan − married
contraceptive_use_modern
unmet_need_modern
demand
demand_satisfied_modern
year
1980
2000
2020
0.0
0.1
0.2
0.3
0.4
0.6
0.8
data_series_type
DHS
National survey
Other

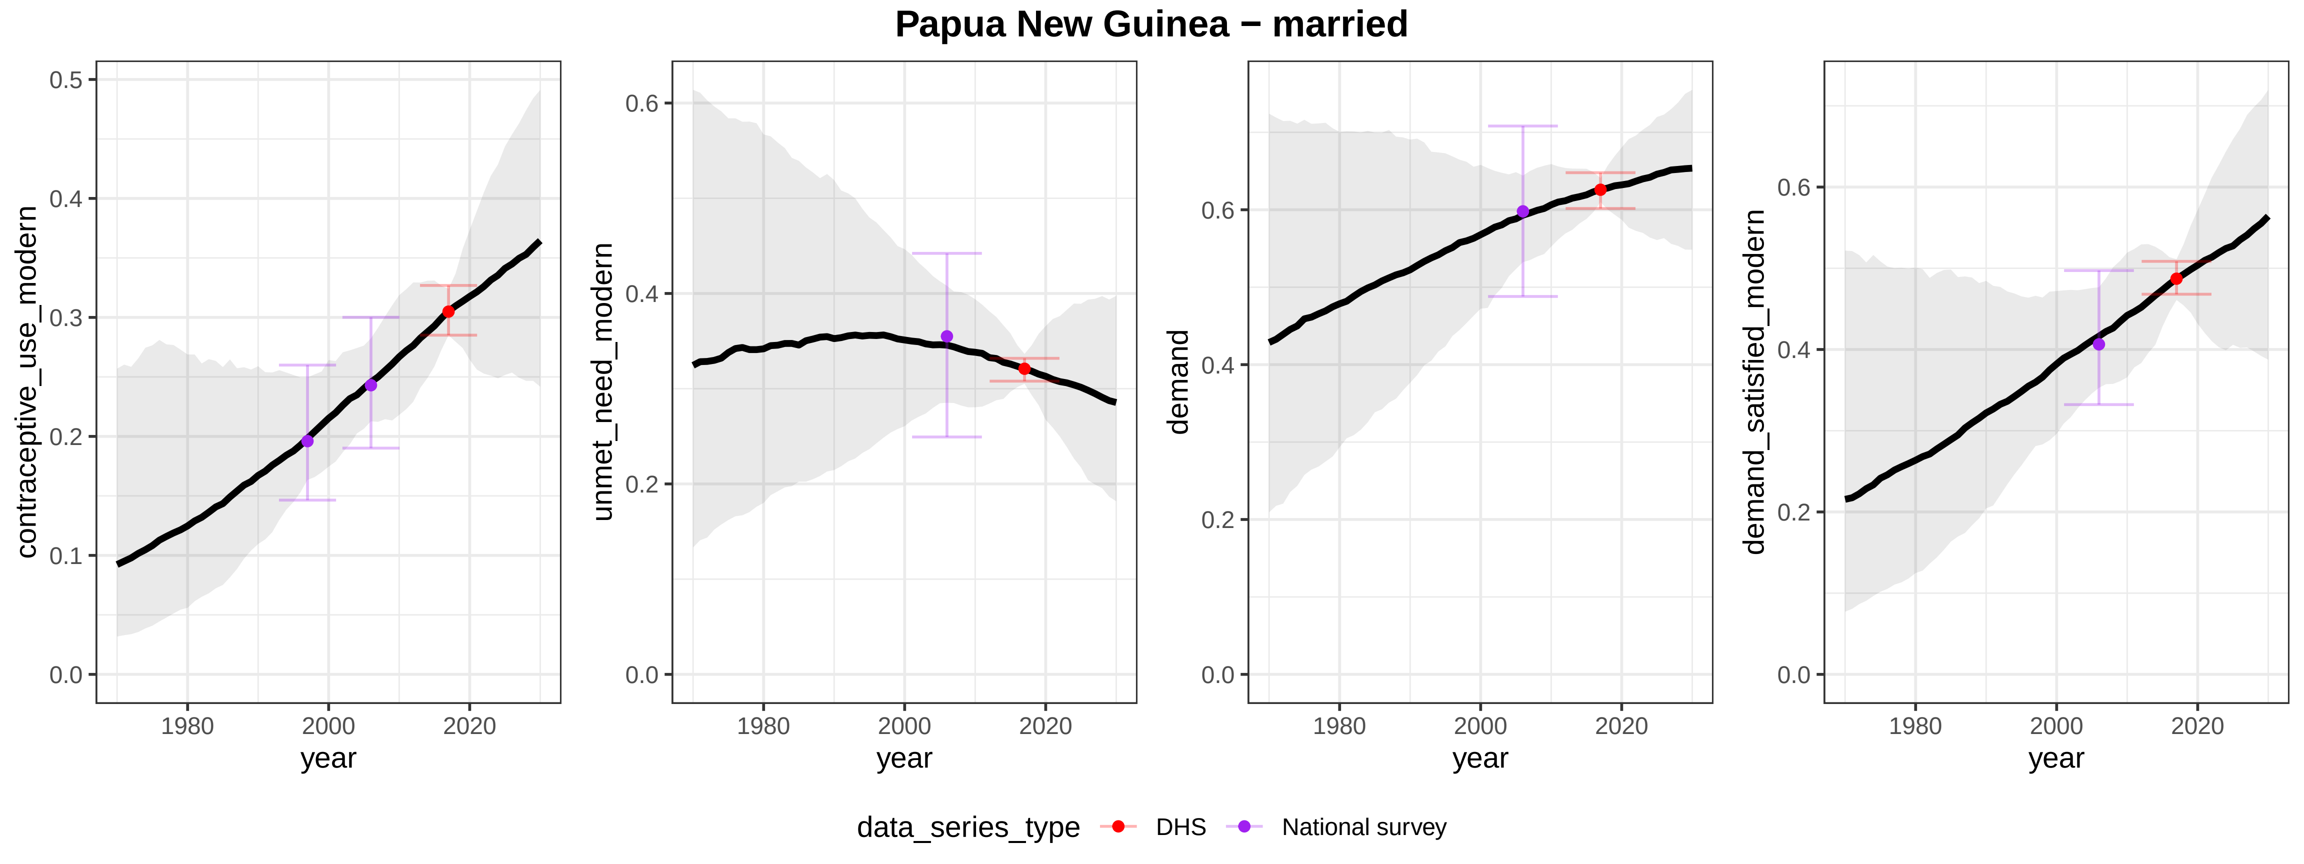

Papua New Guinea − married
contraceptive_use_modern
unmet_need_modern
demand
demand_satisfied_modern
year
1980
2000
2020
0.0
0.1
0.2
0.3
0.4
0.5
0.6
data_series_type
DHS
National survey

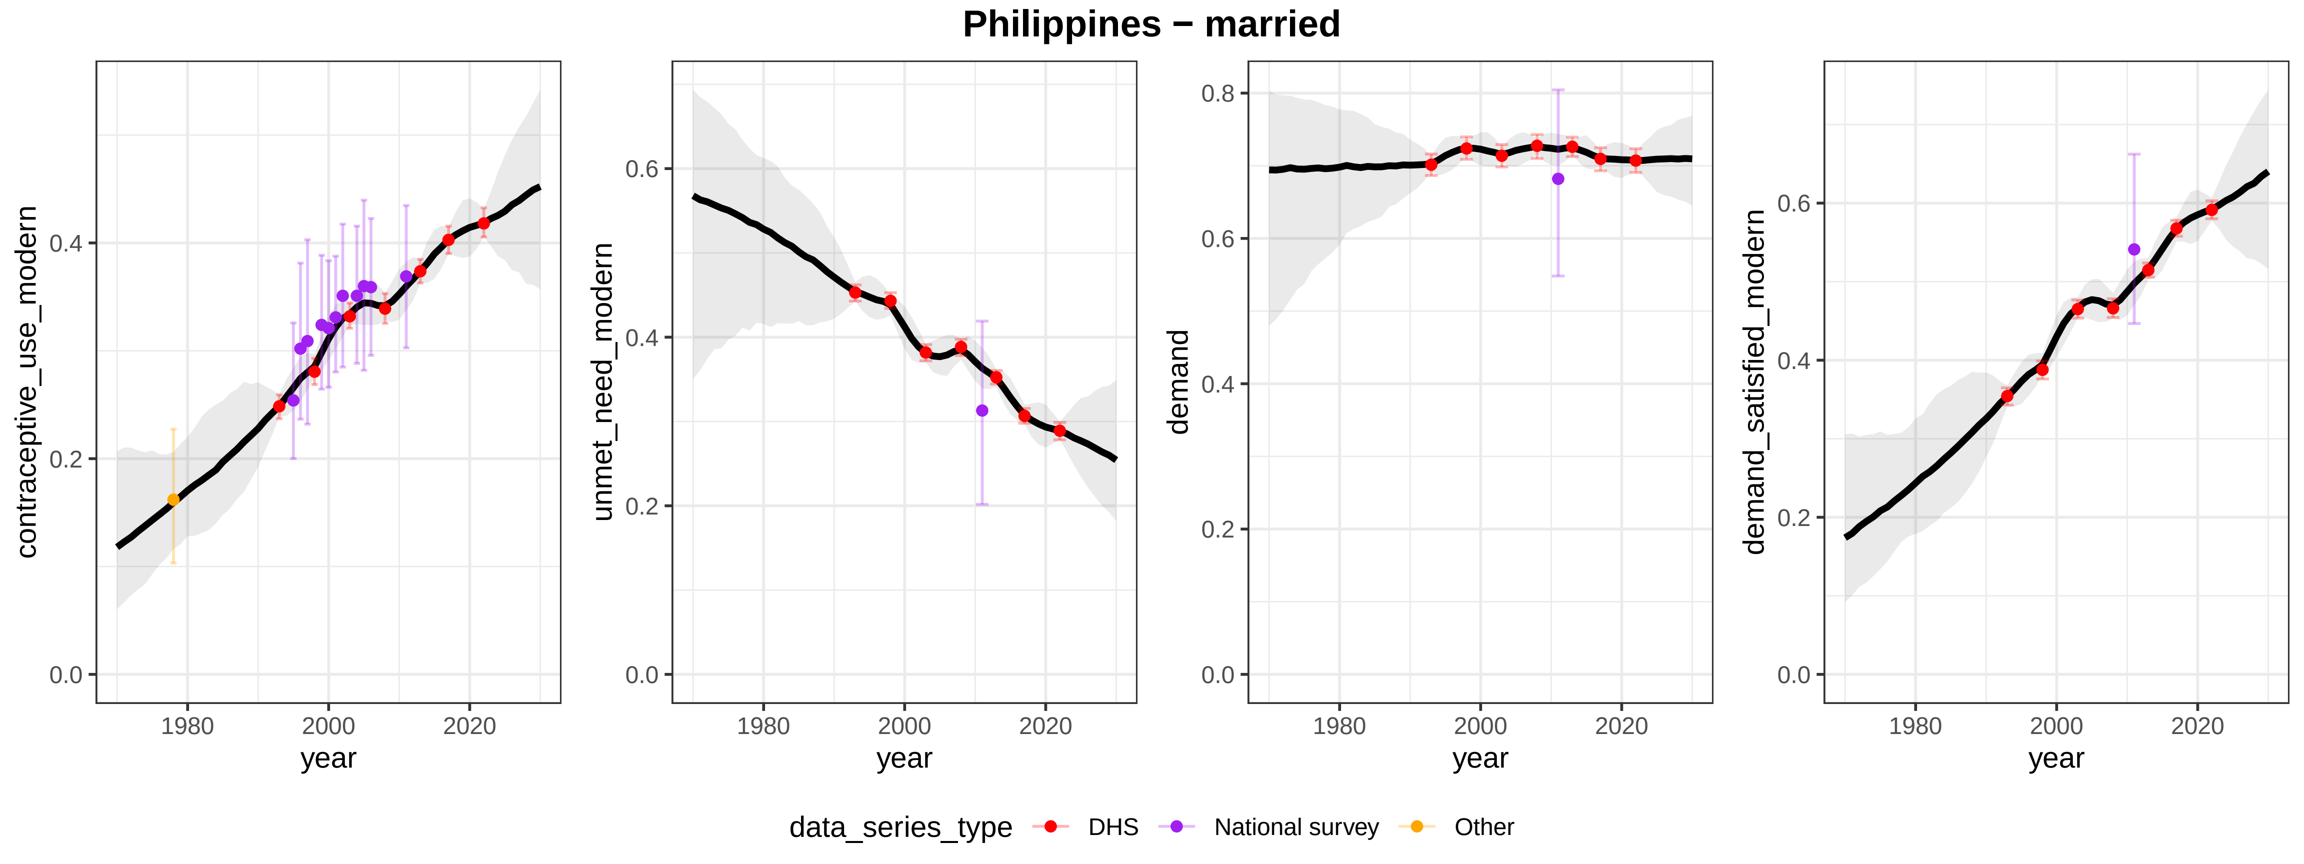

Philippines − married
contraceptive_use_modern
unmet_need_modern
demand
demand_satisfied_modern
year
data_series_type
DHS
National survey
Other

# Rwanda − married

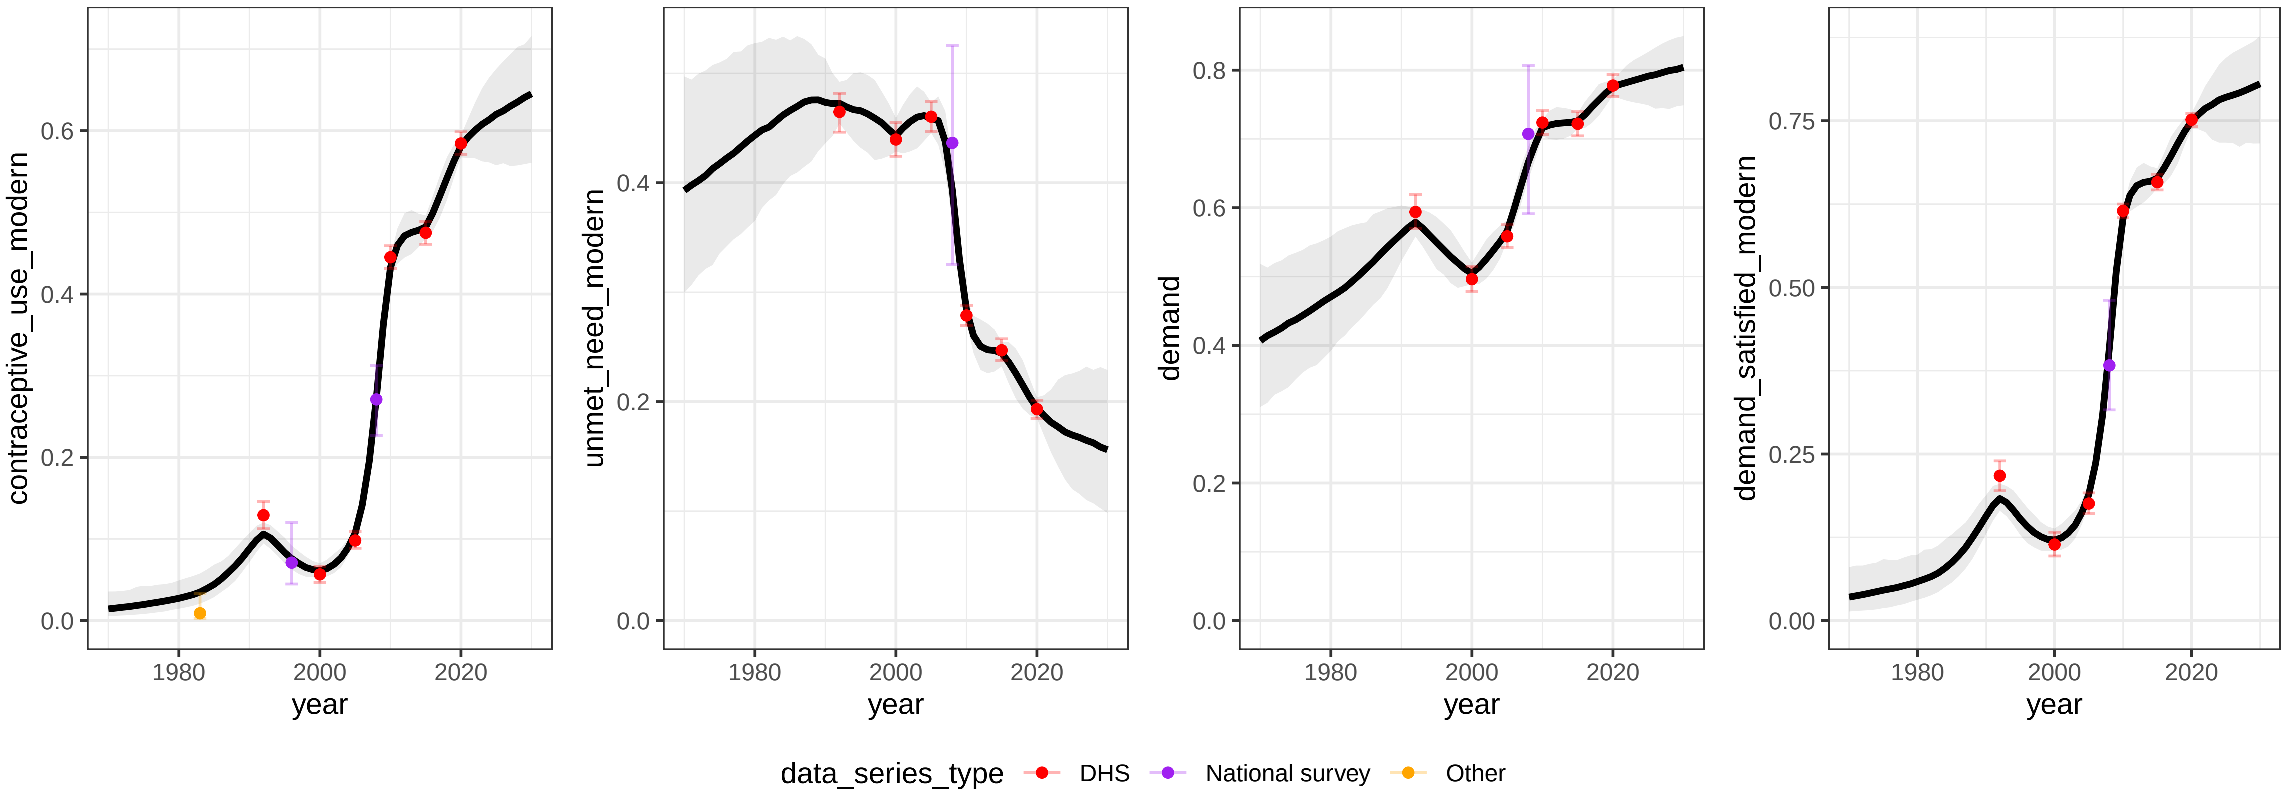

# Sao Tome and Principe − married

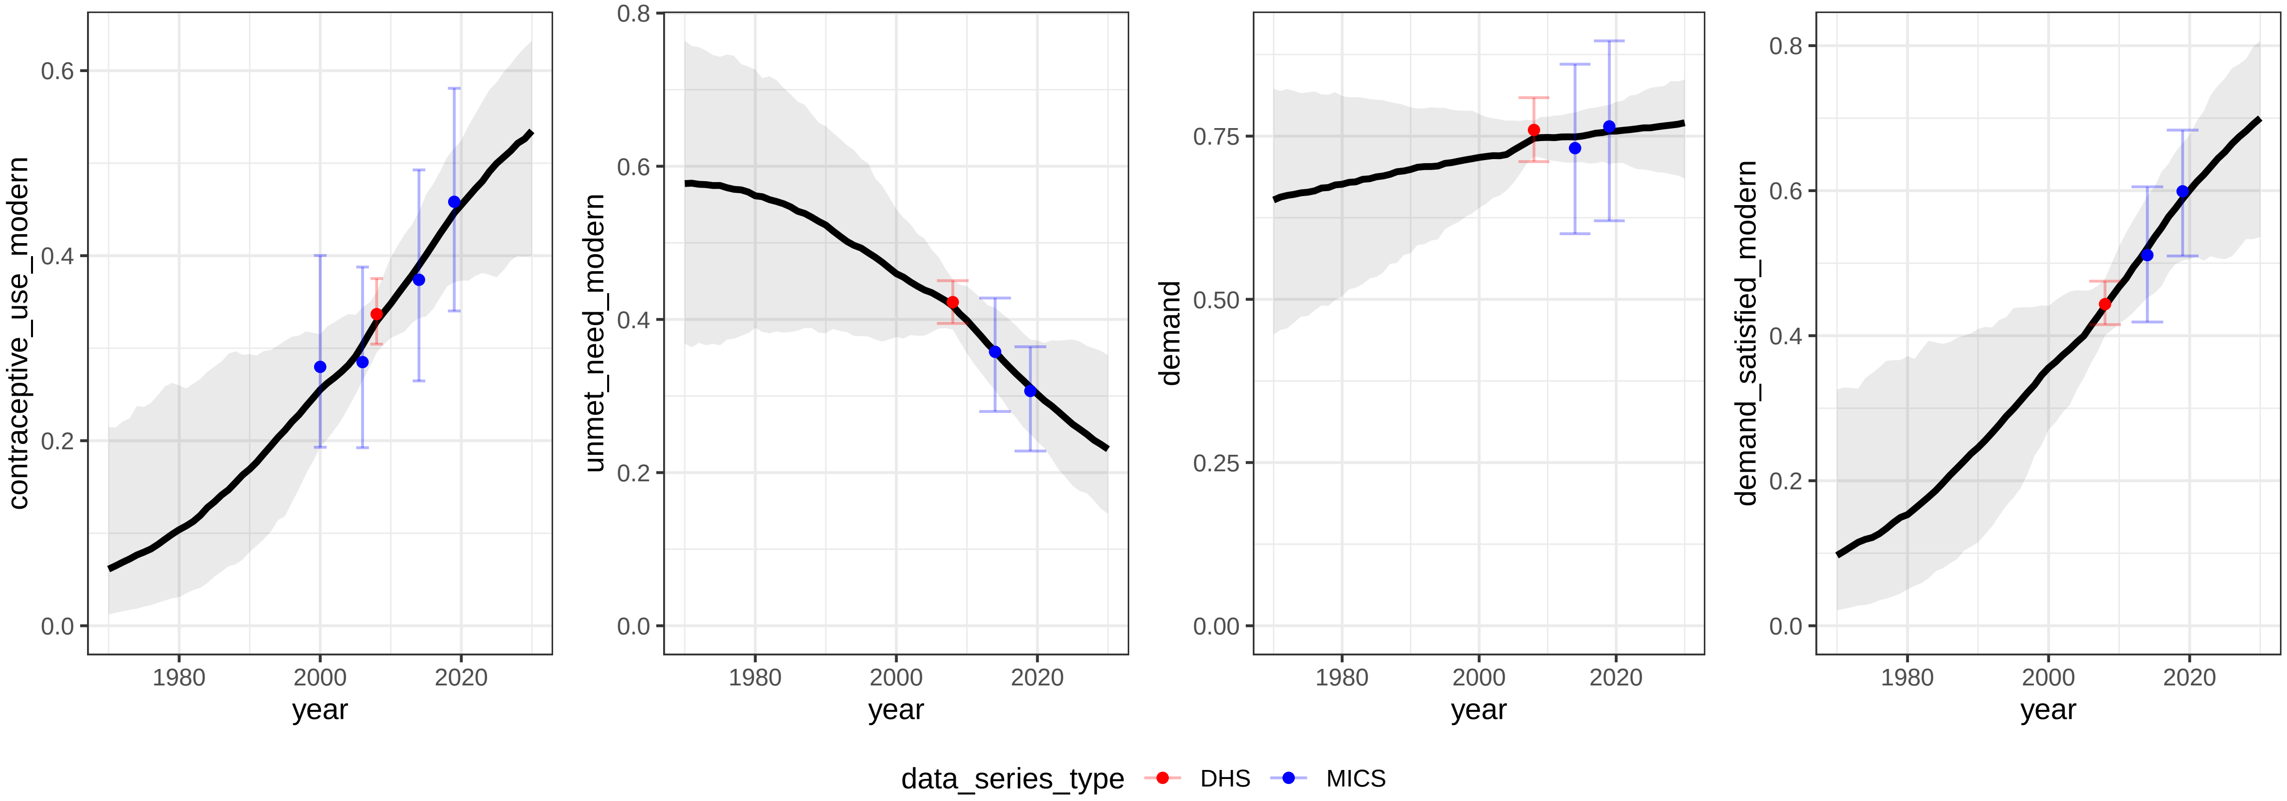

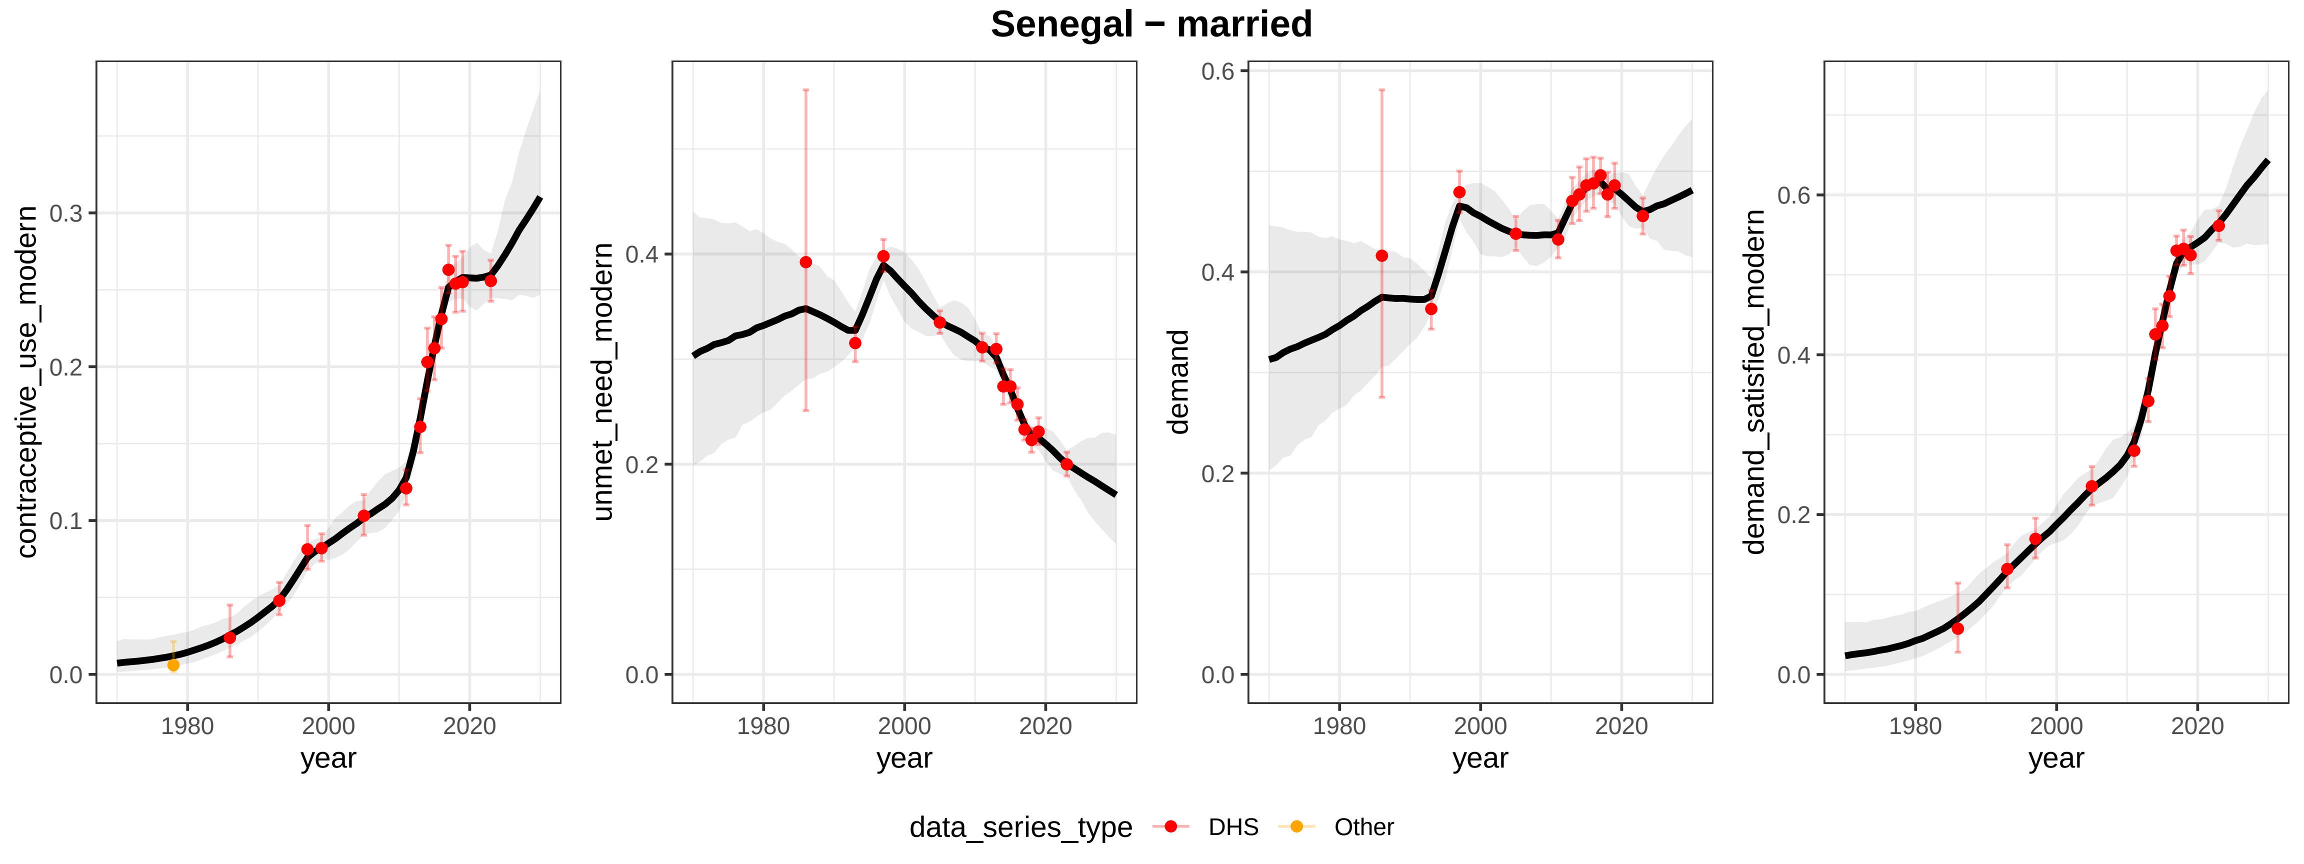
Senegal − married
contraceptive_use_modern
unmet_need_modern
demand
demand_satisfied_modern
year
0.0
0.1
0.2
0.3
0.4
0.6
1980
2000
2020
data_series_type
DHS
Other

# Sierra Leone − married

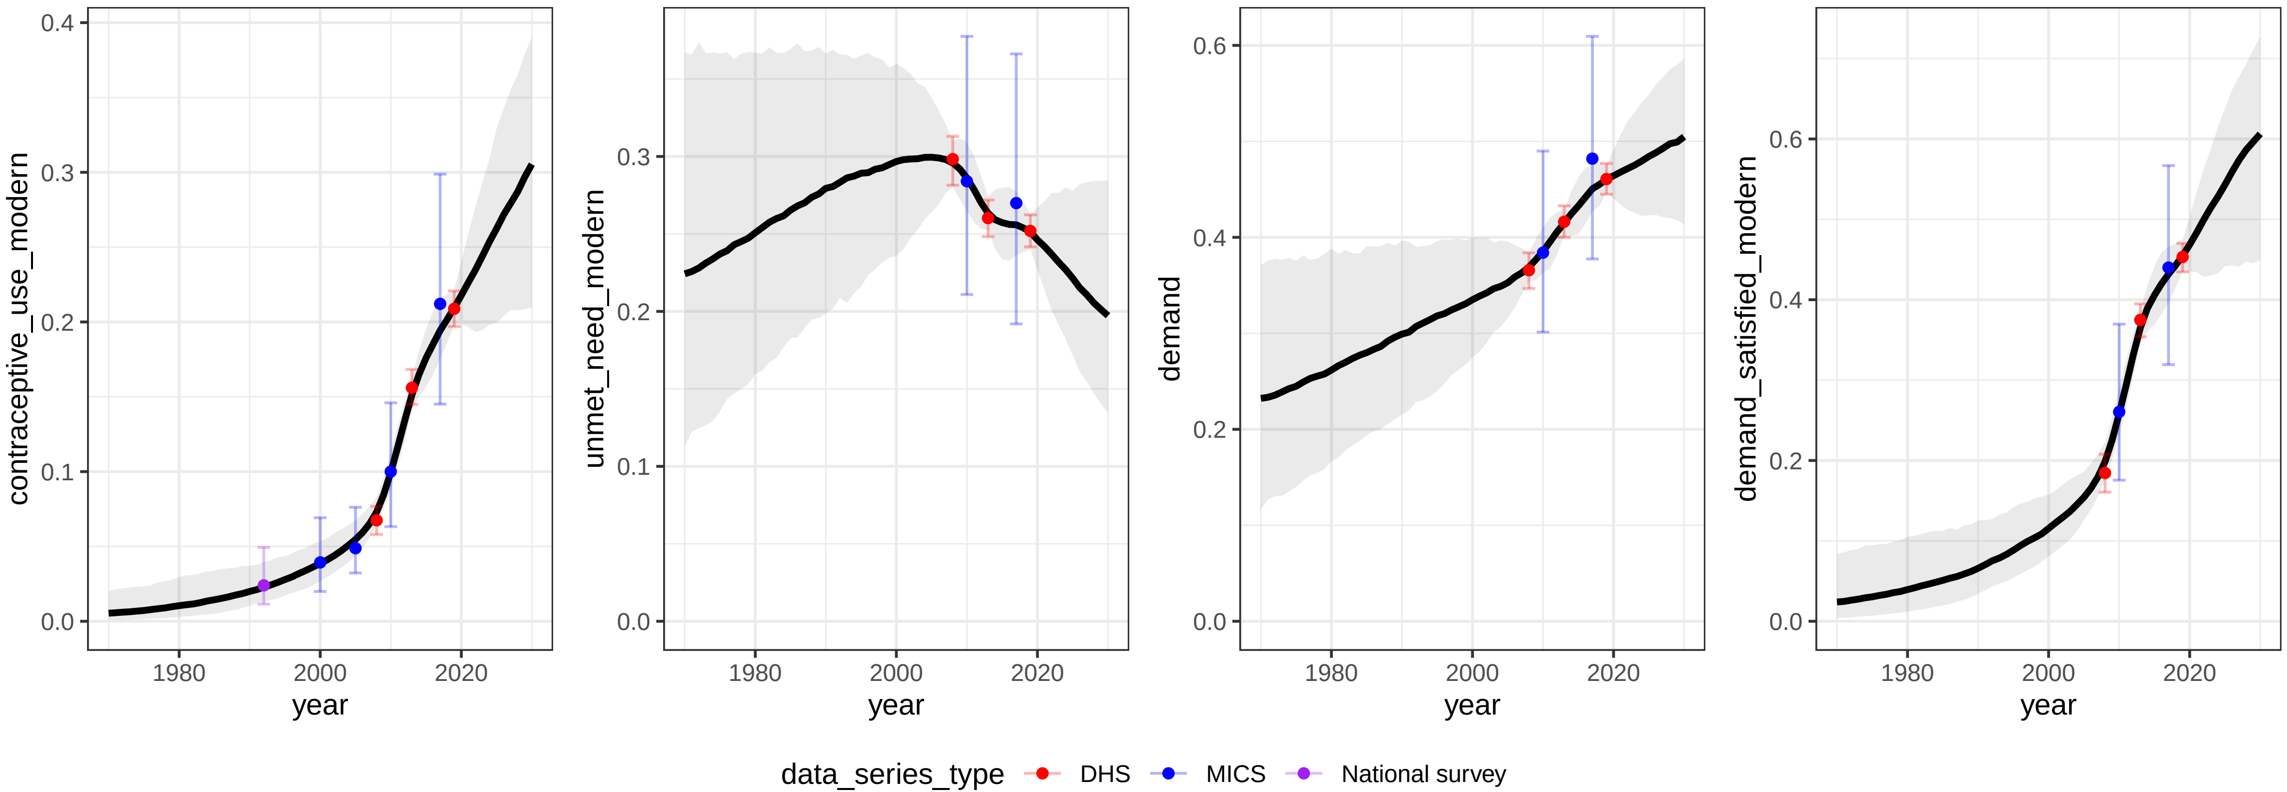

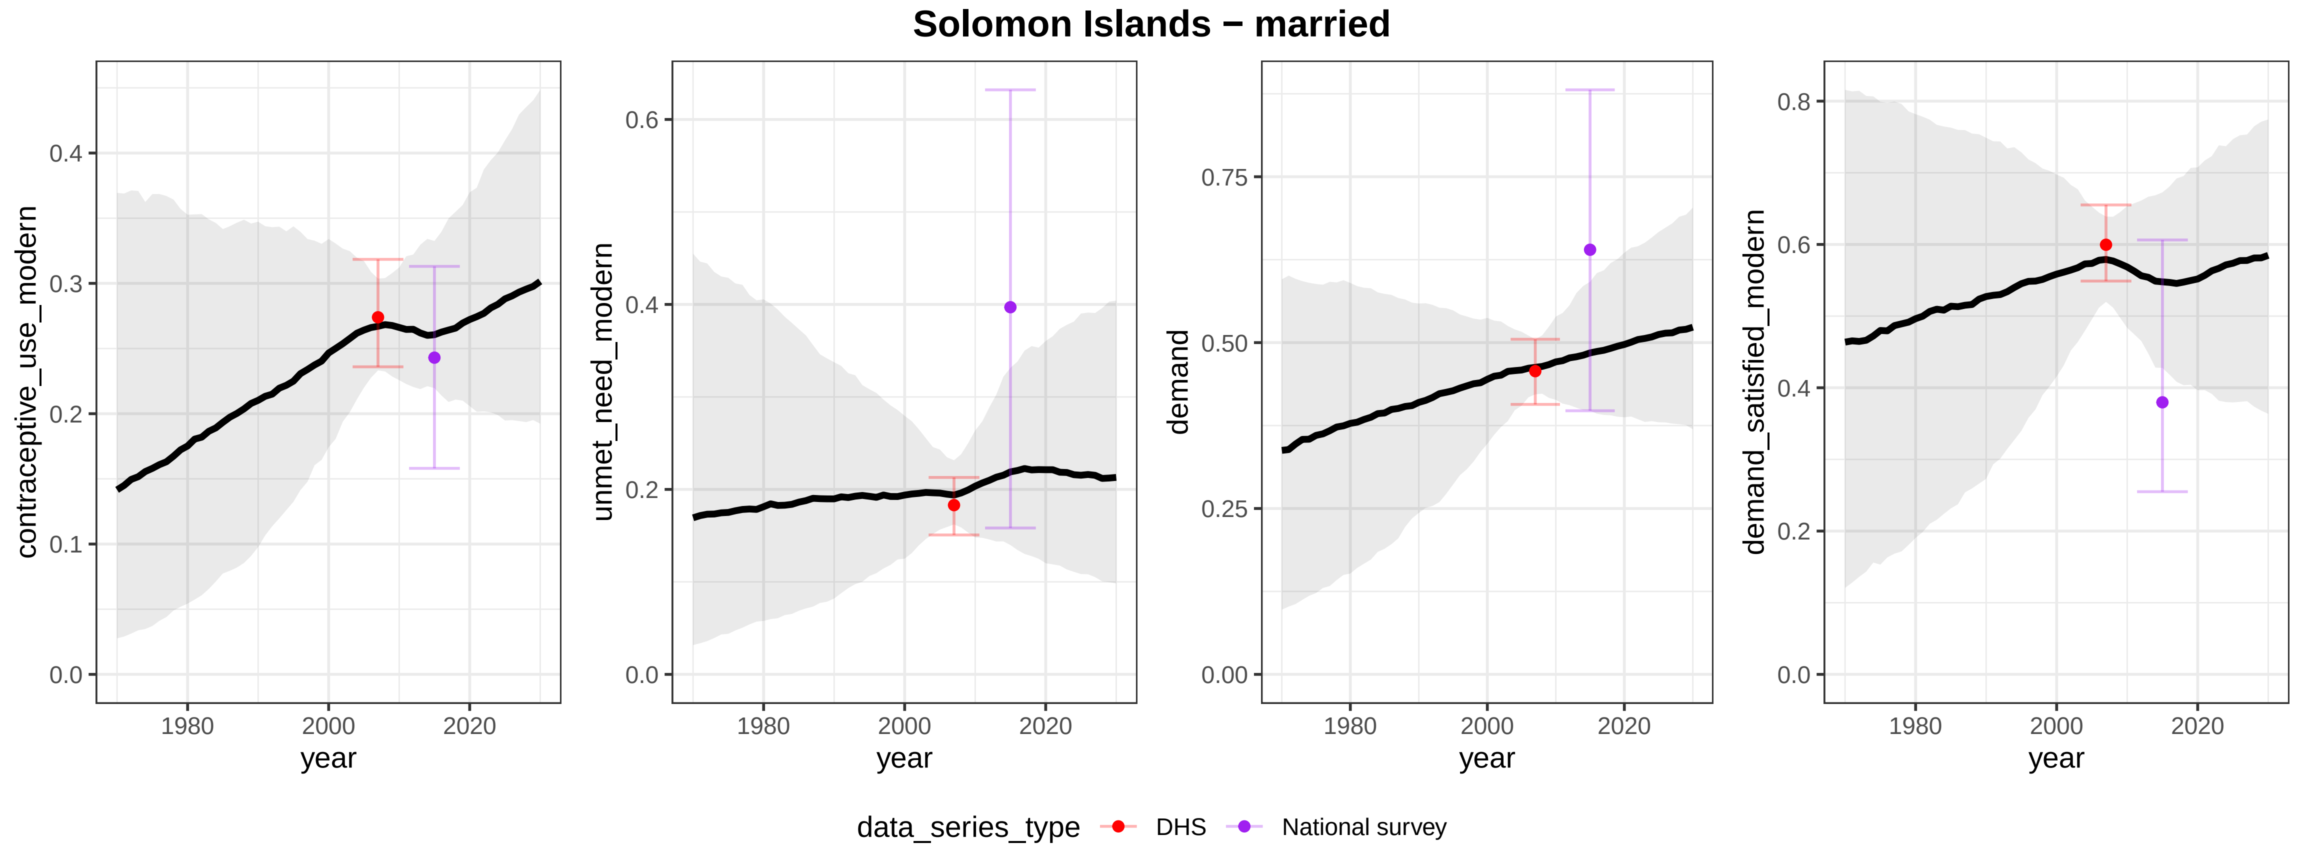

Solomon Islands − married
contraceptive_use_modern
unmet_need_modern
demand
demand_satisfied_modern
year
1980
2000
2020
0.0
0.1
0.2
0.3
0.4
0.6
0.00
0.25
0.50
0.75
0.8
data_series_type
DHS
National survey

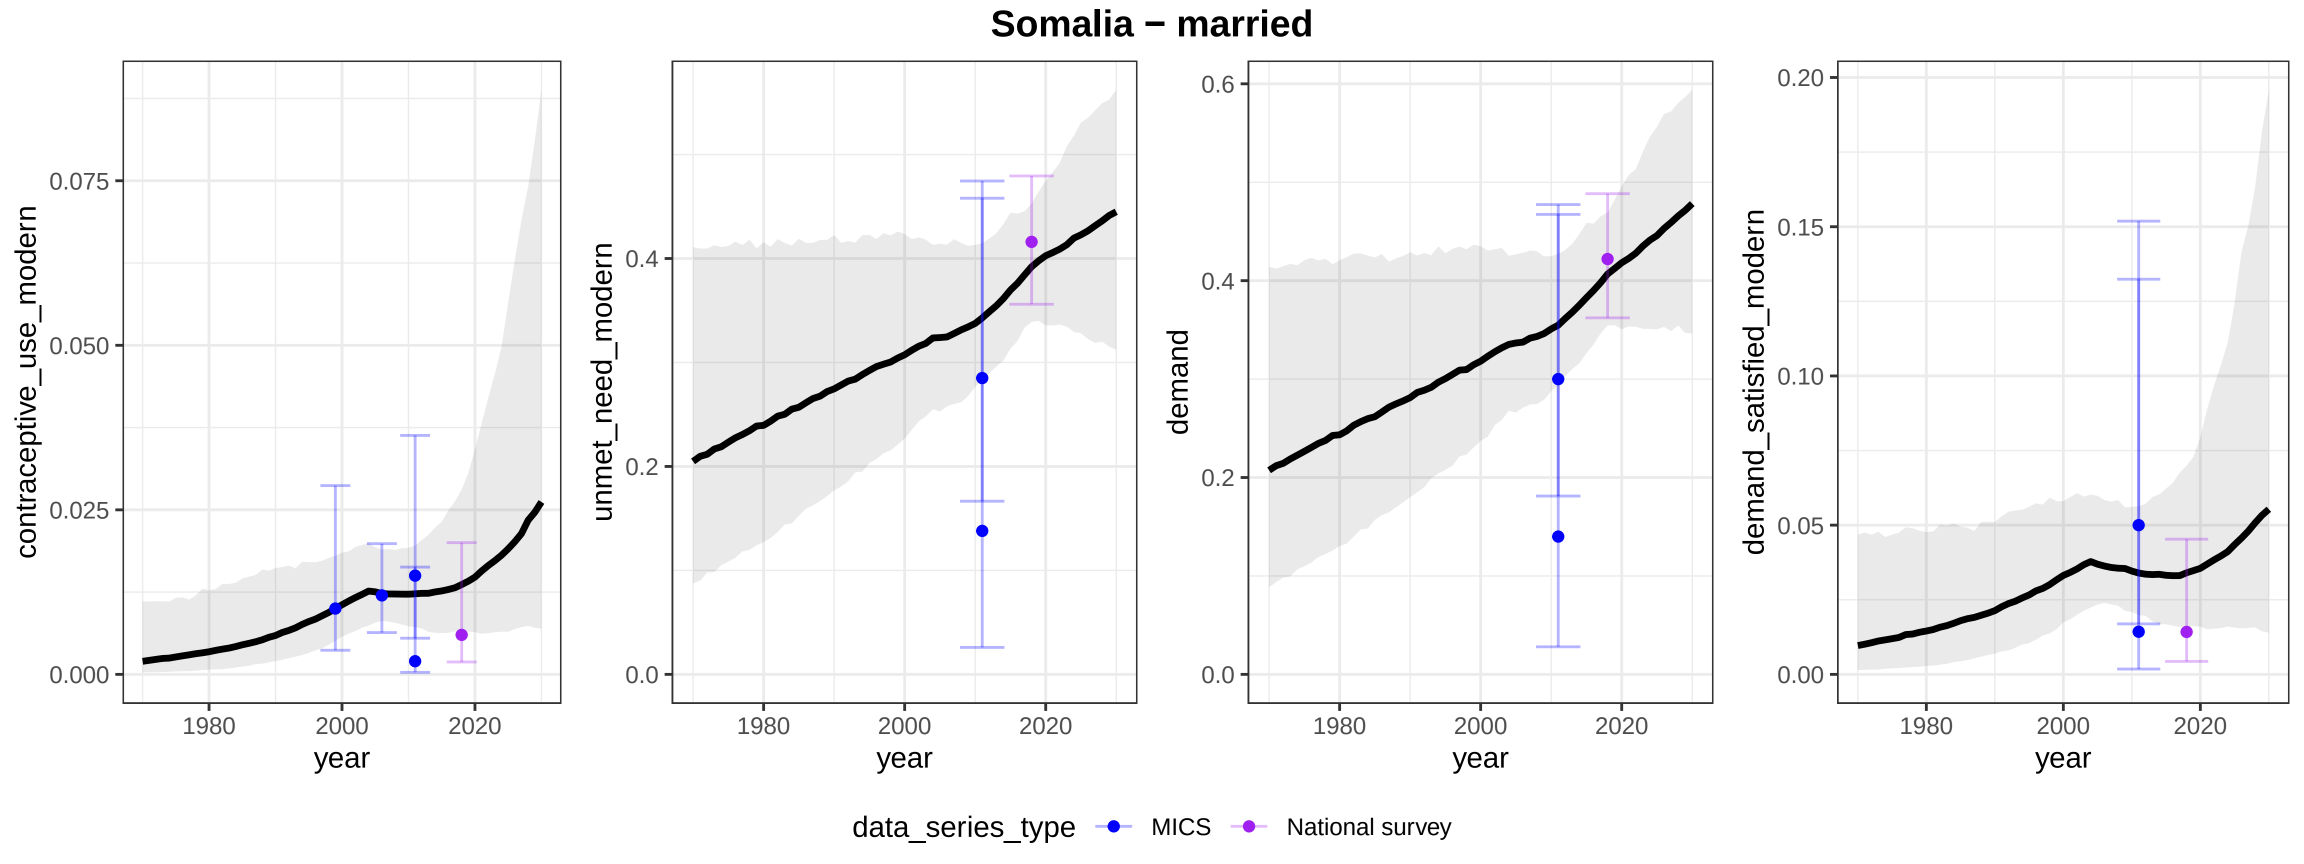

Somalia − married
contraceptive_use_modern
0.000
0.025
0.050
0.075
unmet_need_modern
0.0
0.2
0.4
demand
0.0
0.2
0.4
0.6
demand_satisfied_modern
0.00
0.05
0.10
0.15
0.20
1980
2000
2020
year
data_series_type
MICS
National survey

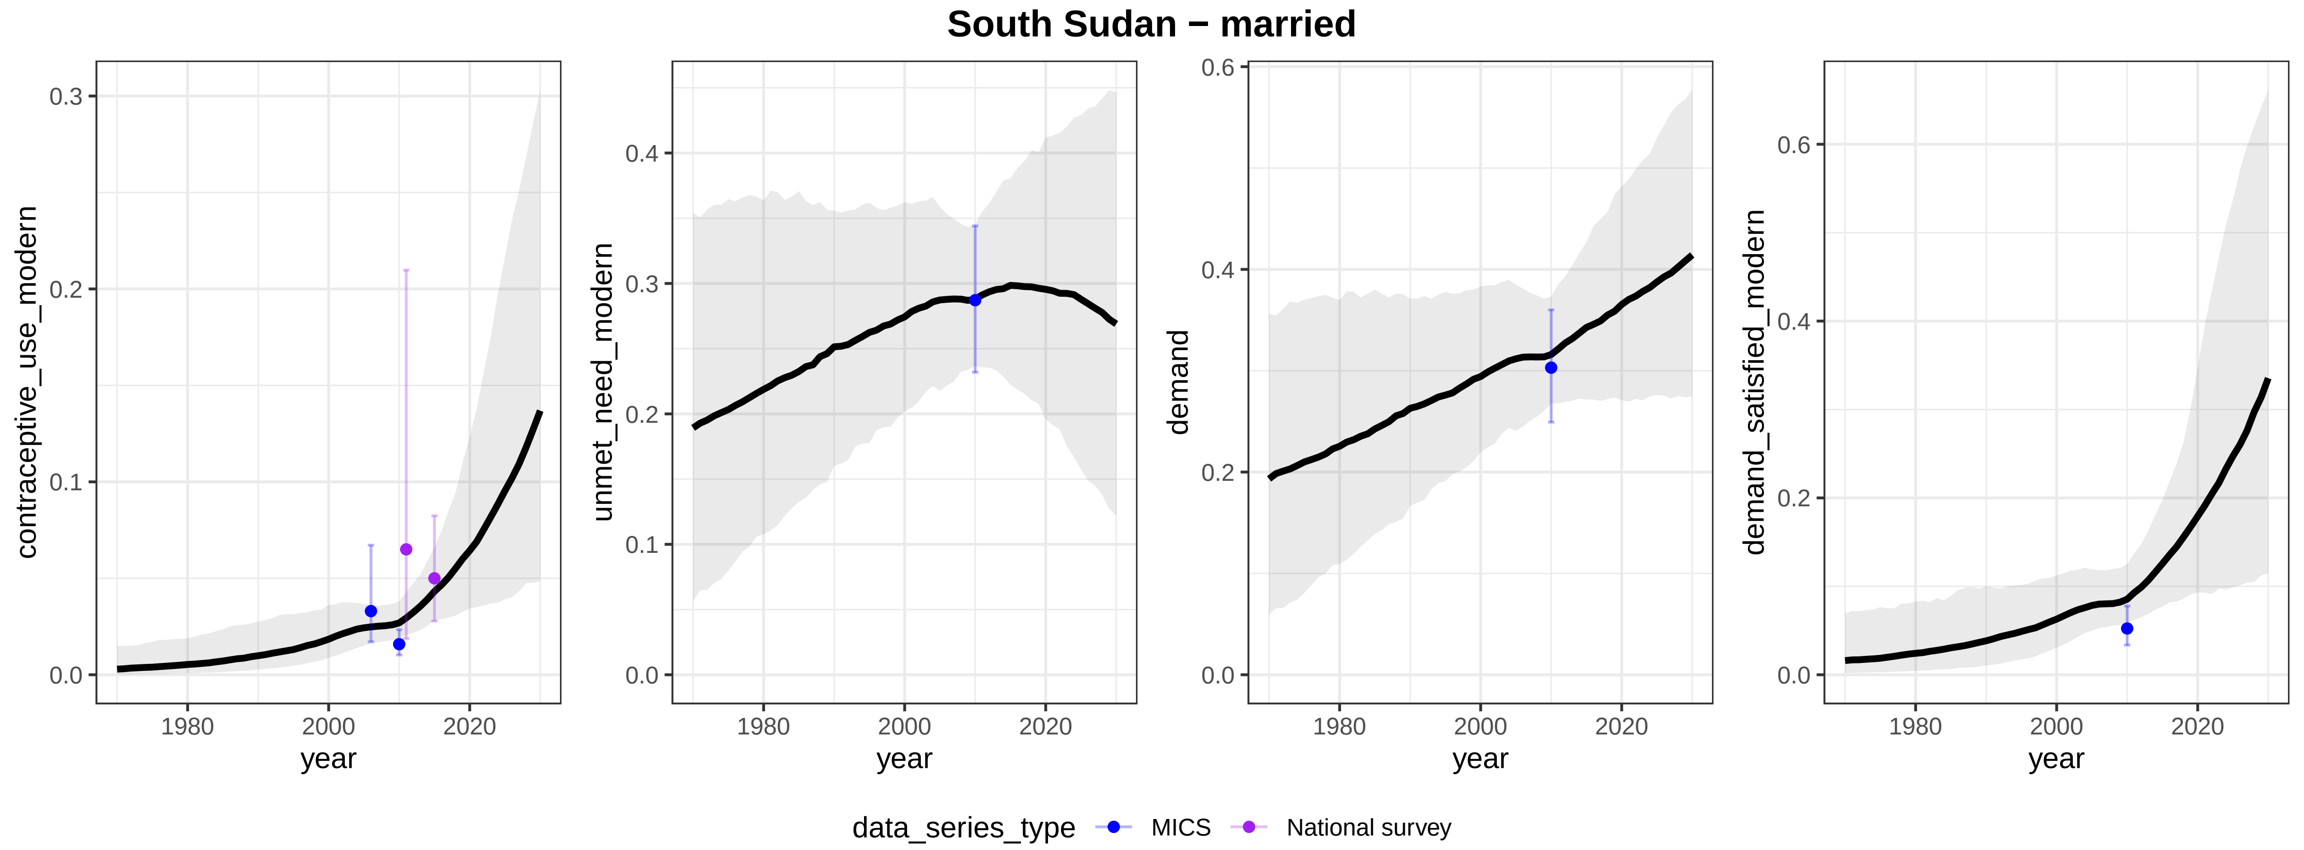
South Sudan − married
contraceptive_use_modern
unmet_need_modern
demand
demand_satisfied_modern
year
0.0
0.1
0.2
0.3
0.4
0.6
1980
2000
2020
data_series_type
MICS
National survey

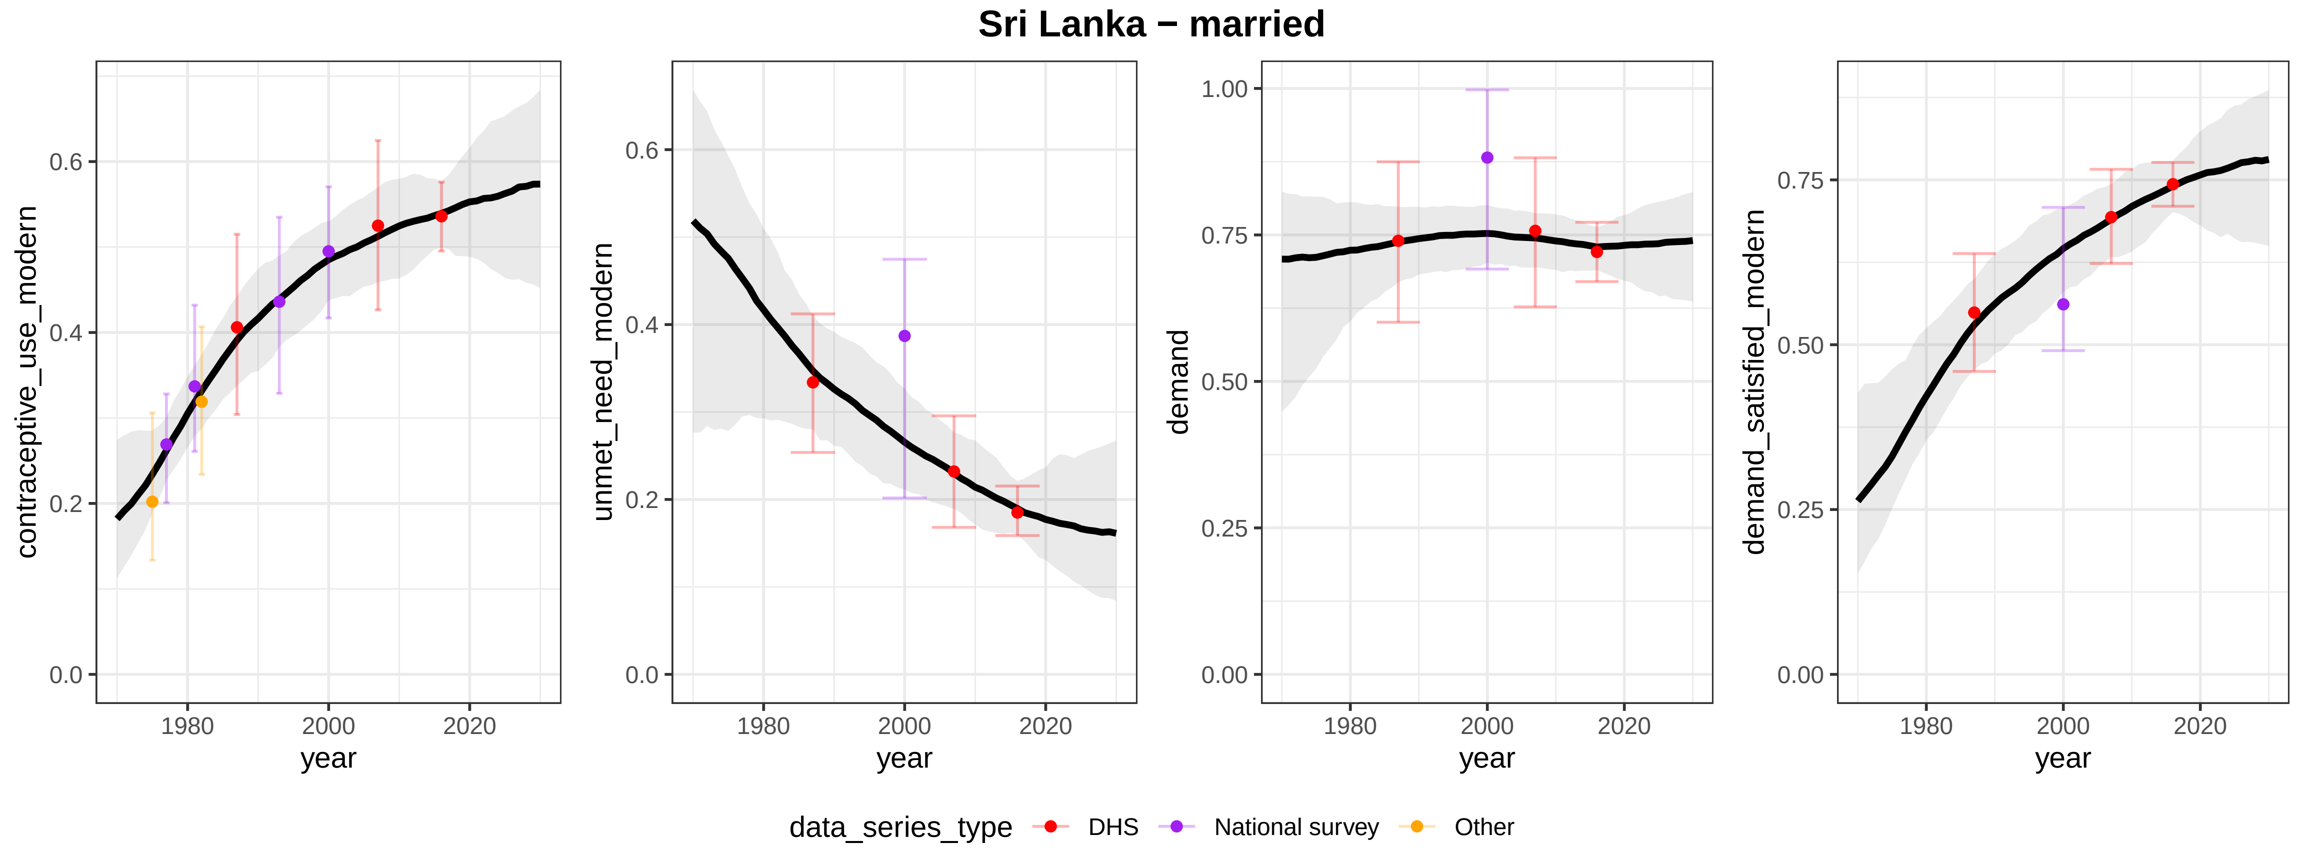

Sri Lanka − married
contraceptive_use_modern
unmet_need_modern
demand
demand_satisfied_modern
year
1980
2000
2020
0.0
0.2
0.4
0.6
0.00
0.25
0.50
0.75
1.00
data_series_type
DHS
National survey
Other

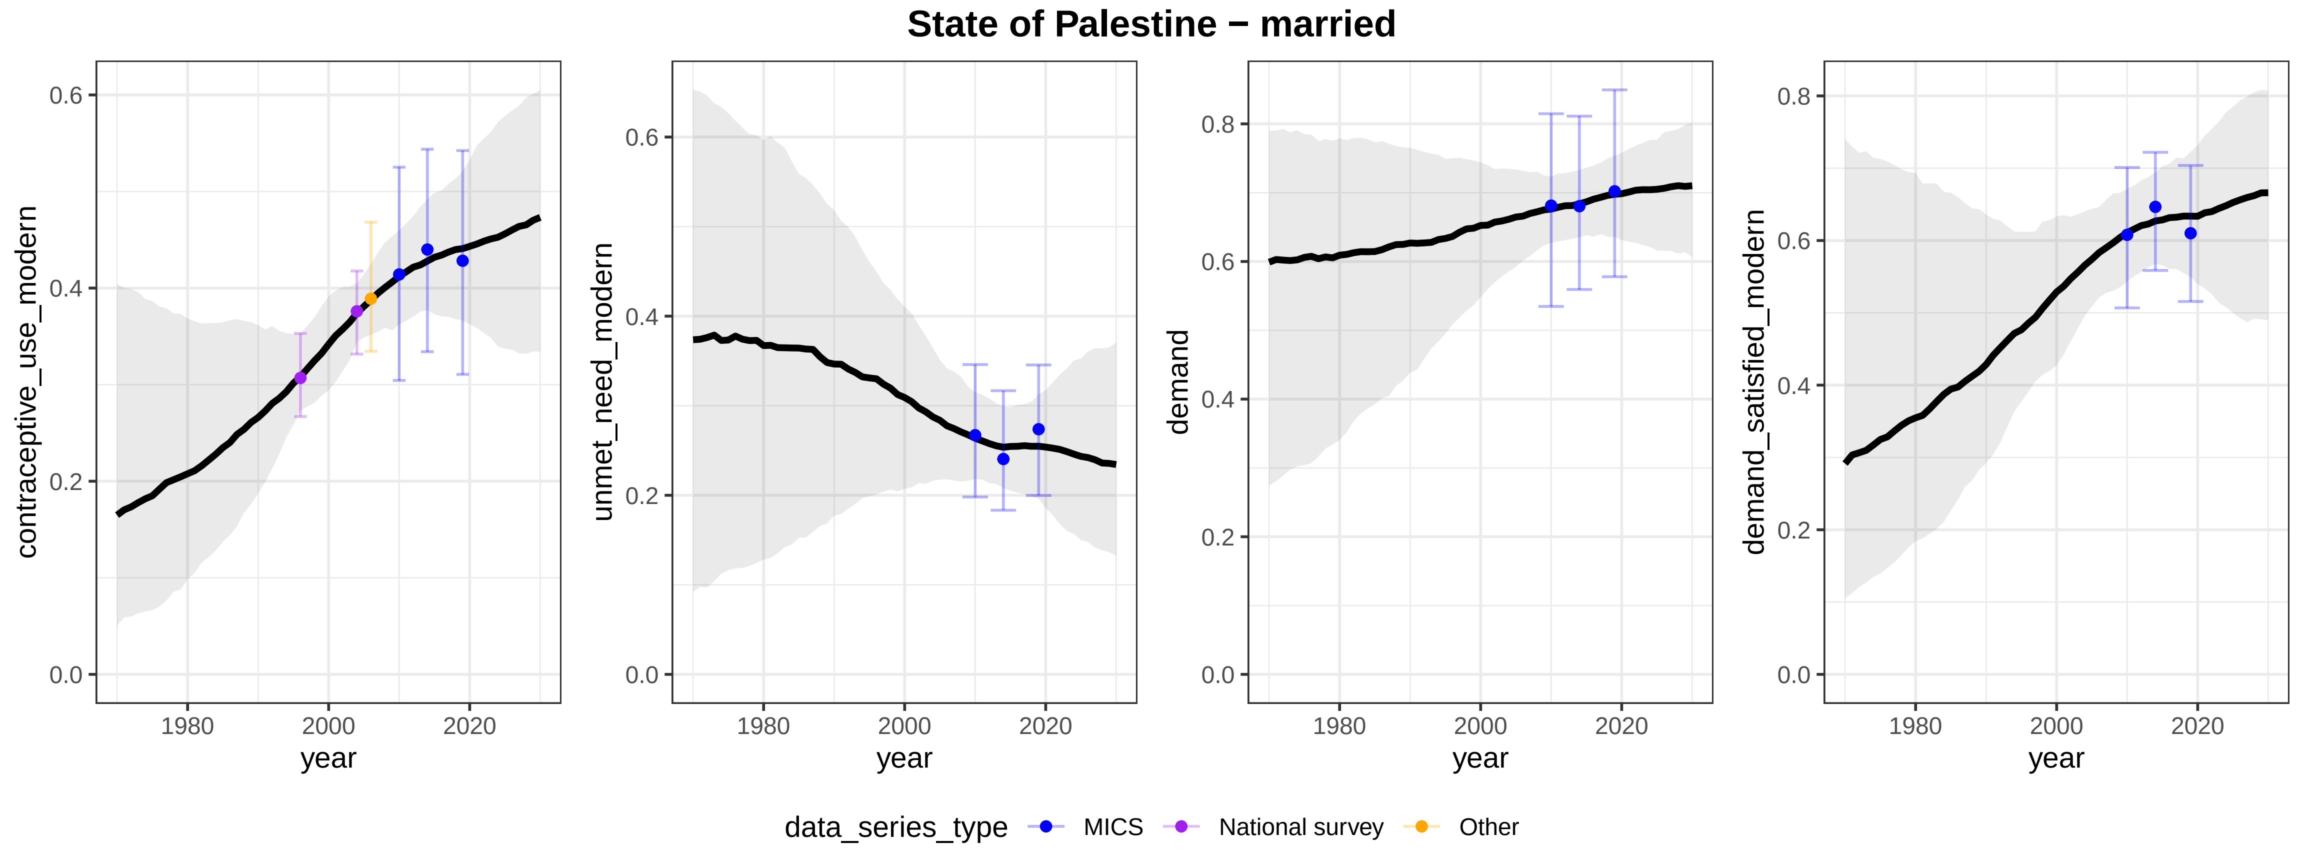
State of Palestine − married
contraceptive_use_modern
unmet_need_modern
demand
demand_satisfied_modern
0.0
0.2
0.4
0.6
0.8
1980
2000
2020
year
data_series_type
MICS
National survey
Other

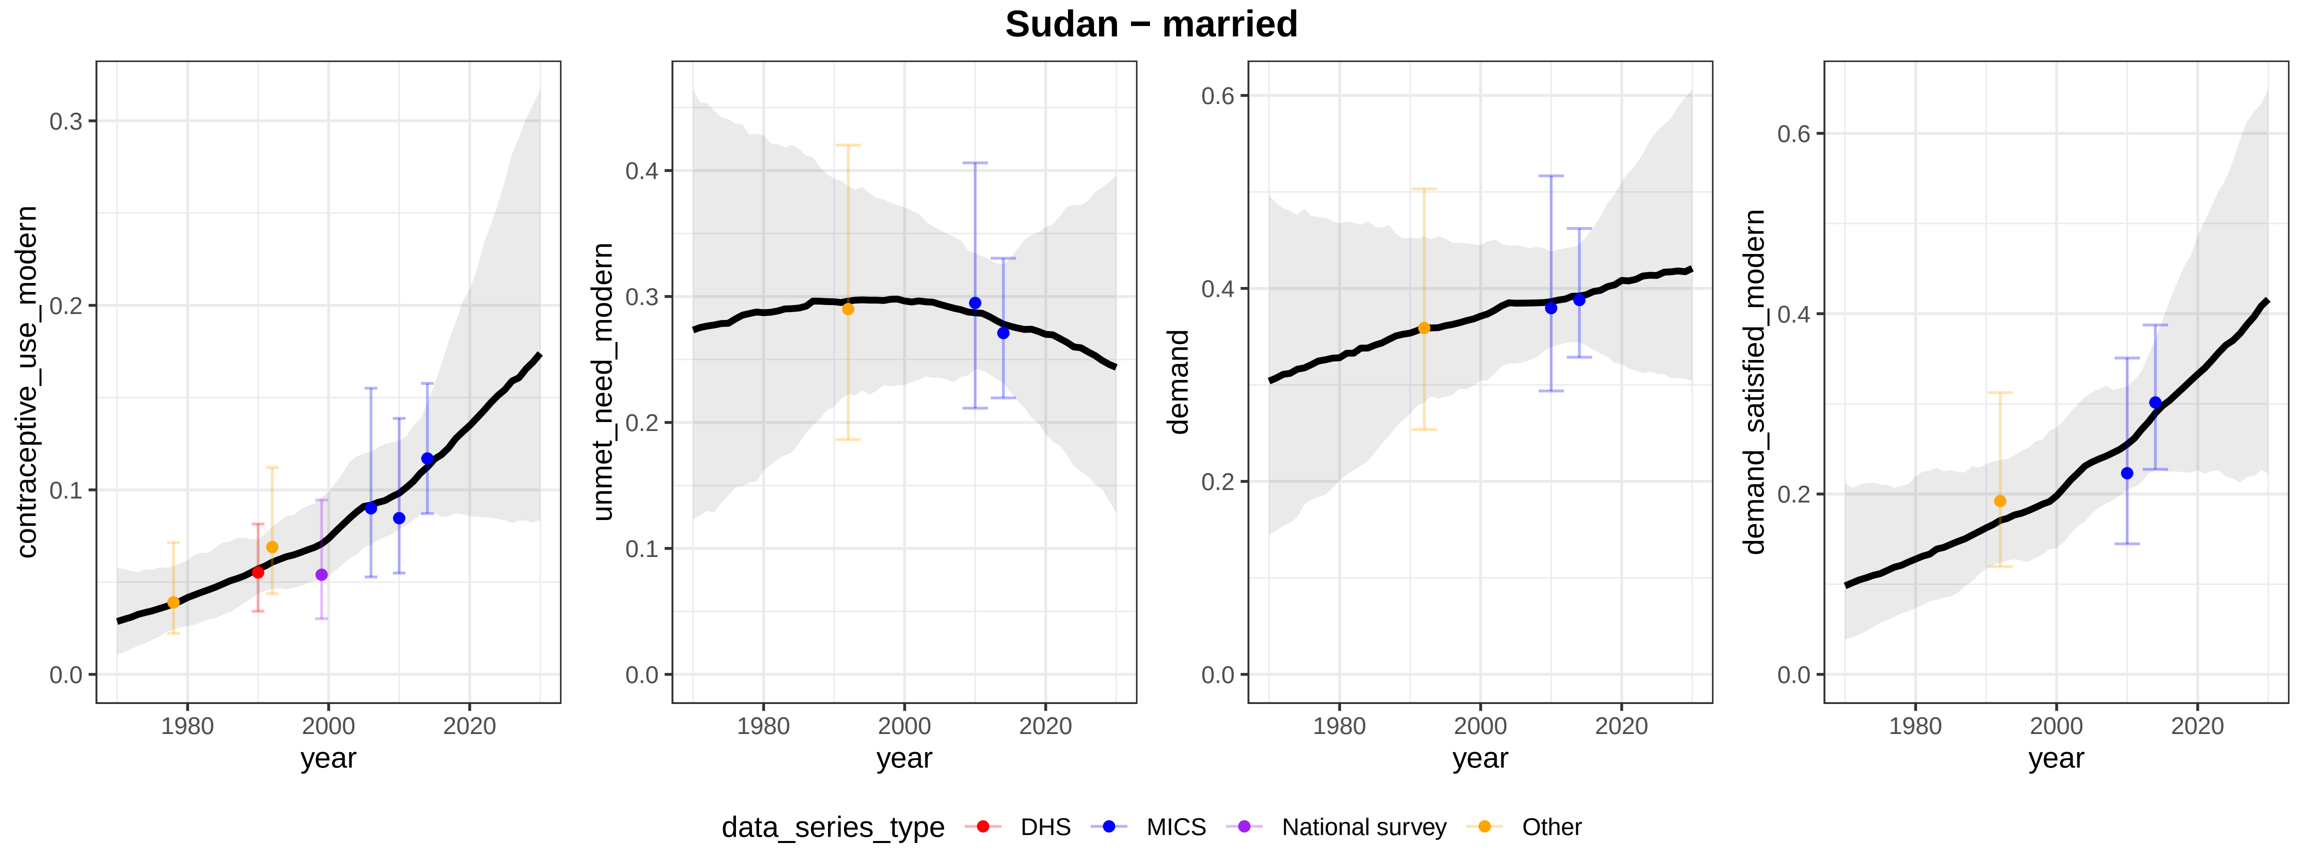
Sudan − married
contraceptive_use_modern
unmet_need_modern
demand
demand_satisfied_modern
year
0.0
0.1
0.2
0.3
0.4
0.6
1980
2000
2020
data_series_type
DHS
MICS
National survey
Other

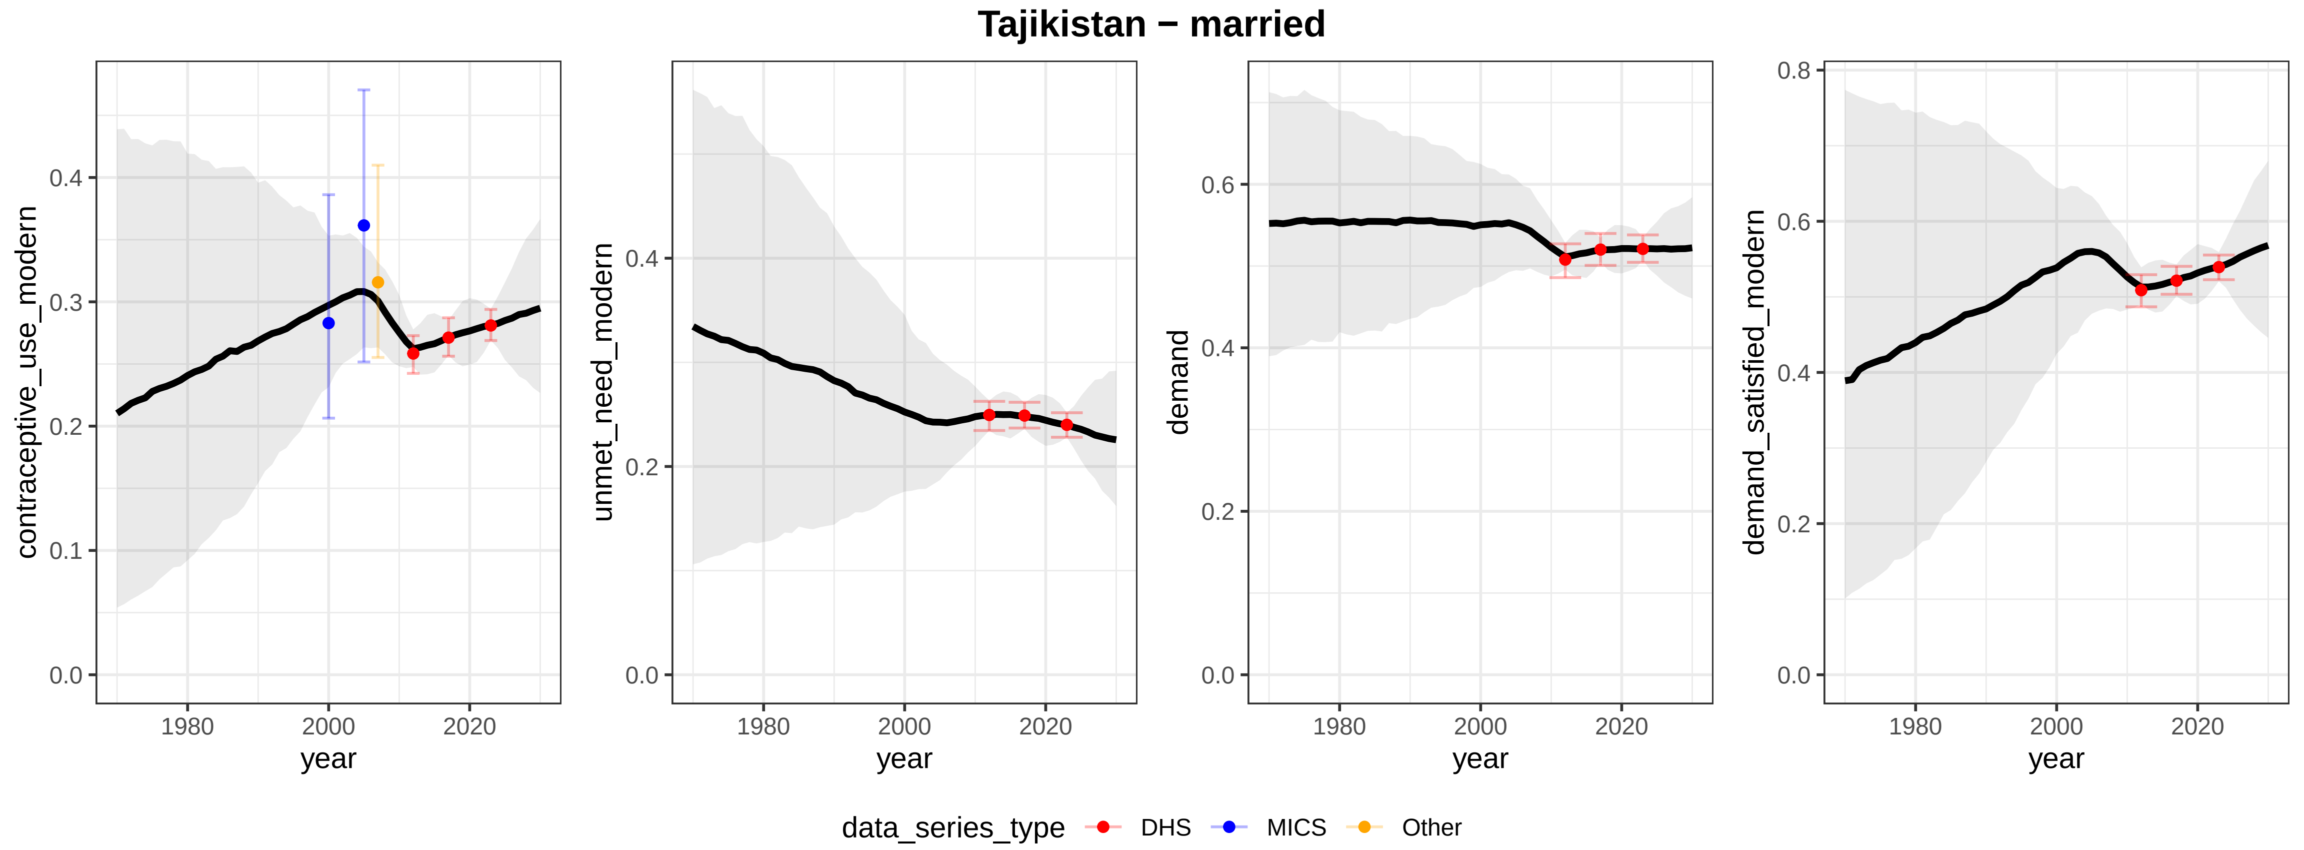

Tajikistan − married
contraceptive_use_modern
unmet_need_modern
demand
demand_satisfied_modern
year
1980
2000
2020
0.0
0.1
0.2
0.3
0.4
0.6
0.8
data_series_type
DHS
MICS
Other

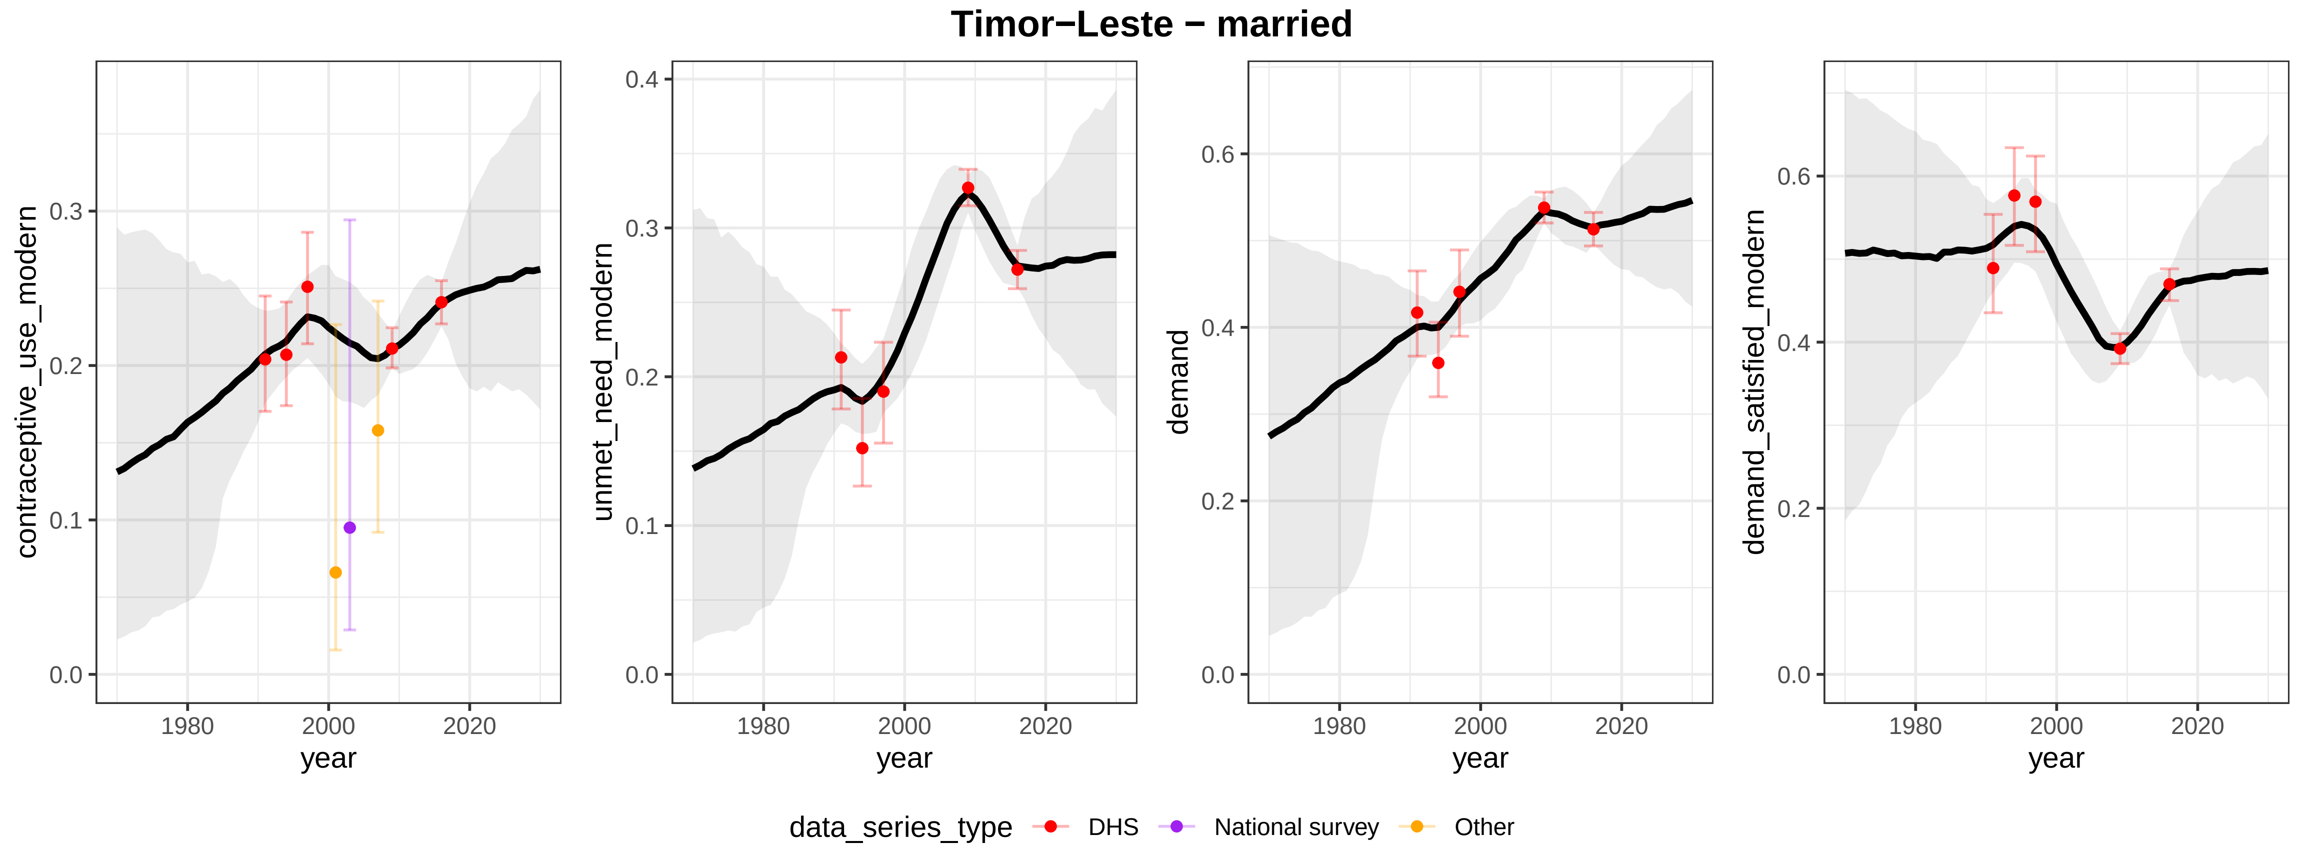
Timor−Leste − married
contraceptive_use_modern
unmet_need_modern
demand
demand_satisfied_modern
year
1980
2000
2020
0.0
0.1
0.2
0.3
0.4
0.6
data_series_type
DHS
National survey
Other

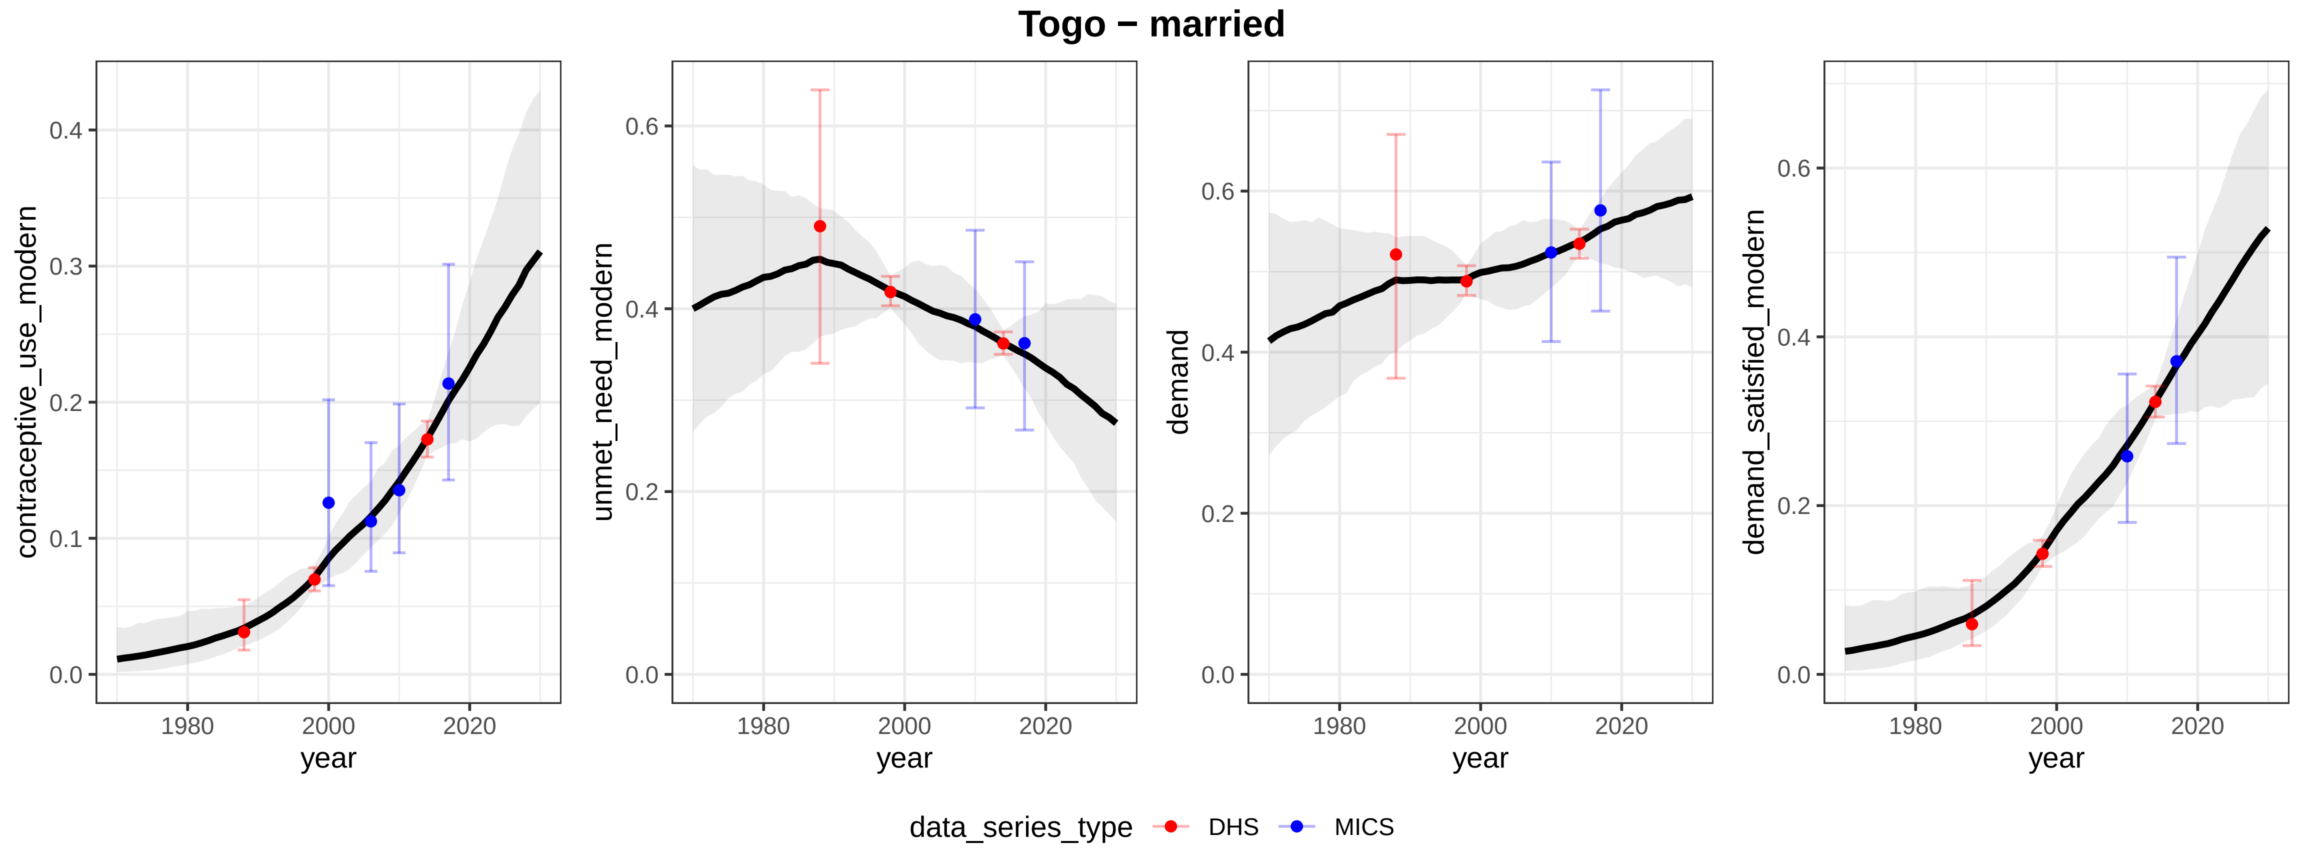

Togo − married
contraceptive_use_modern
unmet_need_modern
demand
demand_satisfied_modern
year
data_series_type
DHS
MICS

# Uganda − married

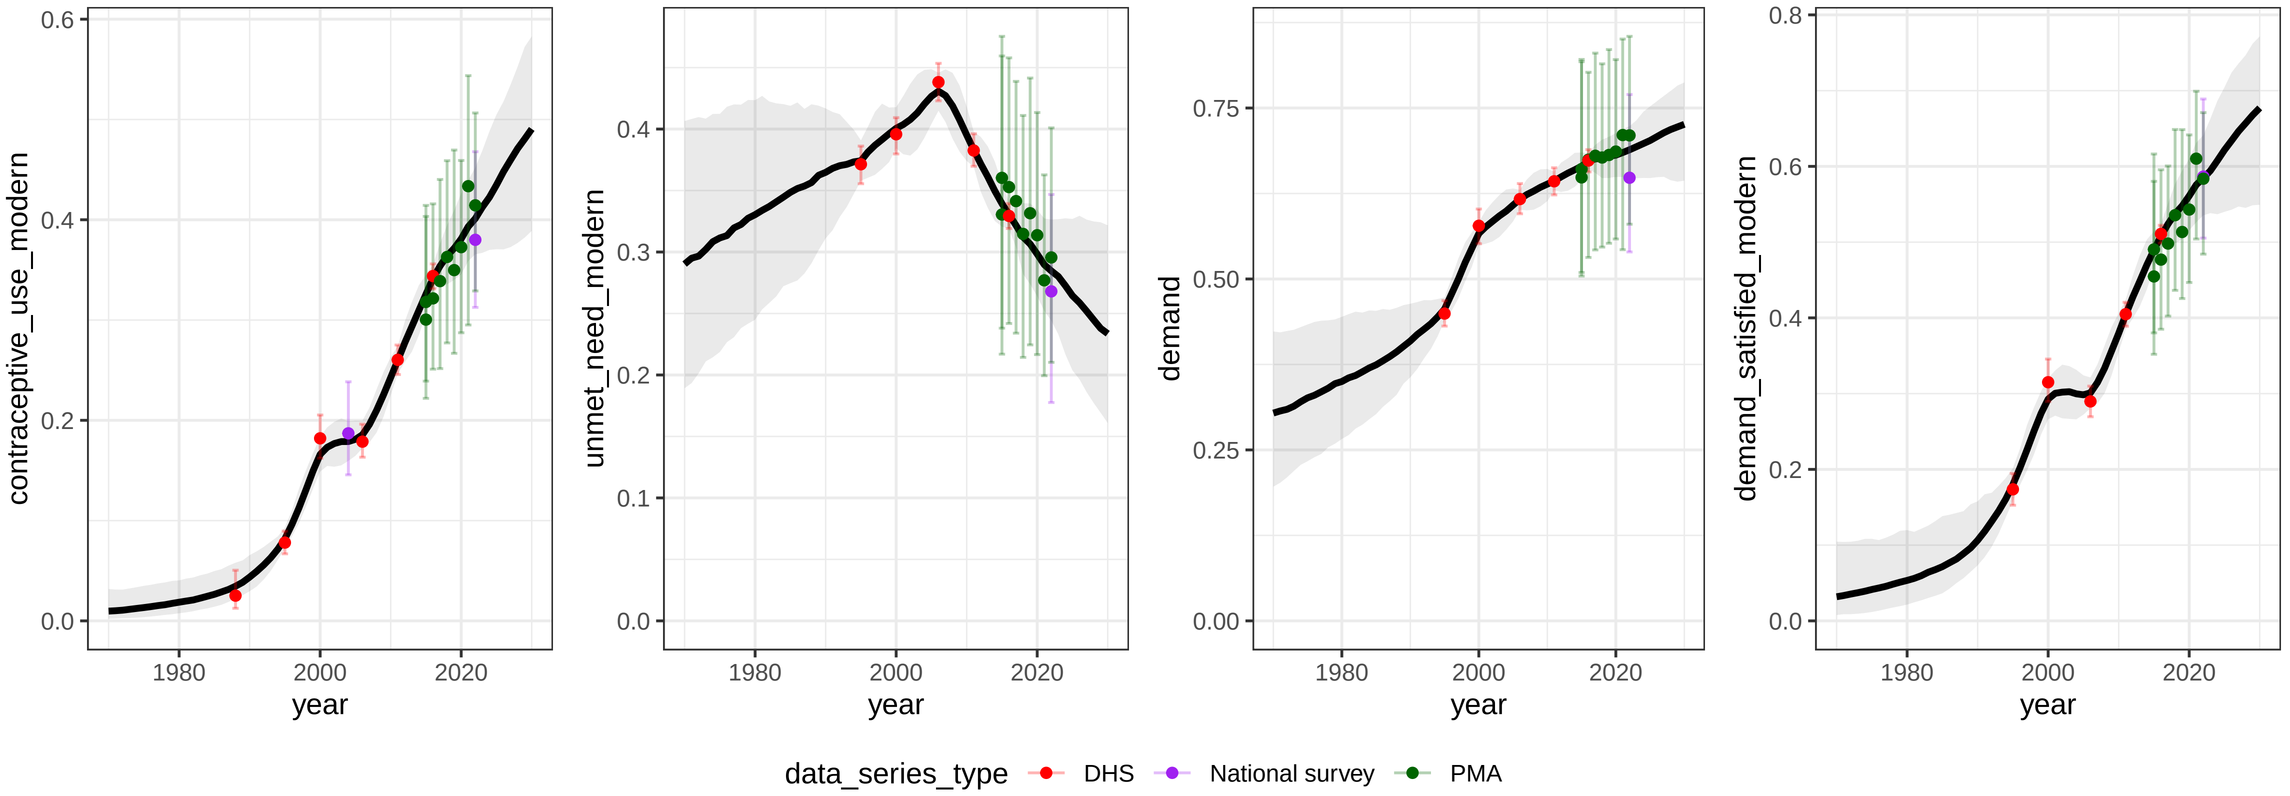

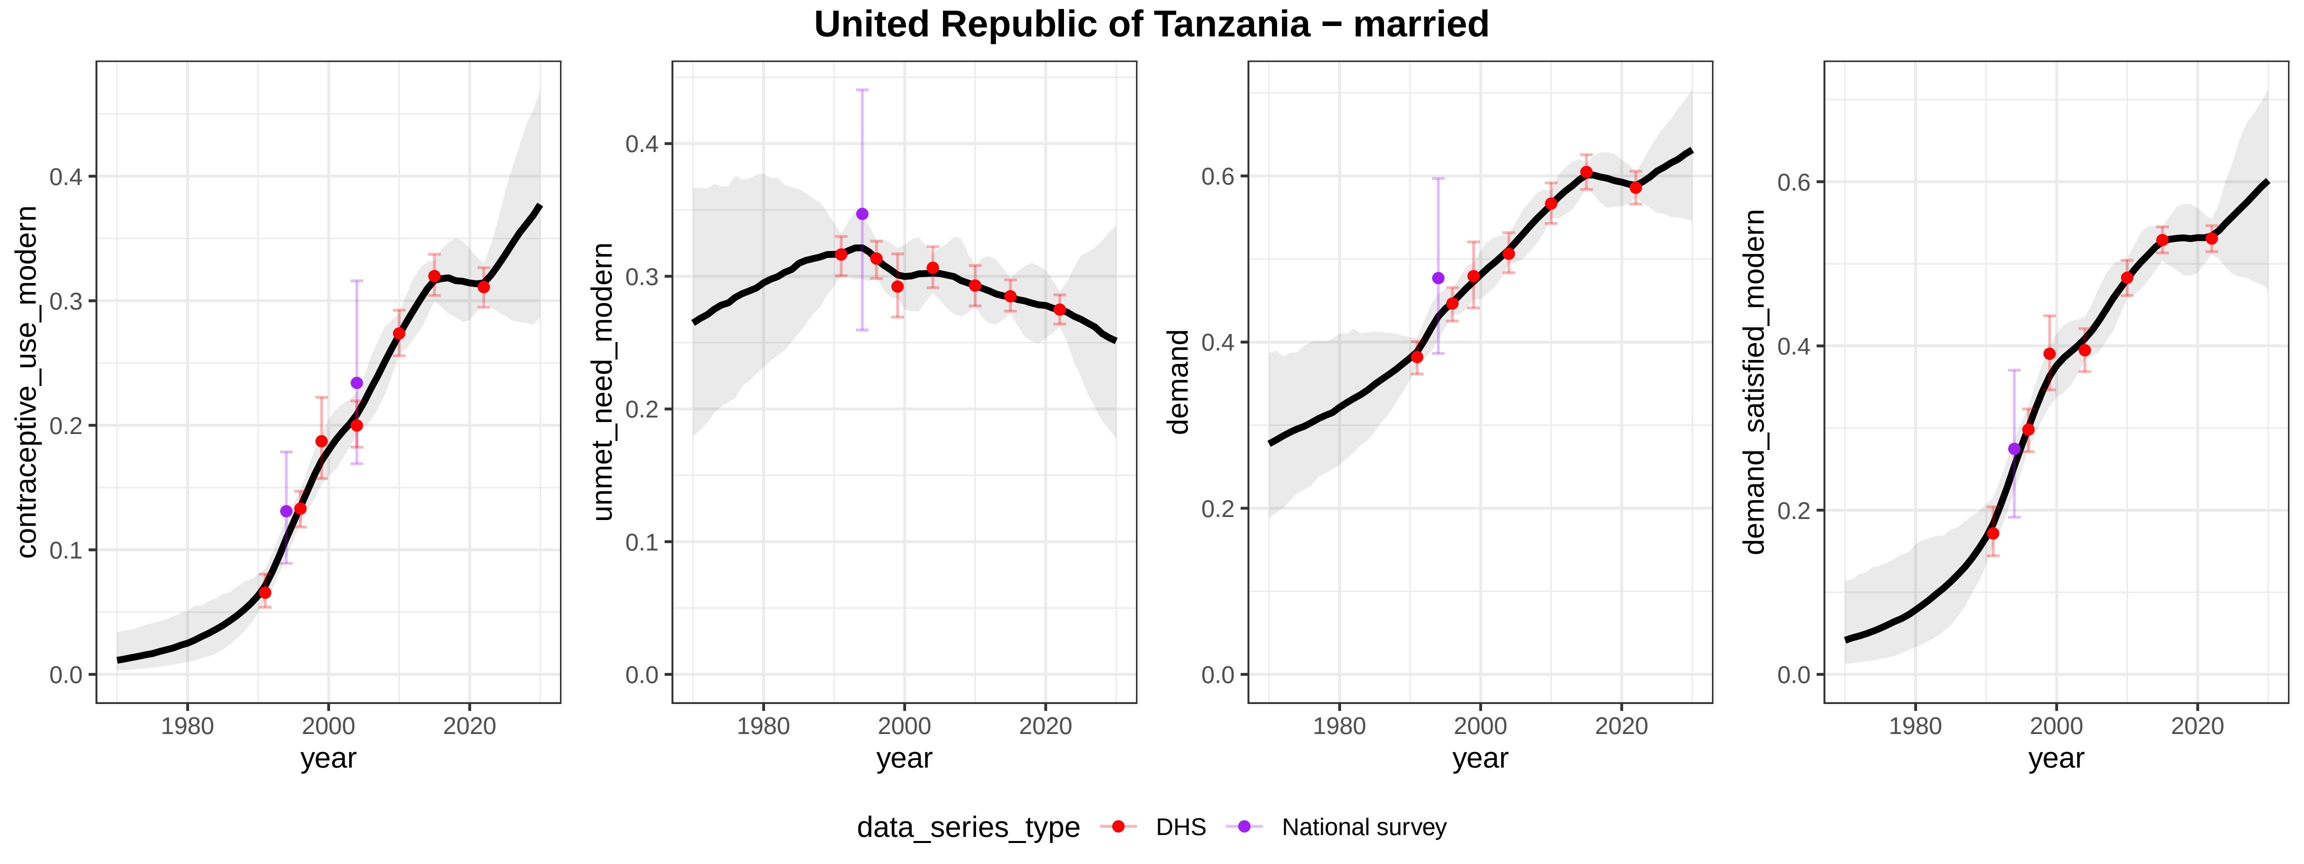

United Republic of Tanzania − married
contraceptive_use_modern
unmet_need_modern
demand
demand_satisfied_modern
year
0.0
0.1
0.2
0.3
0.4
0.6
1980
2000
2020
data_series_type
DHS
National survey

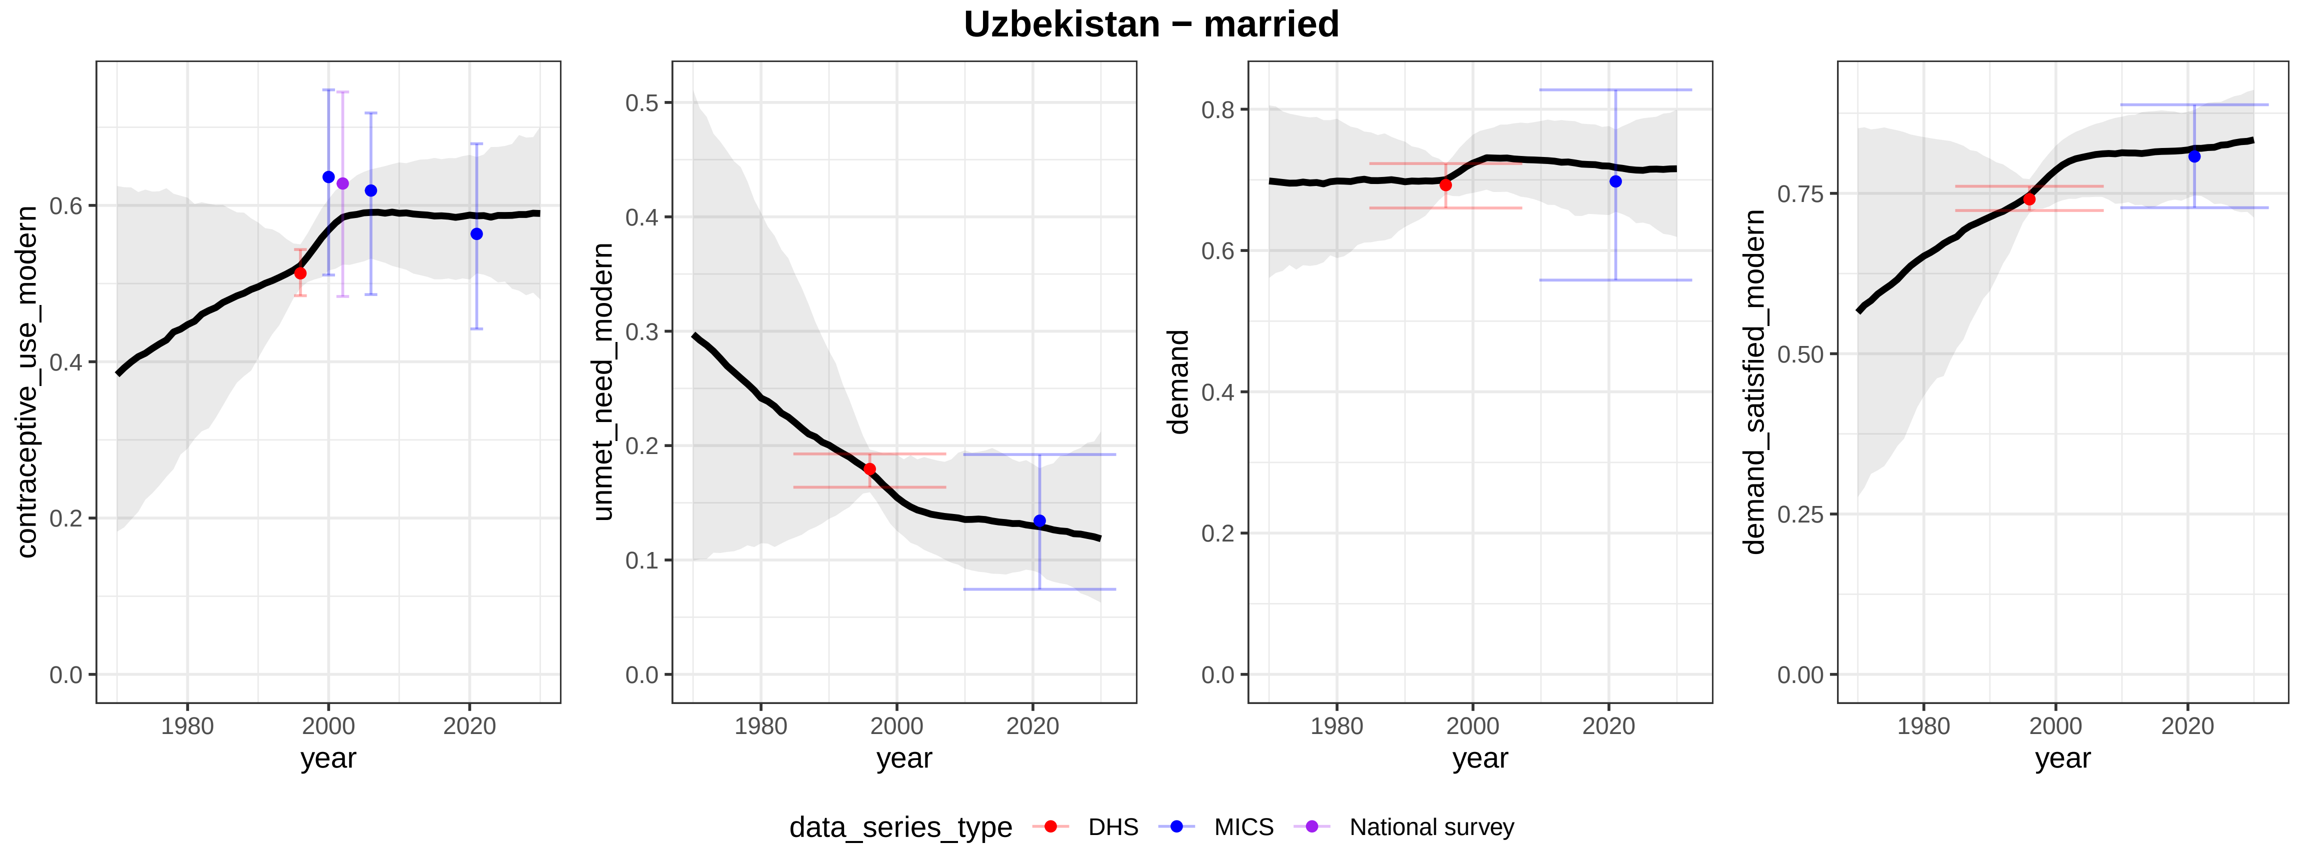
Uzbekistan − married
contraceptive_use_modern
unmet_need_modern
demand
demand_satisfied_modern
year
data_series_type
DHS
MICS
National survey

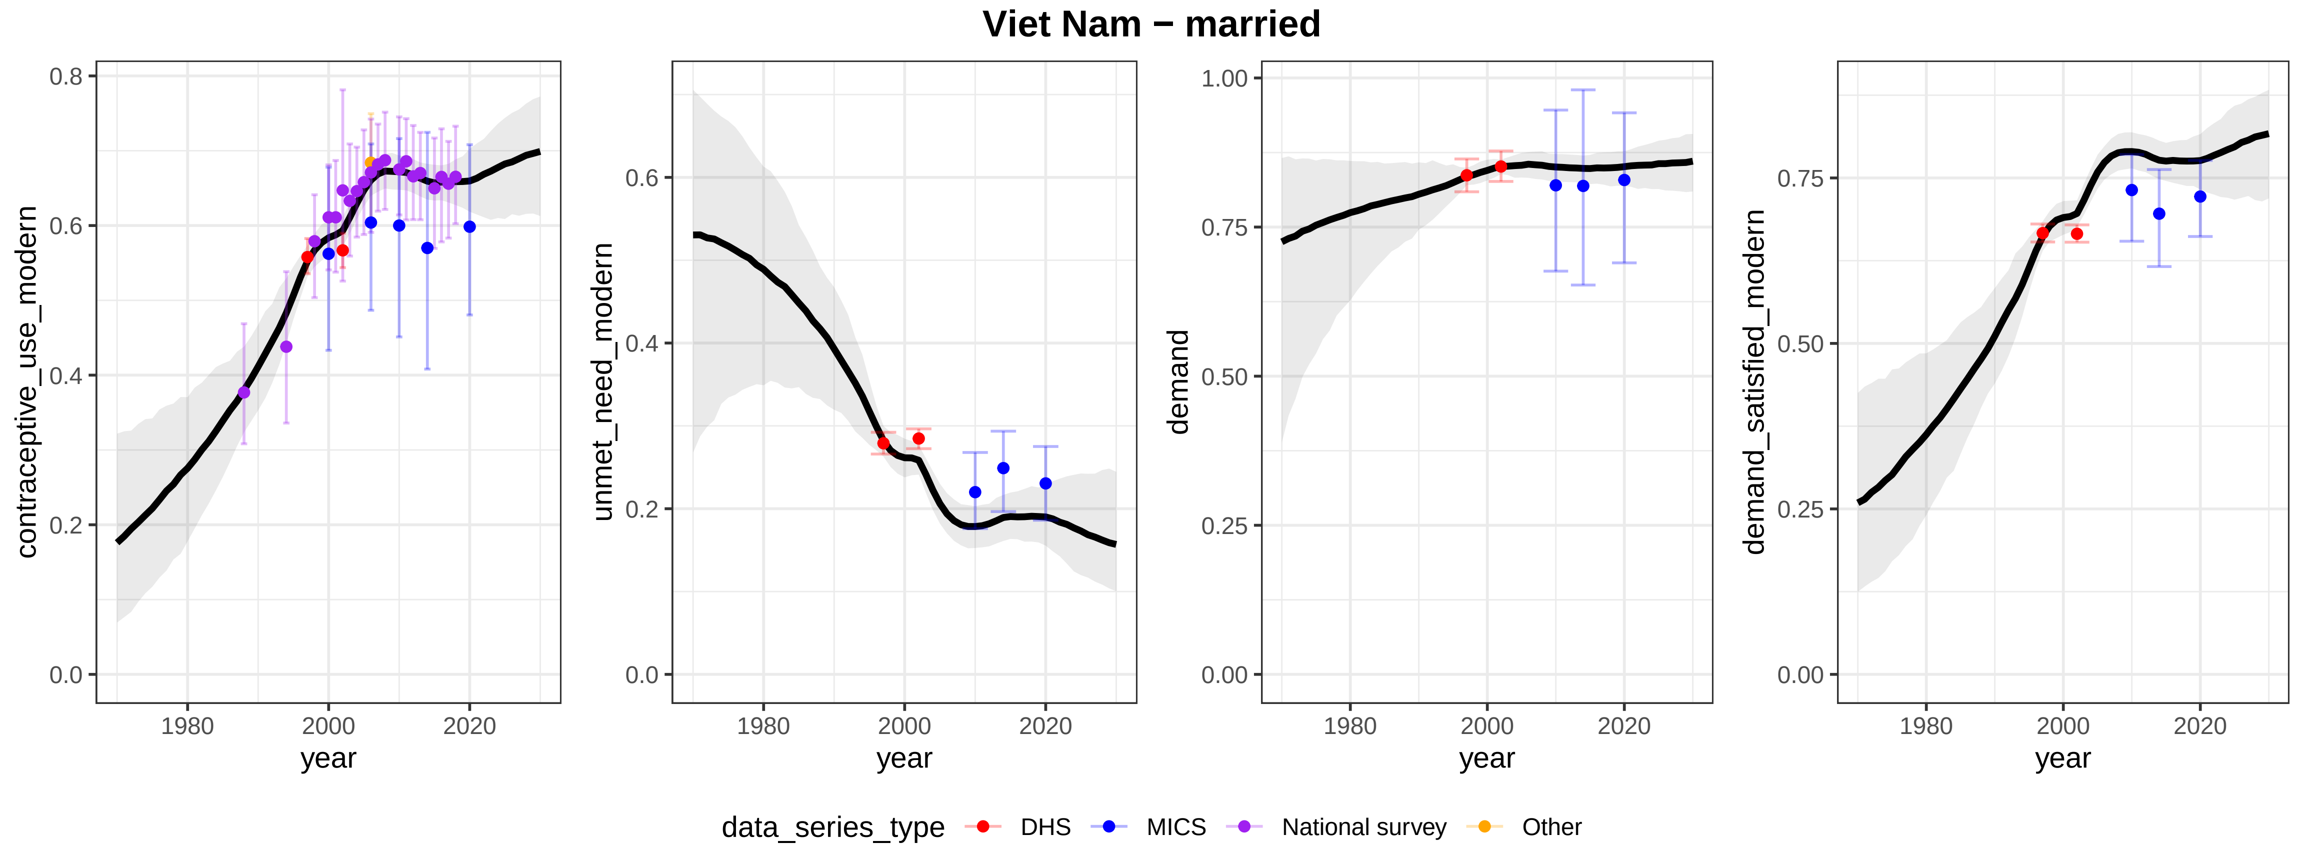

Viet Nam − married
contraceptive_use_modern
unmet_need_modern
demand
demand_satisfied_modern
year
1980
2000
2020
0.0
0.2
0.4
0.6
0.8
0.00
0.25
0.50
0.75
1.00
data_series_type
DHS
MICS
National survey
Other

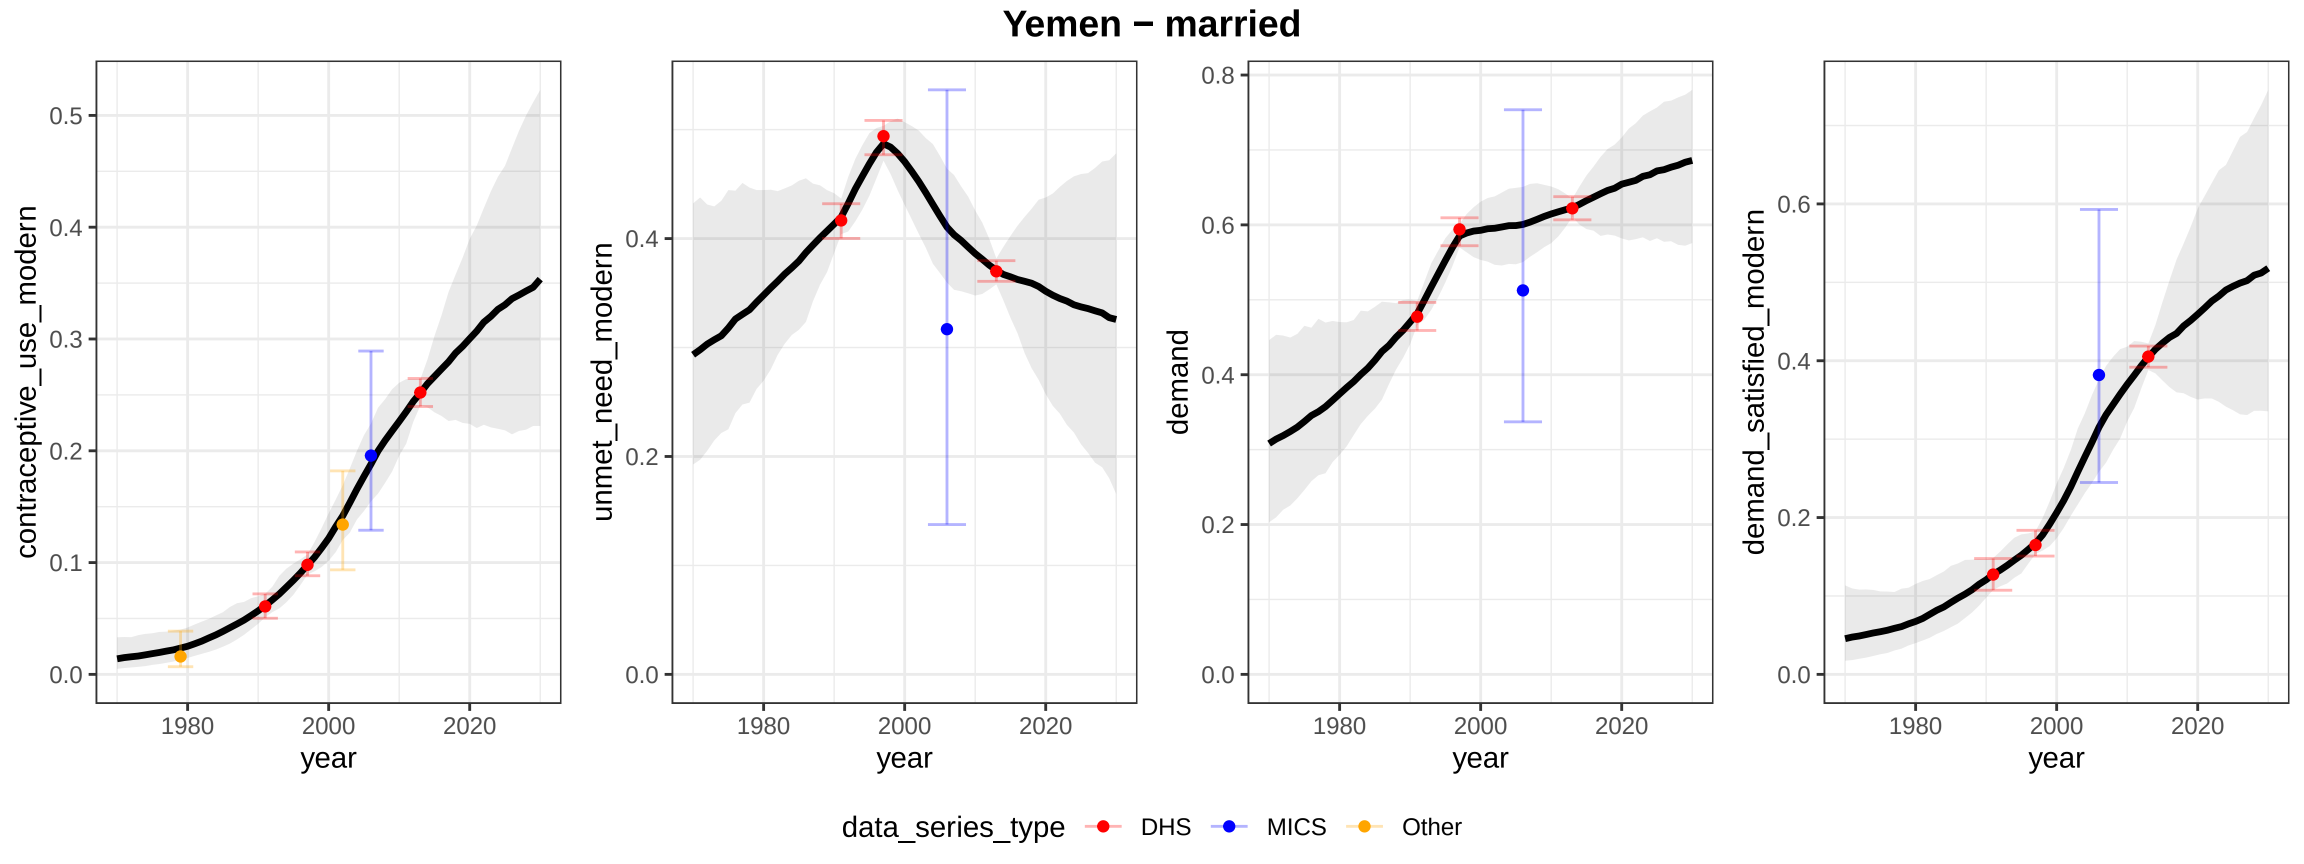
Yemen − married
contraceptive_use_modern
unmet_need_modern
demand
demand_satisfied_modern
0.0
0.1
0.2
0.3
0.4
0.5
0.6
0.8
year
1980
2000
2020
data_series_type
DHS
MICS
Other

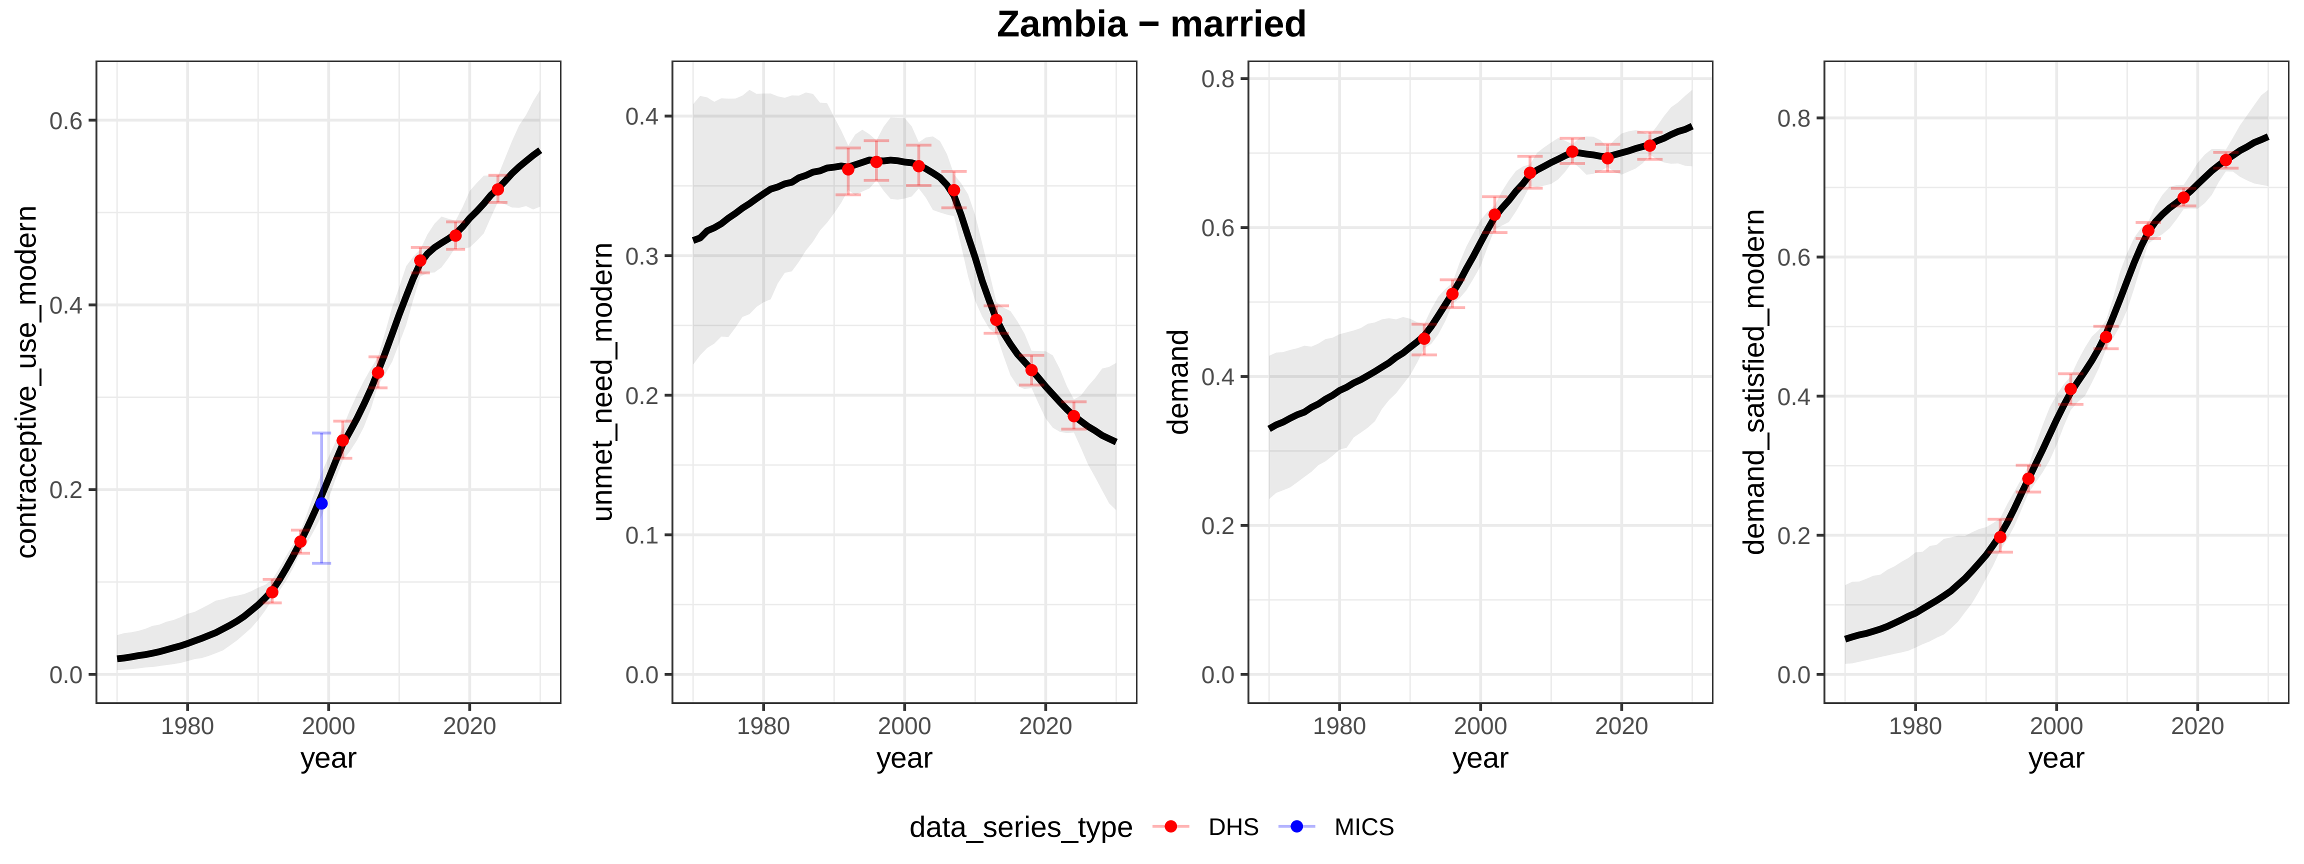

Zambia − married
contraceptive_use_modern
unmet_need_modern
demand
demand_satisfied_modern
year
0.0
0.2
0.4
0.6
0.8
0.1
0.3
1980
2000
2020
data_series_type
DHS
MICS

# Zimbabwe − married

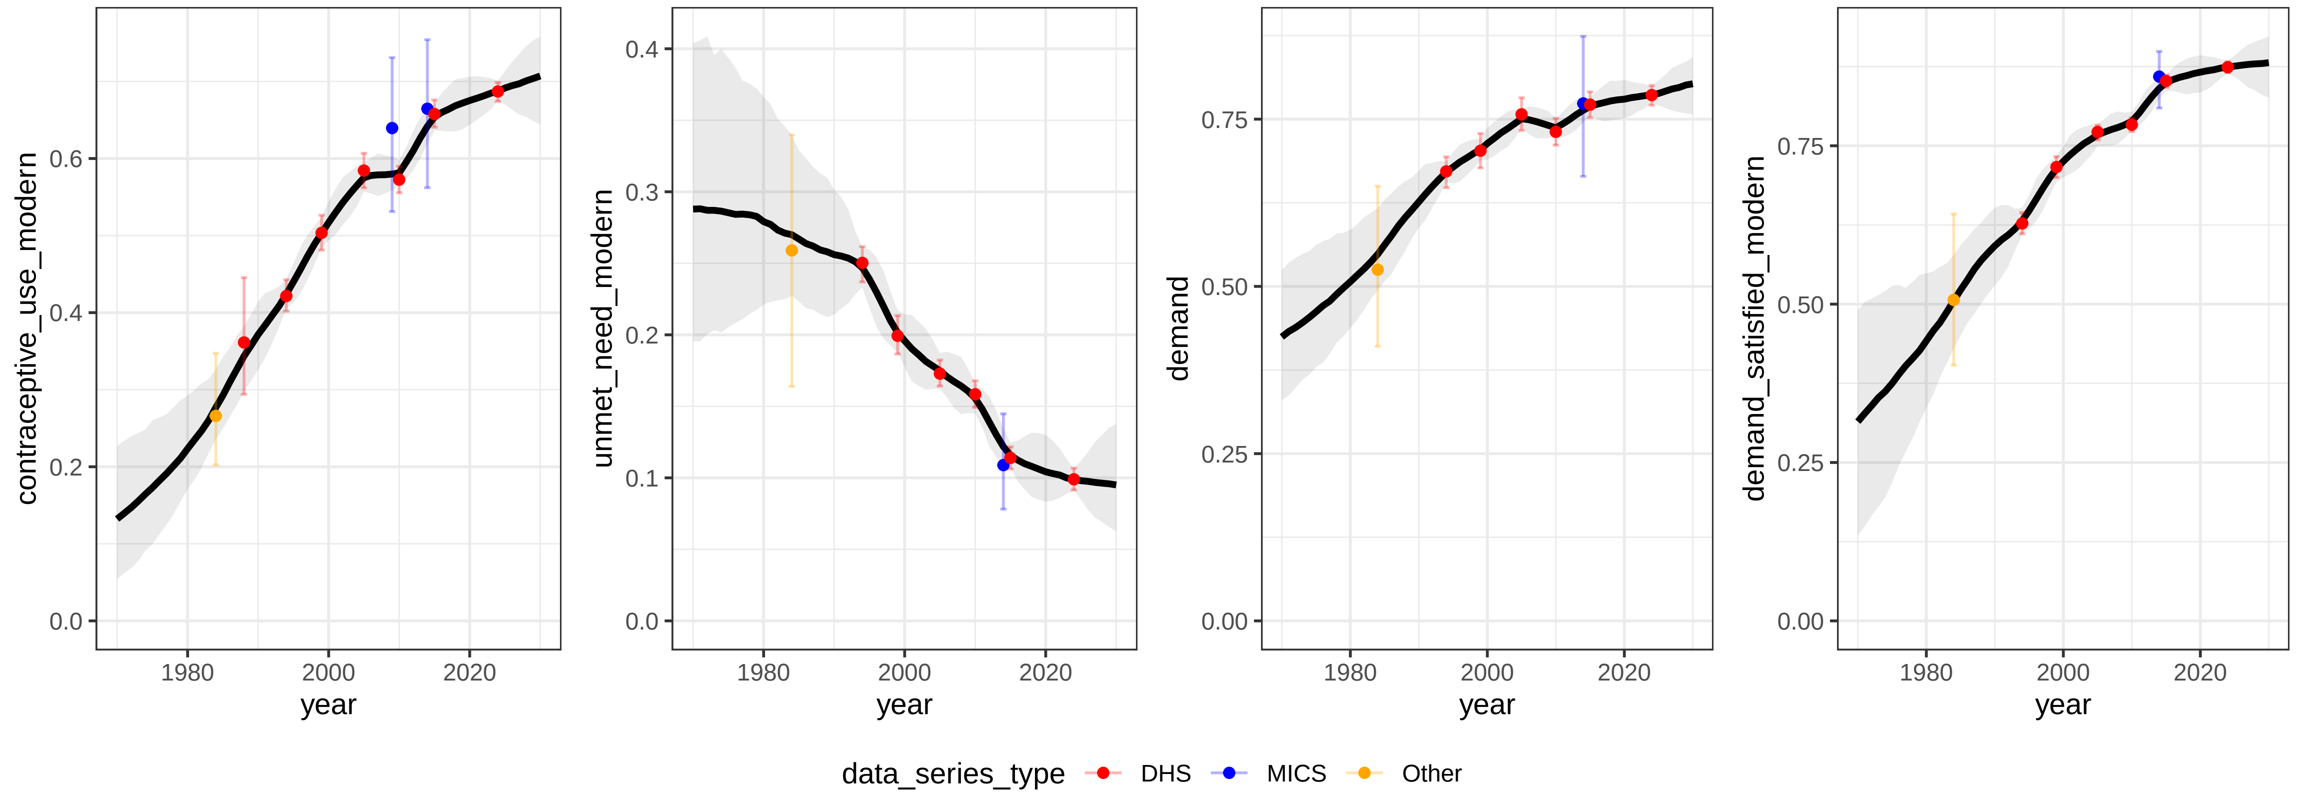

Supplement: Supplementary file 1 [file suppl_allmarried.pdf]
